# Supplementary material for: Unsupervised Domain Adaptation in Semantic Segmentation via Orthogonal and Clustered Embeddings
Source: arXiv:2011.12616 source file (2020-11-25)
Supplement: Supplementary file 1 [file supplementary.tex]

\vspace{-0.5cm}

\section{Qualitative Results}

In Figure~\ref{fig:qual_res} we show some additional qualitative results of the proposed model when adapting source knowledge either from the GTA5 or the SYNTHIA datasets to the Cityscapes one. In these figures we can appreciate a robust improvement with respect to the baselines: e.g., the person in row 1, the sidewalk in row 2, the traffic sign in row 3, the road in rows 4, 5, 7 and 8. Additionally, shapes and details are more refined and localized.
\newcommand{\imgsize}{27.58mm}
\begin{figure*}[h!]
\centering
\begin{subfigure}[htbp]{\textwidth}

%\hspace{0.22cm}
\centering
\resizebox{\textwidth}{!}{%
\hspace{0.6cm}
\begin{tabular}{cccccccccc}
\cellcolor[HTML]{804080}{\color[HTML]{FFFFFF} \textbf{road}} & \cellcolor[HTML]{F423E8}\textbf{sidewalk} & \cellcolor[HTML]{464646}{\color[HTML]{FFFFFF} \textbf{building}} & \cellcolor[HTML]{66669C}{\color[HTML]{FFFFFF} \textbf{wall}} & \cellcolor[HTML]{BE9999}\textbf{fence} & \cellcolor[HTML]{999999}\textbf{pole} & \cellcolor[HTML]{FAAA1E}\textbf{traffic light} & \cellcolor[HTML]{DCDC00}\textbf{traffic sign} &\cellcolor[HTML]{6B8E23} \textbf{vegetation} & \cellcolor[HTML]{98FB98}\textbf{terrain} \\ %\cline{10-10} 
\cellcolor[HTML]{4682B4}\textbf{sky} & \cellcolor[HTML]{DC143C}{\color[HTML]{FFFFFF} \textbf{person}} & \cellcolor[HTML]{FF0000}{\color[HTML]{FFFFFF} \textbf{rider}} & \cellcolor[HTML]{00008E}{\color[HTML]{FFFFFF} \textbf{car}} & \cellcolor[HTML]{000046}{\color[HTML]{FFFFFF} \textbf{truck}} & \cellcolor[HTML]{003C64}{\color[HTML]{FFFFFF} \textbf{bus}} & \cellcolor[HTML]{005064}{\color[HTML]{FFFFFF} \textbf{train}} & \cellcolor[HTML]{0000E6}{\color[HTML]{FFFFFF} \textbf{motorcycle}} & \cellcolor[HTML]{770B20}{\color[HTML]{FFFFFF} \textbf{bicycle}} & \cellcolor[HTML]{000000}{\color[HTML]{FFFFFF} \textbf{unlabeled}} \\ 
%& \multicolumn{1}{c|}{\cellcolor[HTML]{770B20}{\color[HTML]{FFFFFF} \textbf{bicycle}}} & \multicolumn{1}{c|}{\textbf{unlabeled}} \\ \cline{10-10} 
\end{tabular}%
}

\vspace{0.1cm}
\end{subfigure}
\setlength{\tabcolsep}{0.7pt} % Default value: 6pt

\centering
\begin{subfigure}[htbp]{2\textwidth}
\begin{tabular}{c @{\hspace{1mm}} | @{\hspace{1.5mm}} cccccc}
  
   \multirow{8}{*}{\rotatebox{90}{GTA5 $\rightarrow$ Cityscapes}} &
   \includegraphics[width=\imgsize]{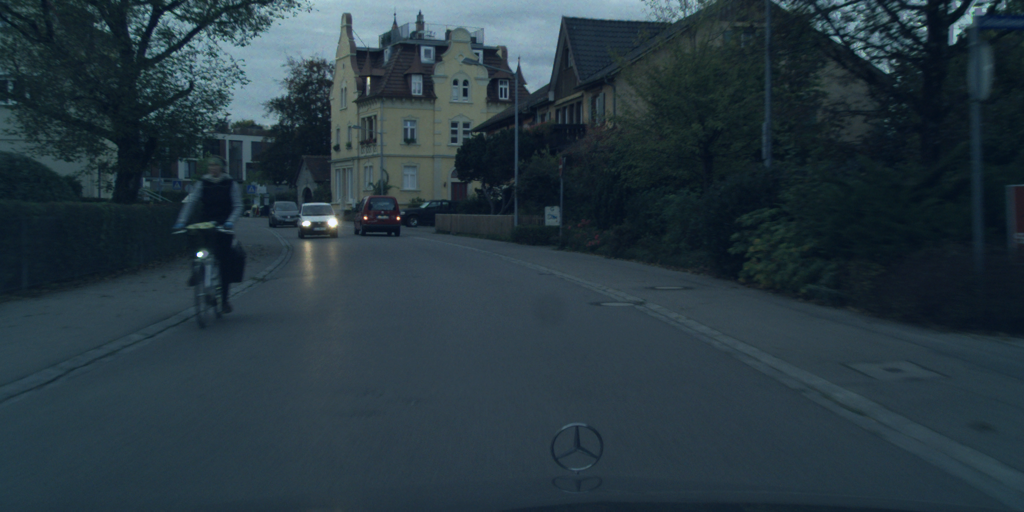} &
   \includegraphics[width=\imgsize]{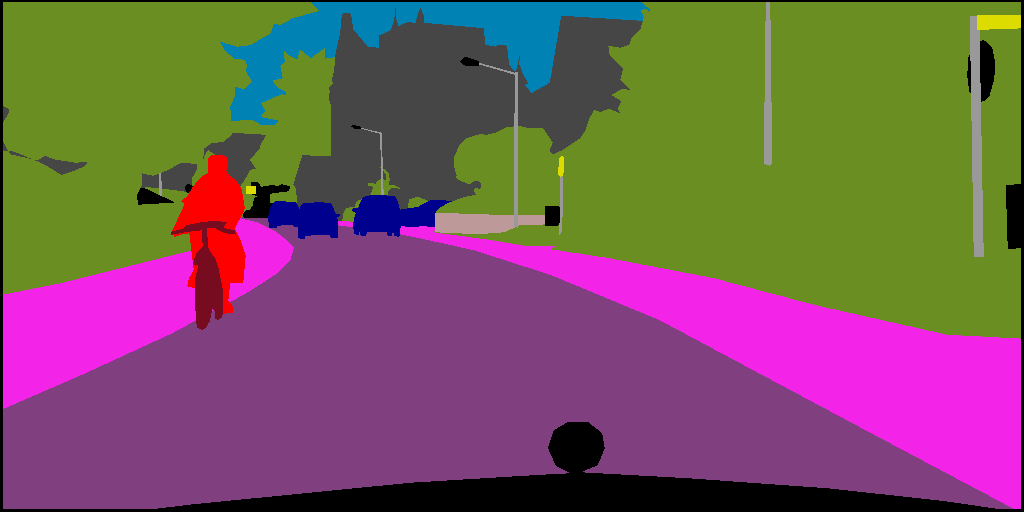} & 
   \includegraphics[width=\imgsize]{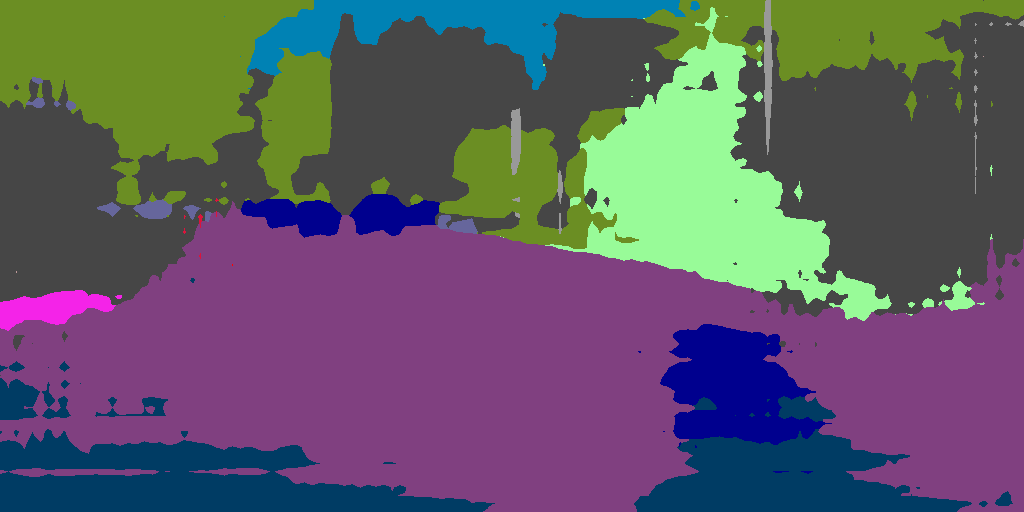} & 
   \includegraphics[width=\imgsize]{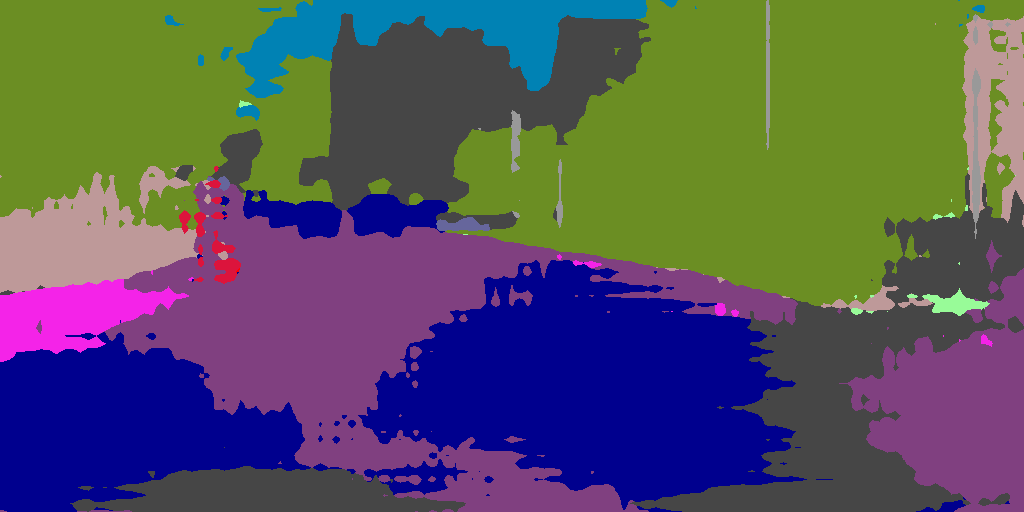} & 
   \includegraphics[width=\imgsize]{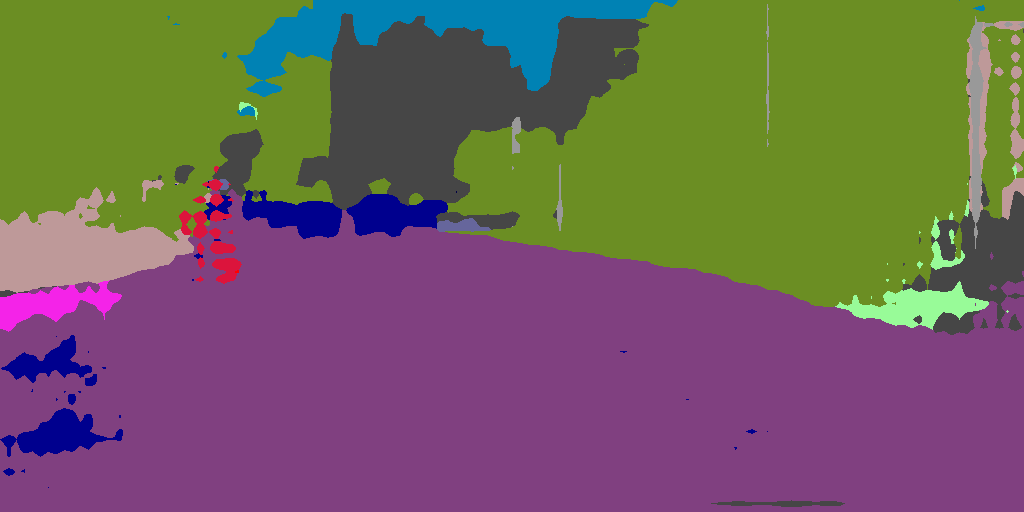} &
   \includegraphics[width=\imgsize]{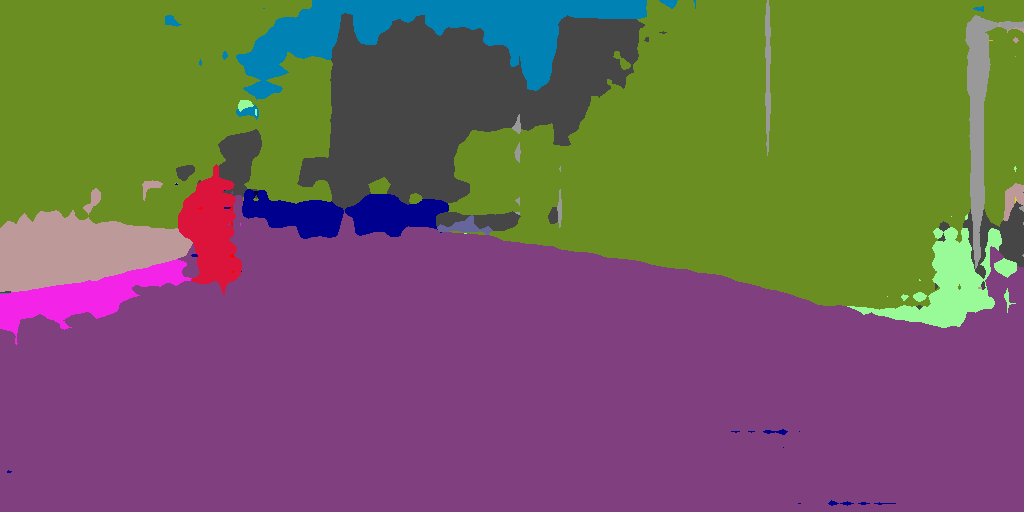} \\ 
   
   &
   \includegraphics[width=\imgsize]{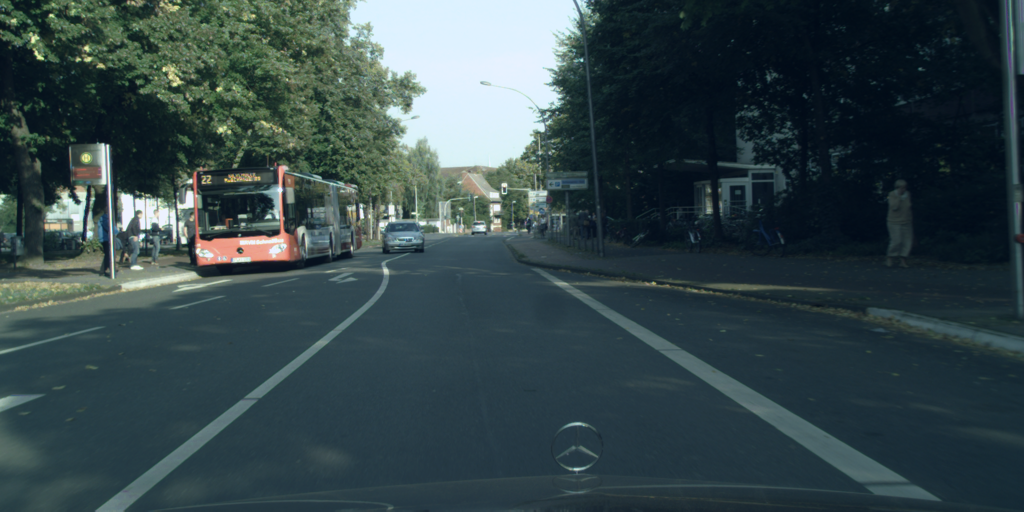} &
   \includegraphics[width=\imgsize]{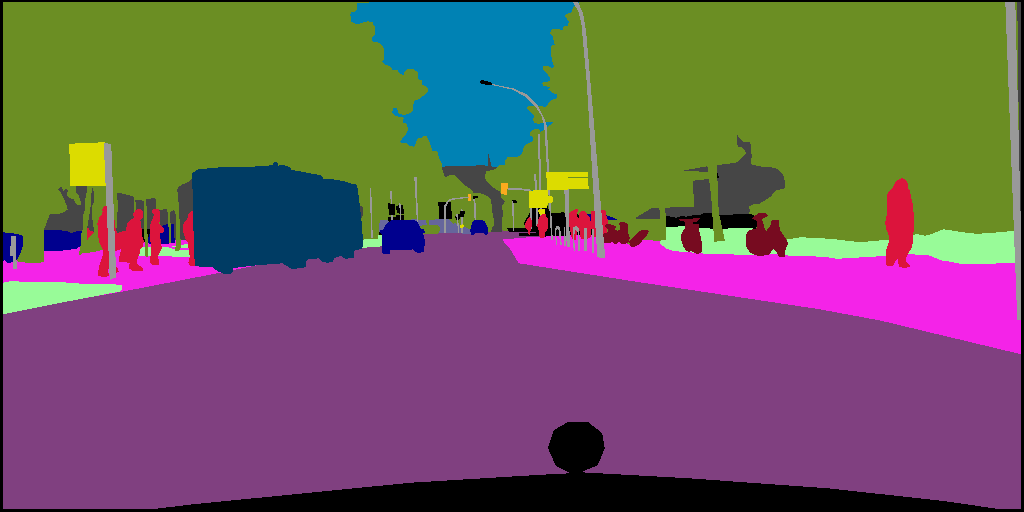} & 
   \includegraphics[width=\imgsize]{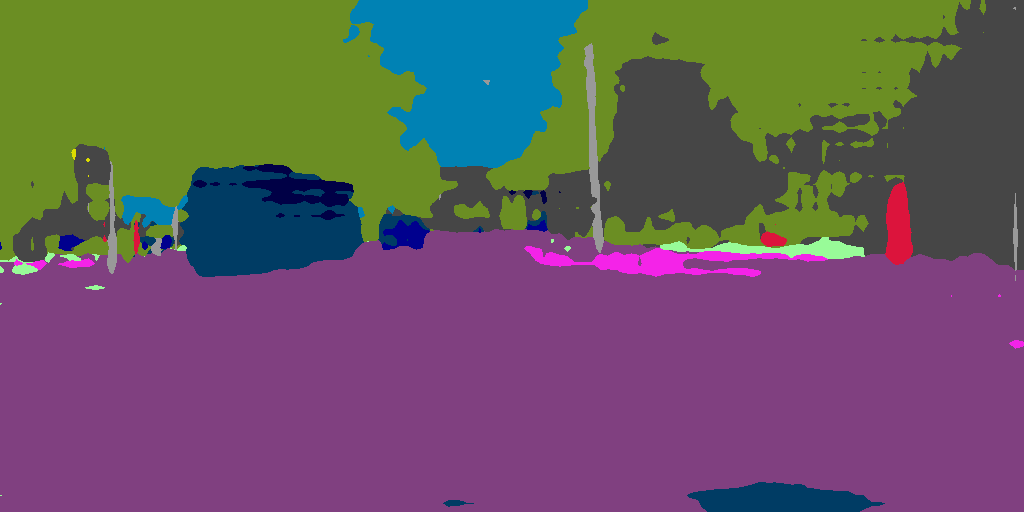} & 
   \includegraphics[width=\imgsize]{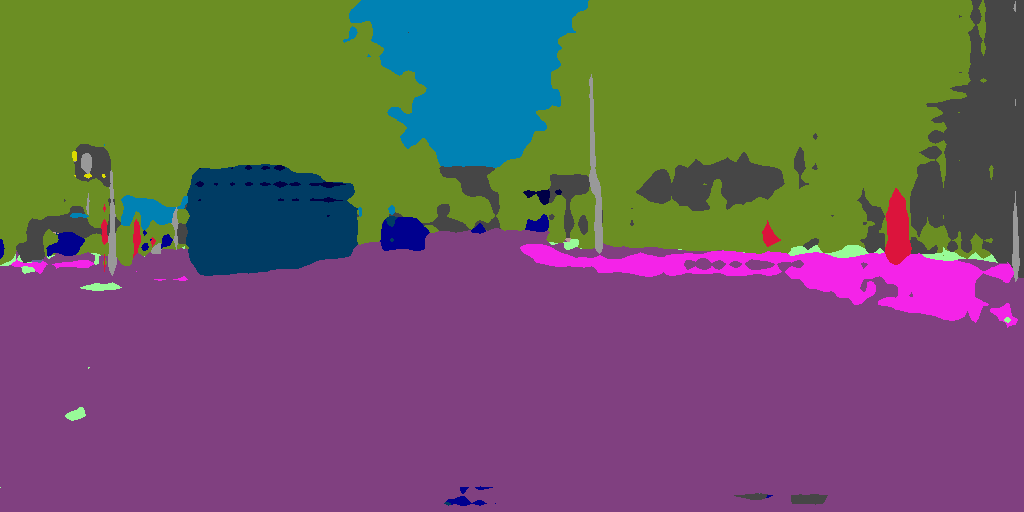} & 
   \includegraphics[width=\imgsize]{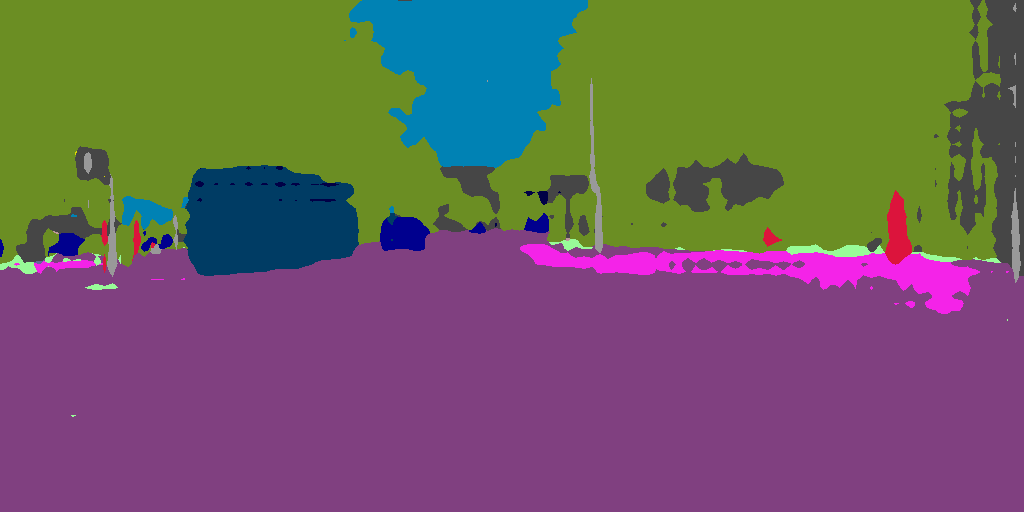} &
   \includegraphics[width=\imgsize]{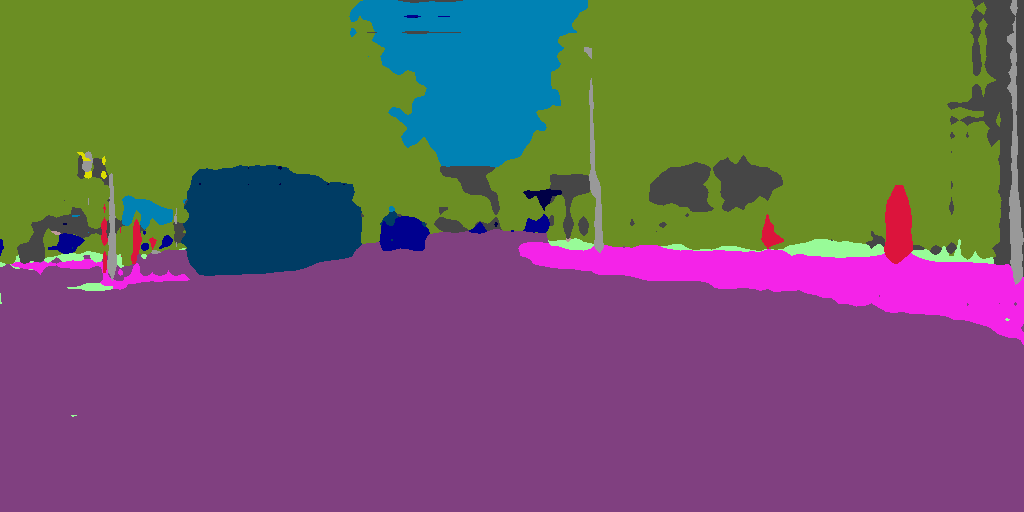} \\    
   
   &
   \includegraphics[width=\imgsize]{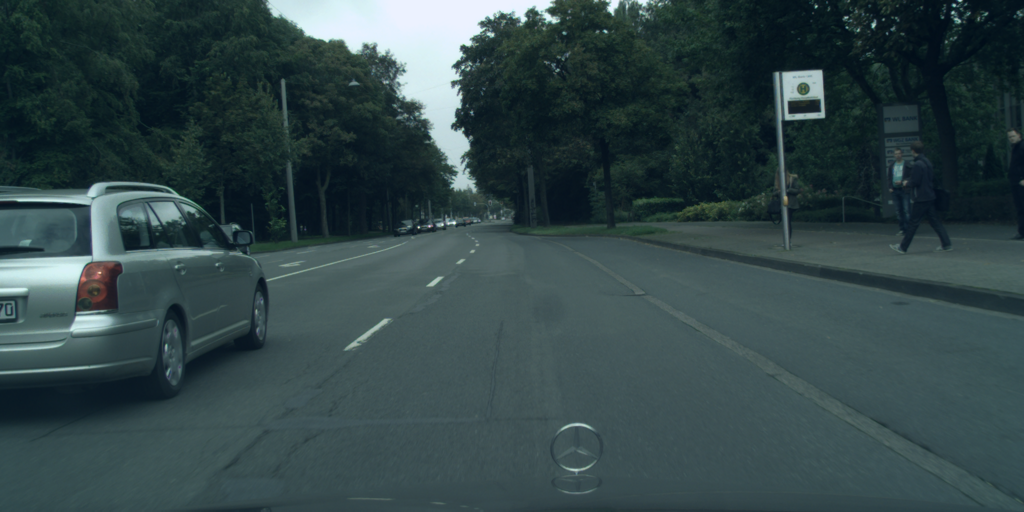} &
   \includegraphics[width=\imgsize]{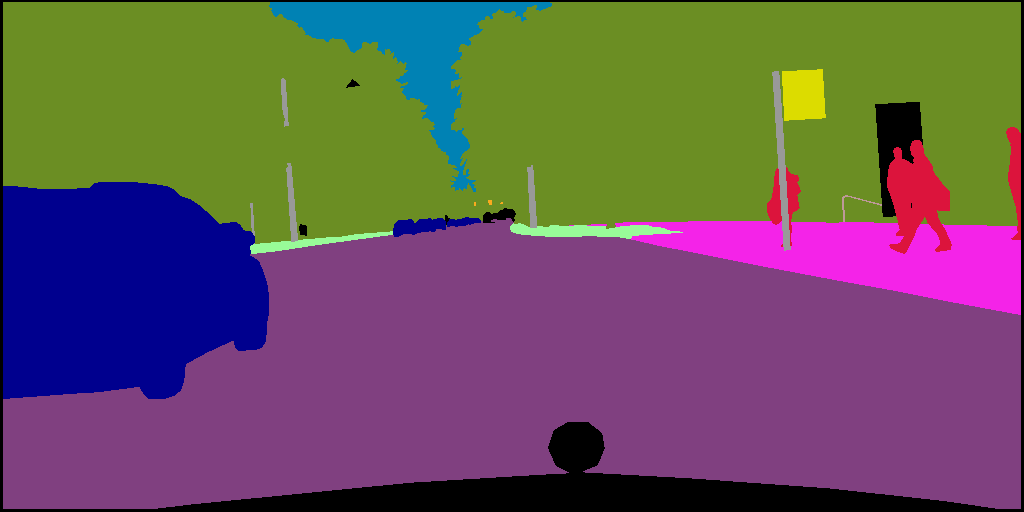} & 
   \includegraphics[width=\imgsize]{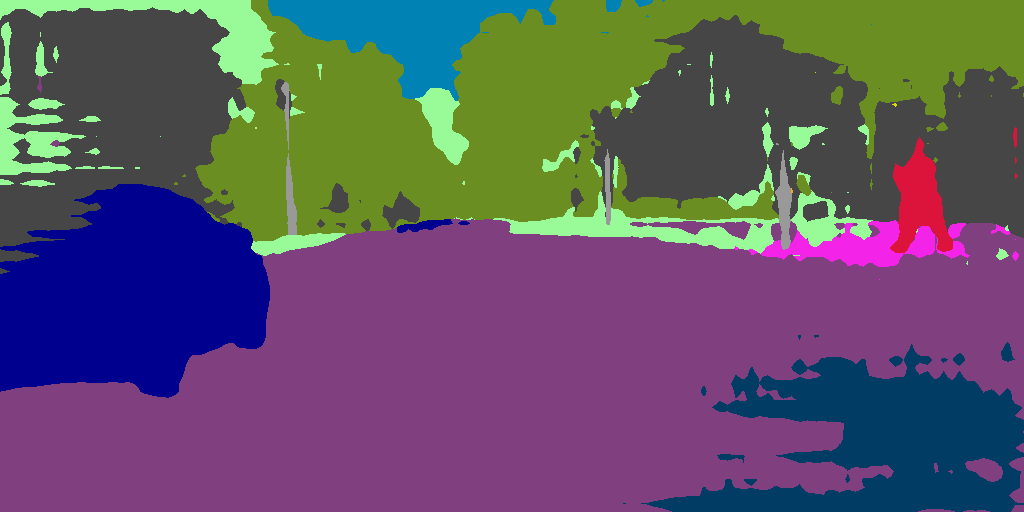} & 
   \includegraphics[width=\imgsize]{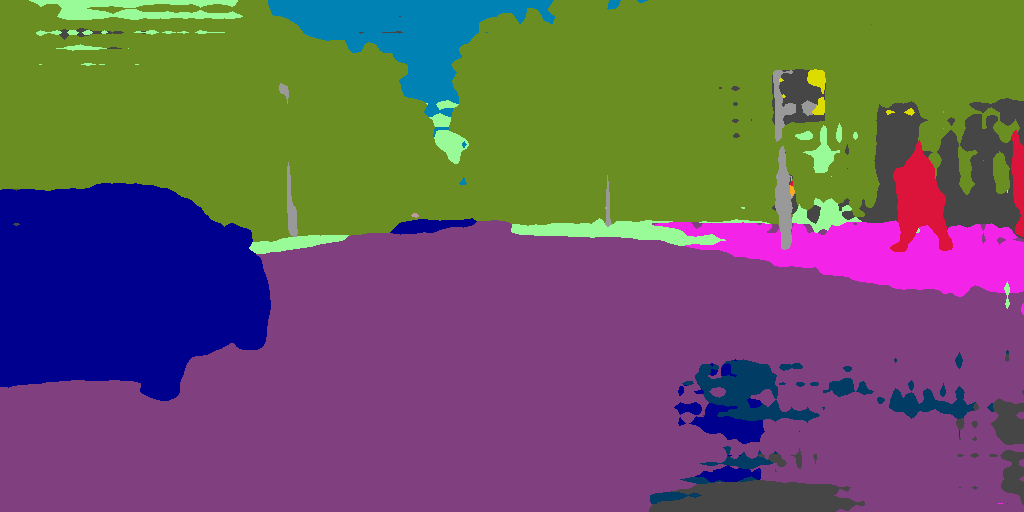} & 
   \includegraphics[width=\imgsize]{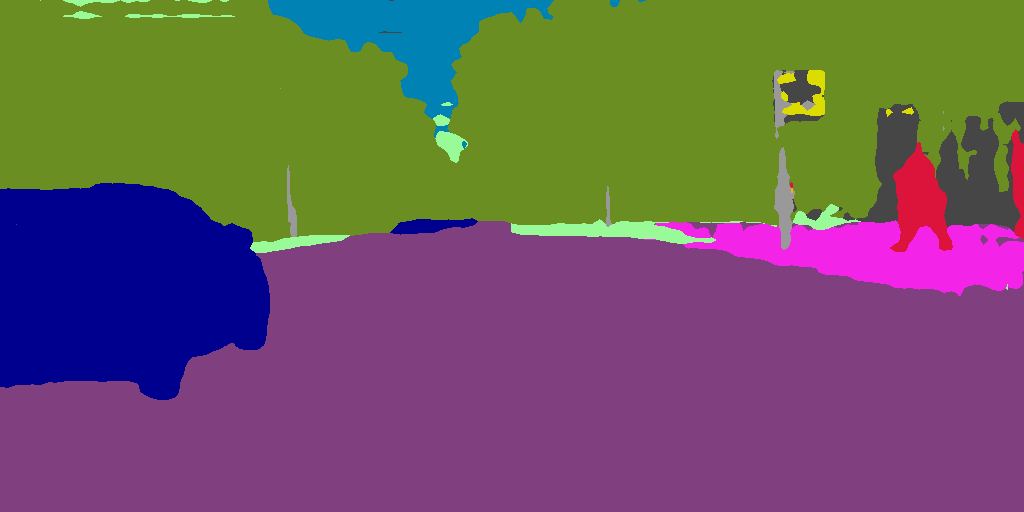} &
   \includegraphics[width=\imgsize]{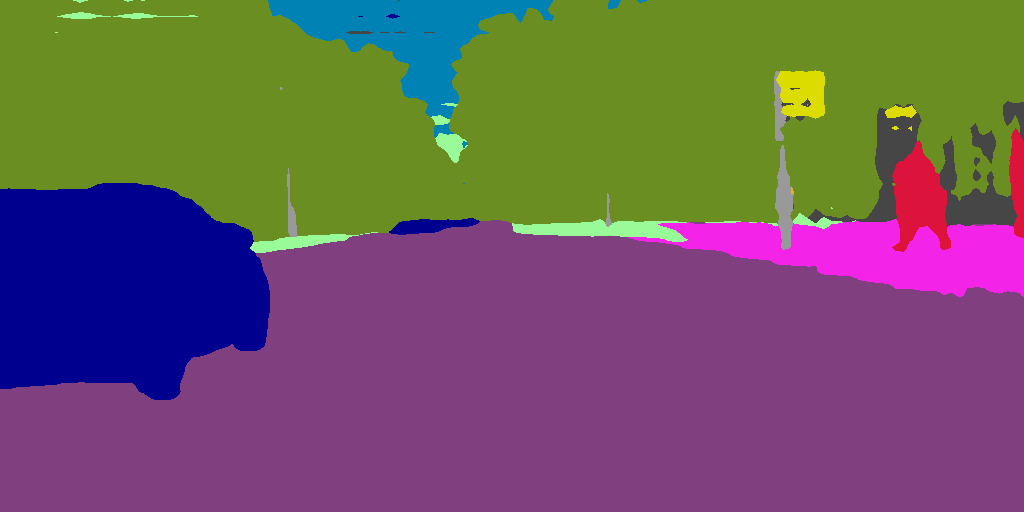} \\
   
   &
   \includegraphics[width=\imgsize]{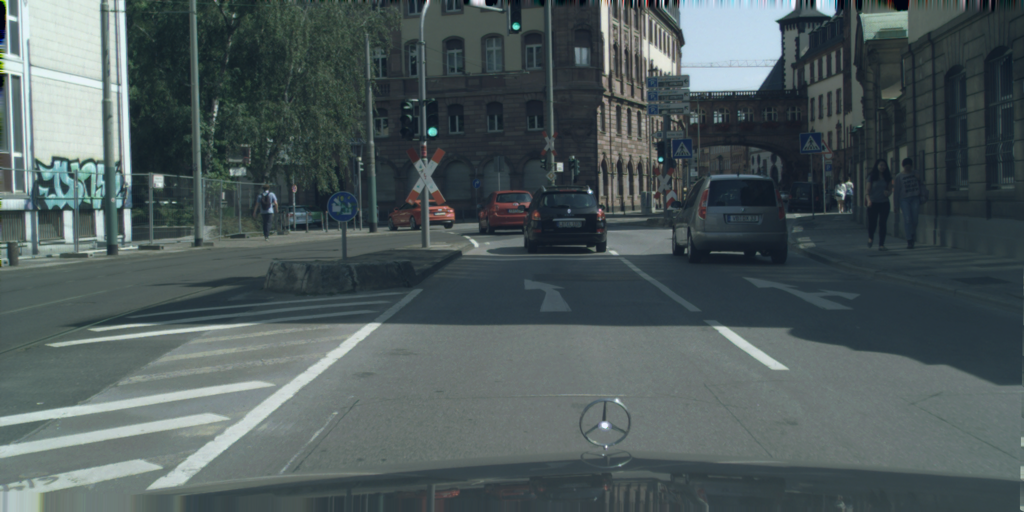} &
   \includegraphics[width=\imgsize]{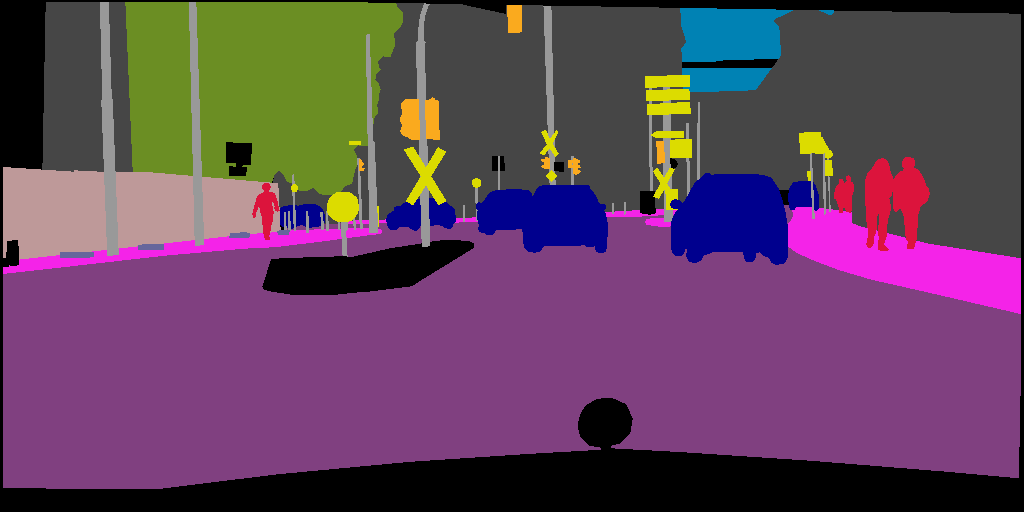} & 
   \includegraphics[width=\imgsize]{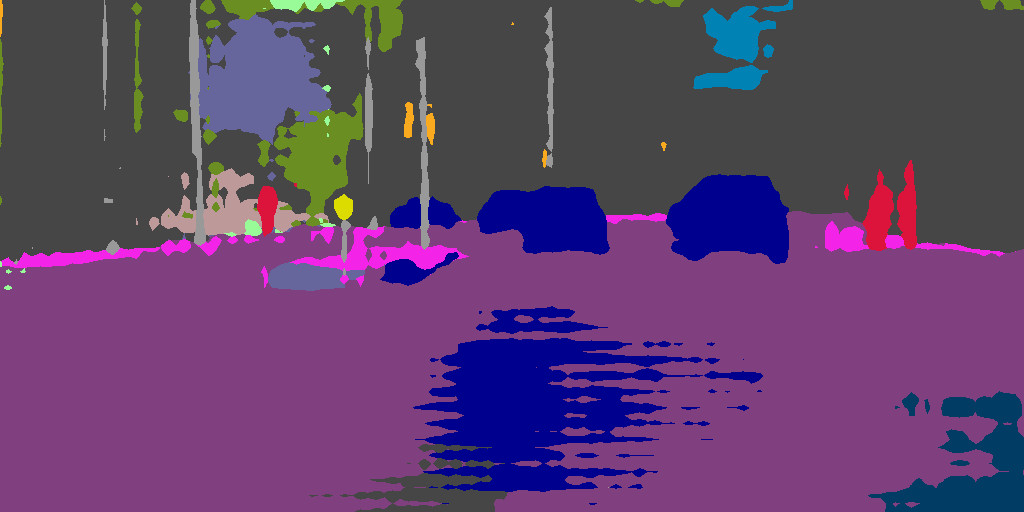} & 
   \includegraphics[width=\imgsize]{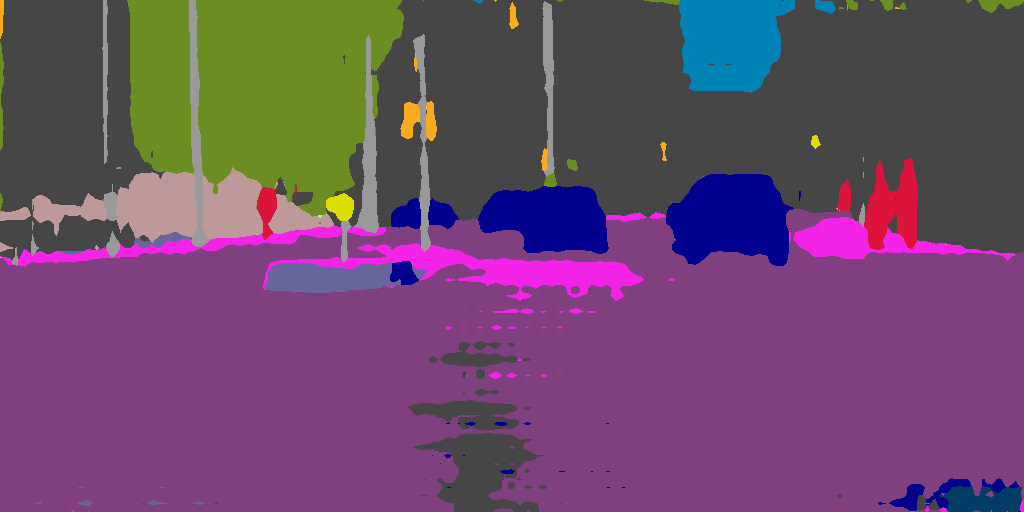} & 
   \includegraphics[width=\imgsize]{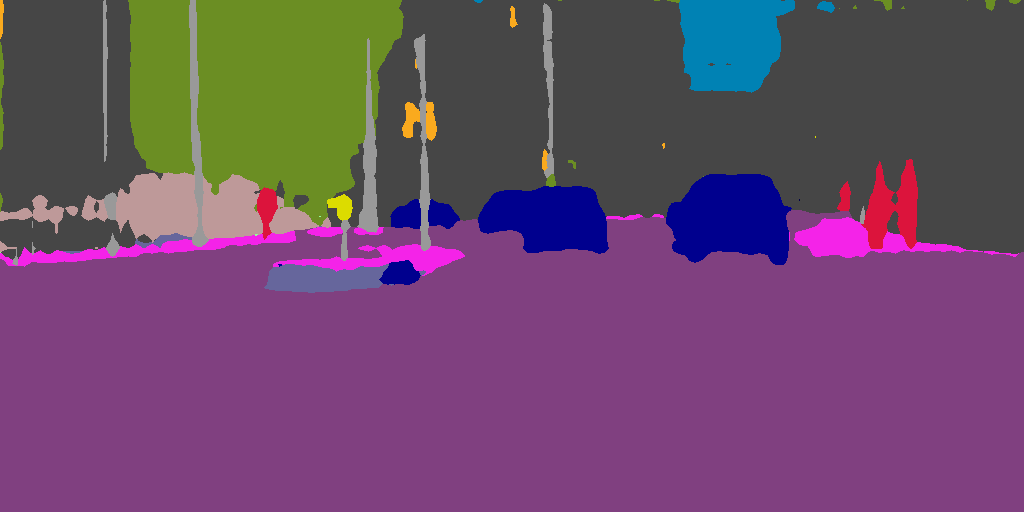} &
   \includegraphics[width=\imgsize]{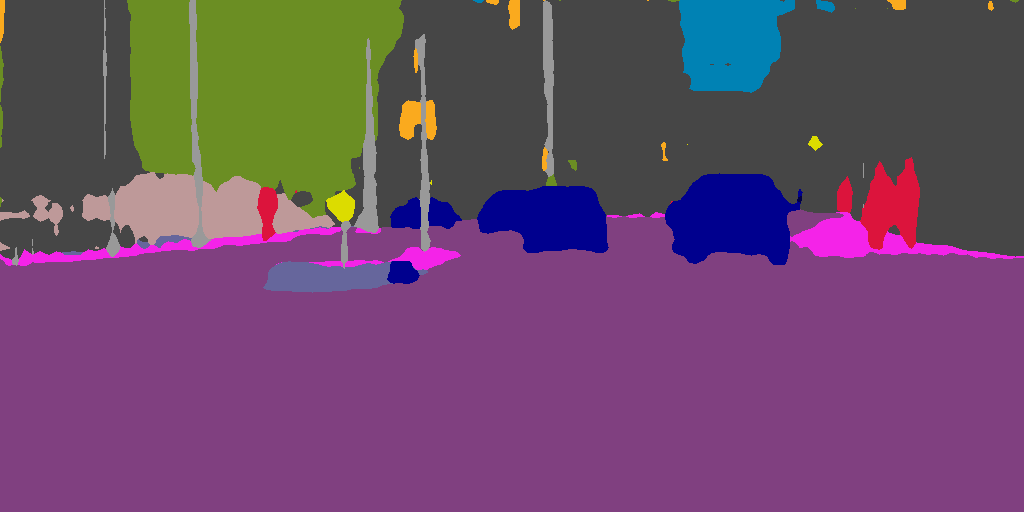} \\%[-0.1em] 
   
   \midrule 
   \rule{0pt}{41pt}
   
   \multirow{1}{*}{\rotatebox{90}{SYNTHIA $\rightarrow$ Cityscapes}} &
   \includegraphics[width=\imgsize]{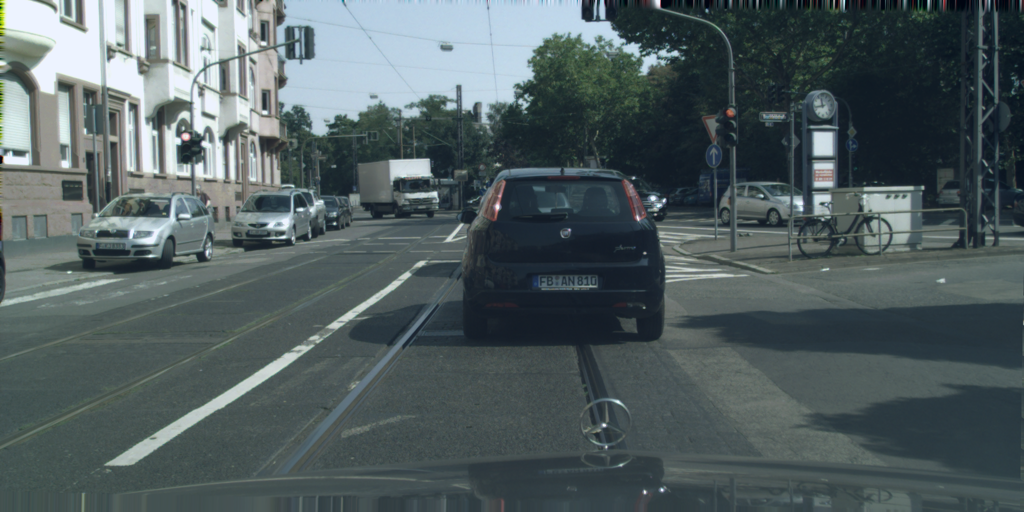} &
   \includegraphics[width=\imgsize]{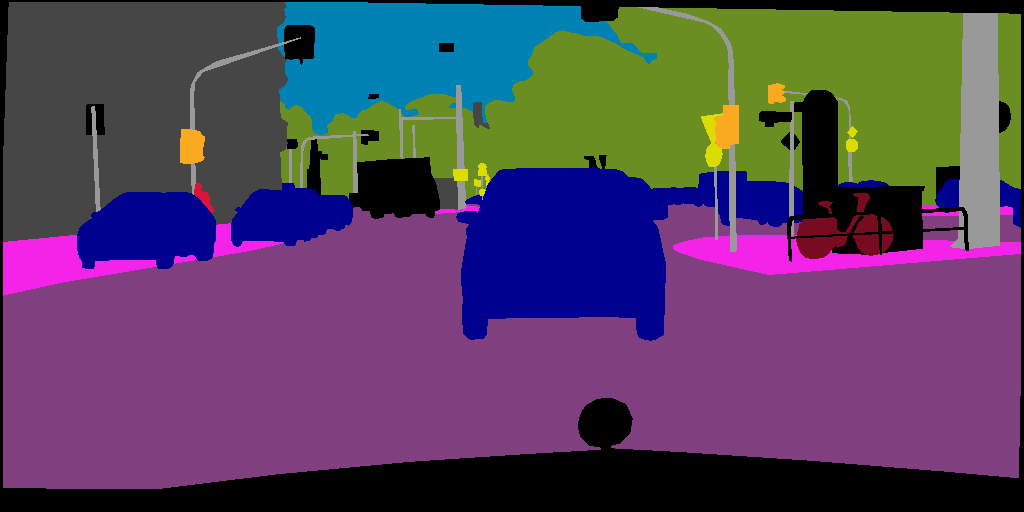} & 
   \includegraphics[width=\imgsize]{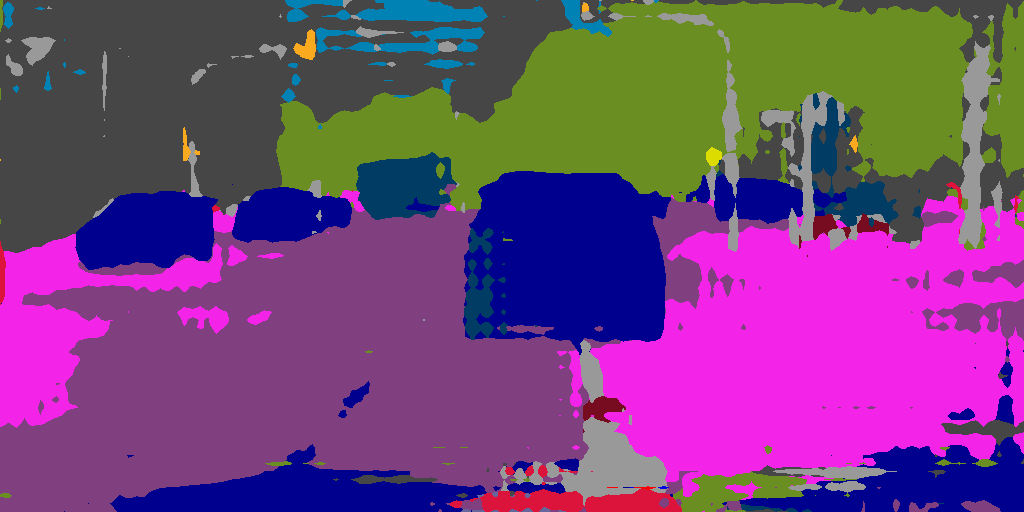} & 
   \includegraphics[width=\imgsize]{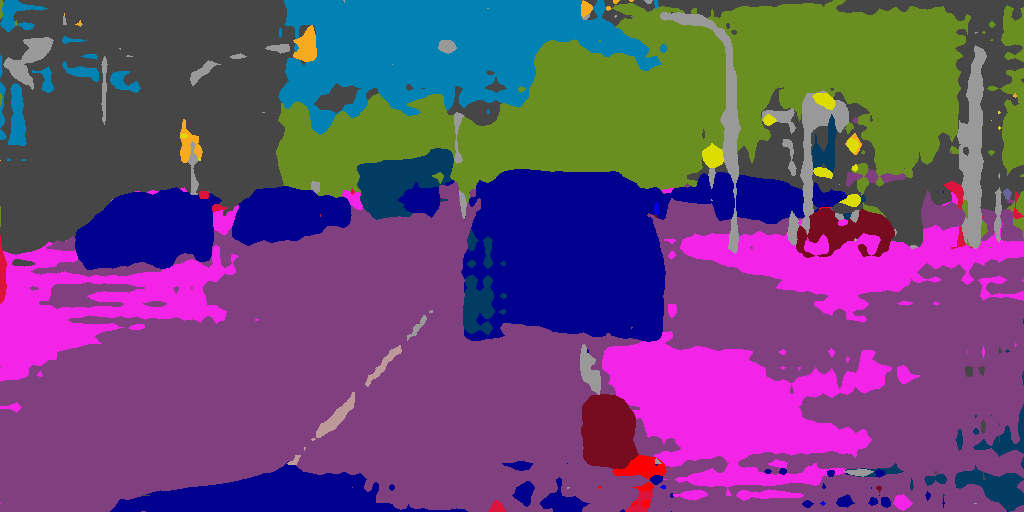} & 
   \includegraphics[width=\imgsize]{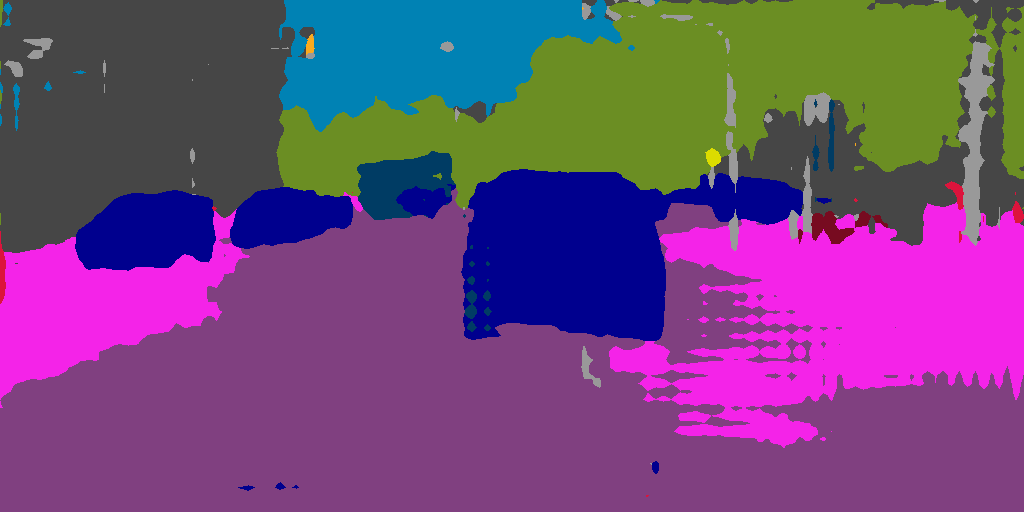} &
   \includegraphics[width=\imgsize]{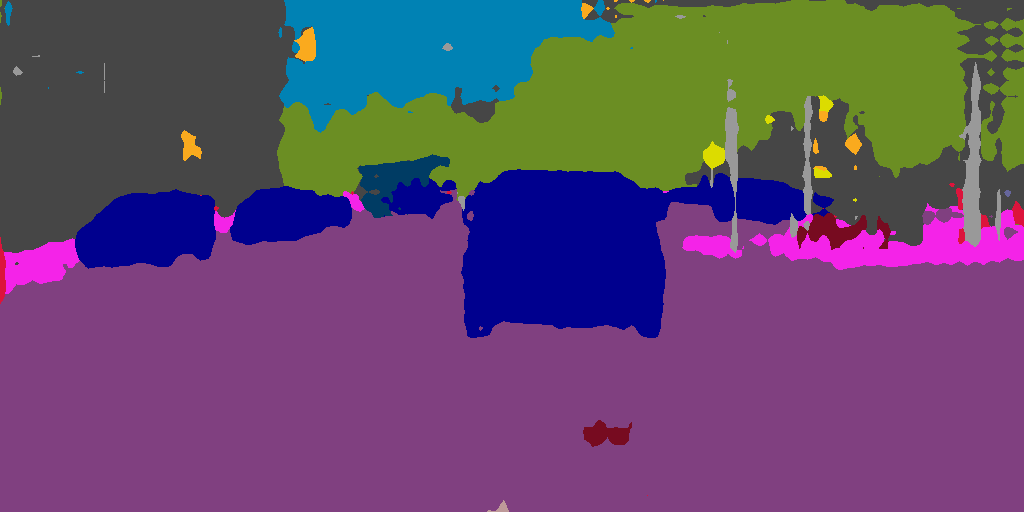} \\ 
   
   &
   \includegraphics[width=\imgsize]{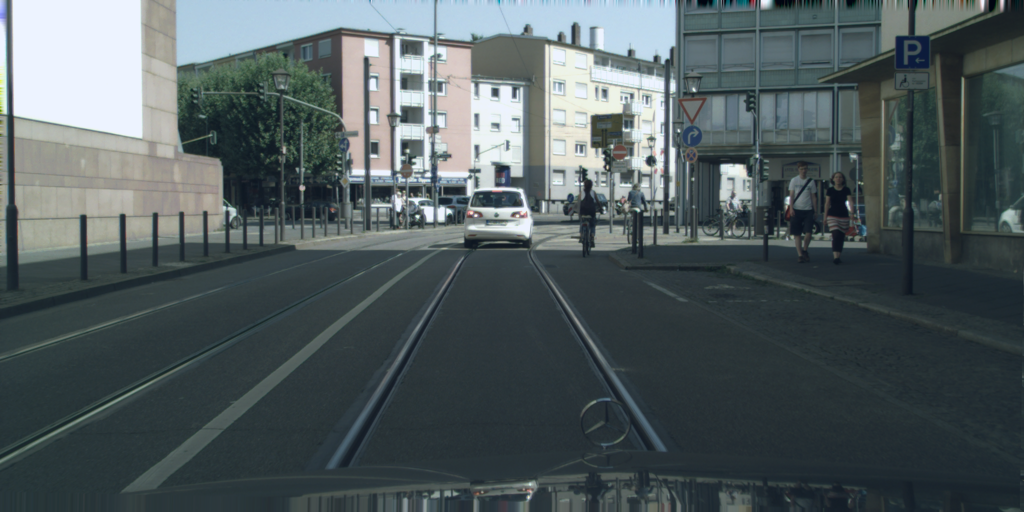} &
   \includegraphics[width=\imgsize]{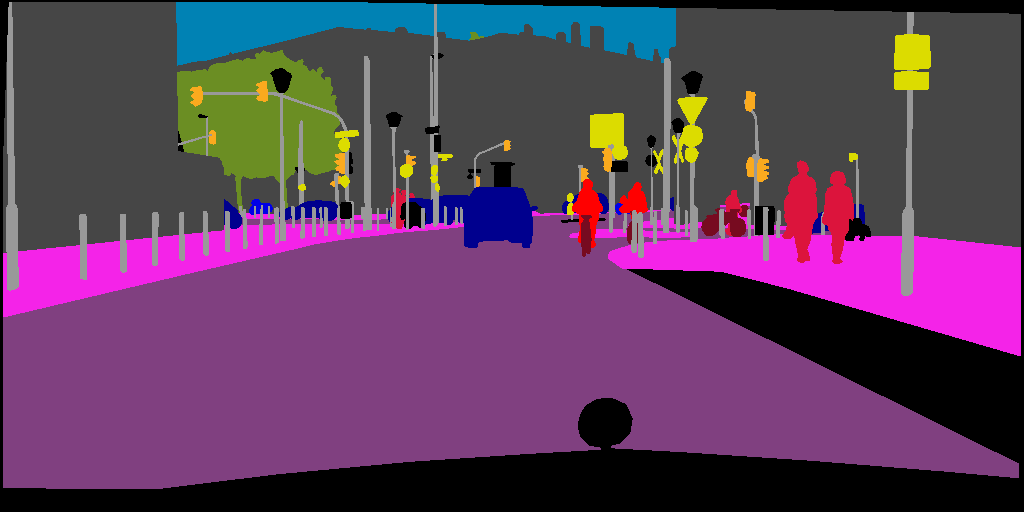} & 
   \includegraphics[width=\imgsize]{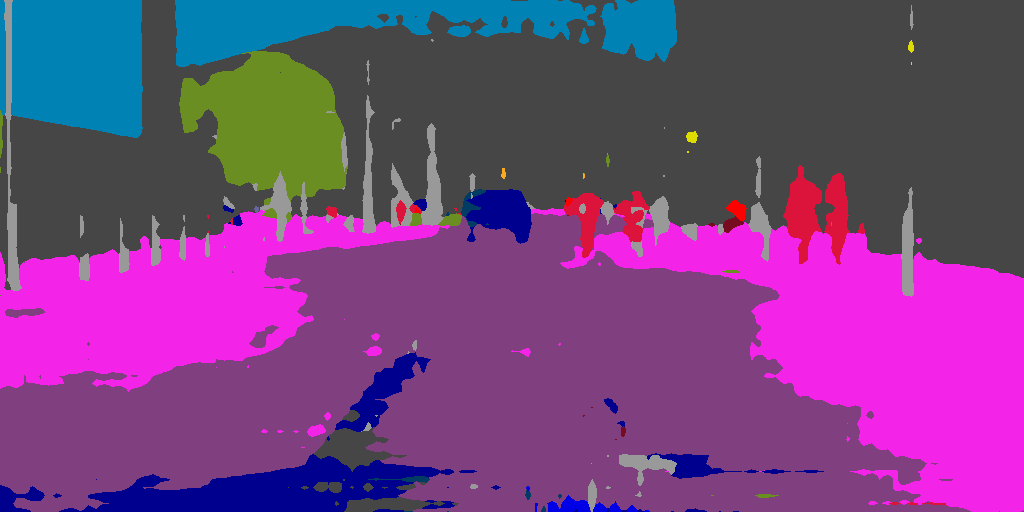} & 
   \includegraphics[width=\imgsize]{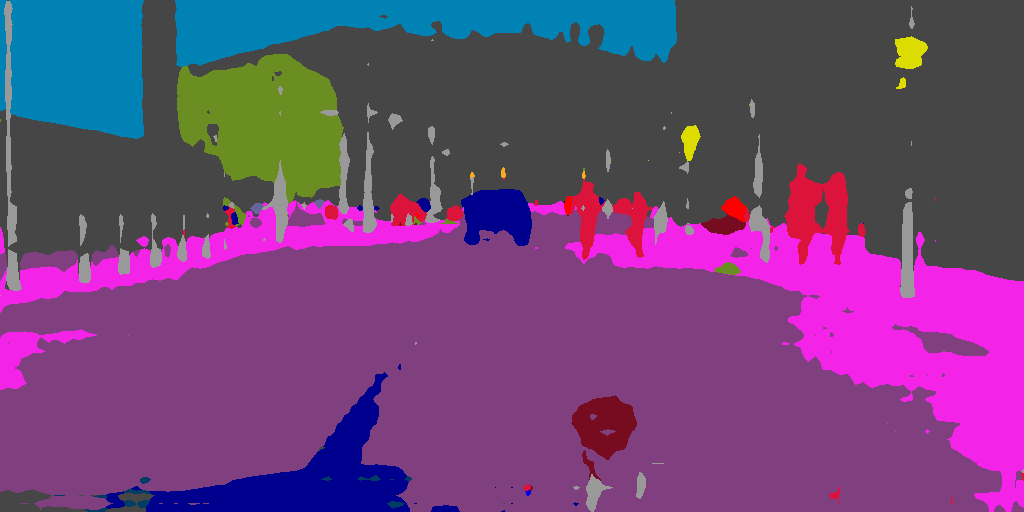} & 
   \includegraphics[width=\imgsize]{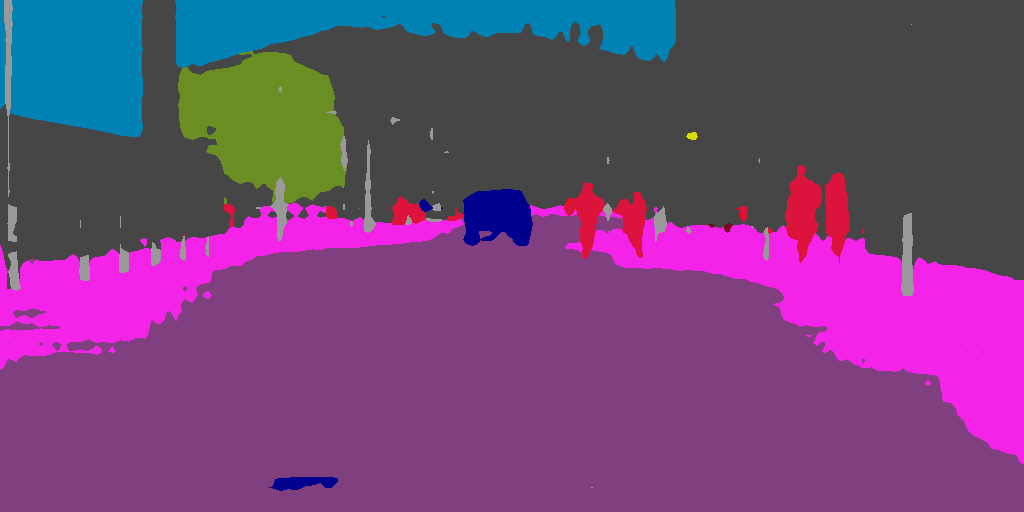} &
   \includegraphics[width=\imgsize]{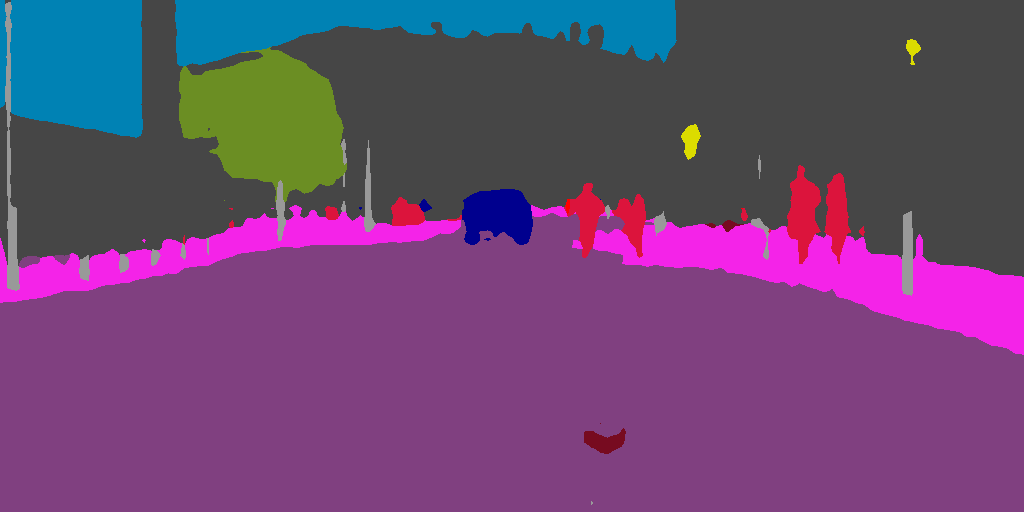} \\    
   
   &
   \includegraphics[width=\imgsize]{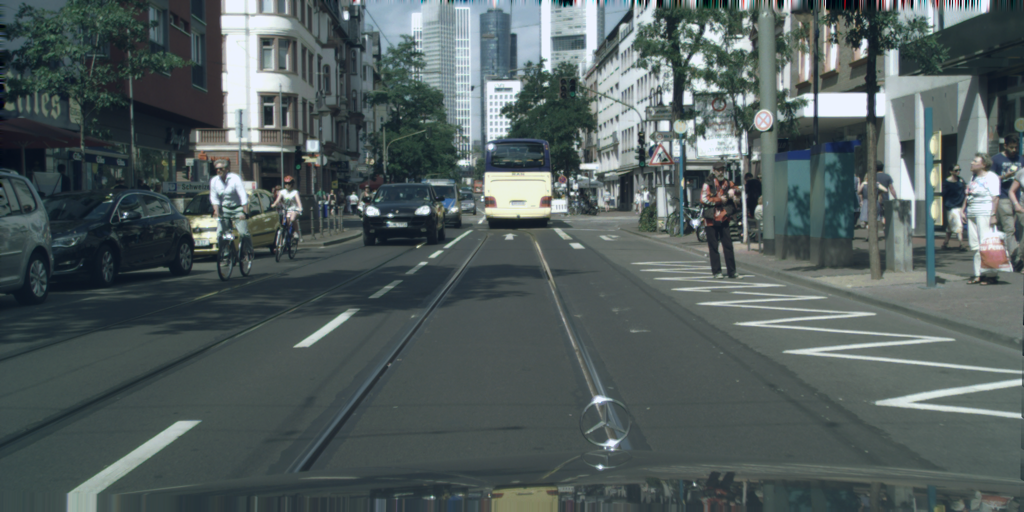} &
   \includegraphics[width=\imgsize]{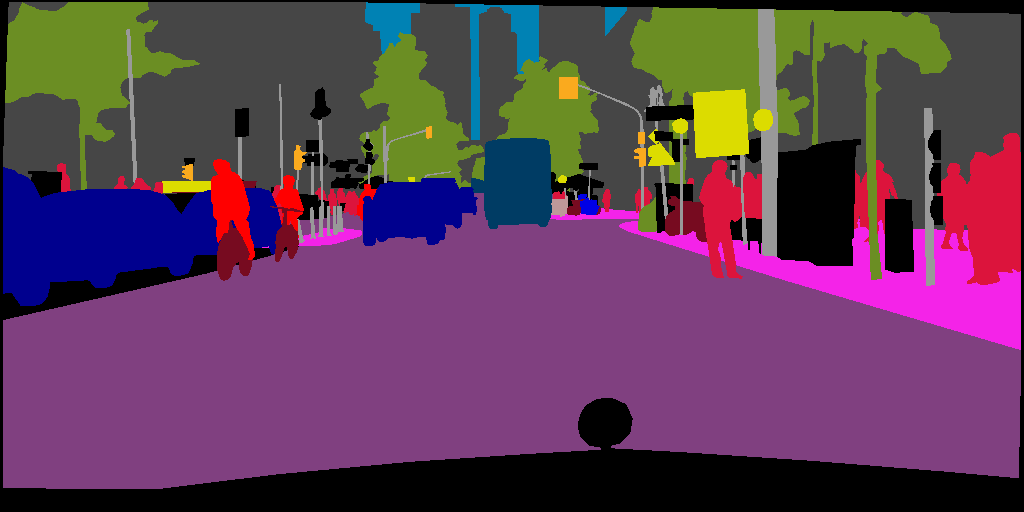} & 
   \includegraphics[width=\imgsize]{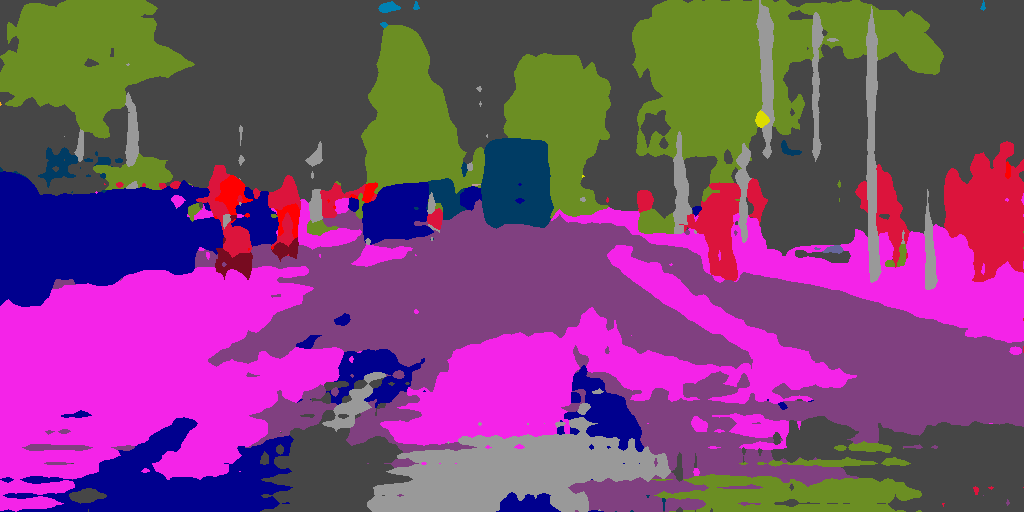} & 
   \includegraphics[width=\imgsize]{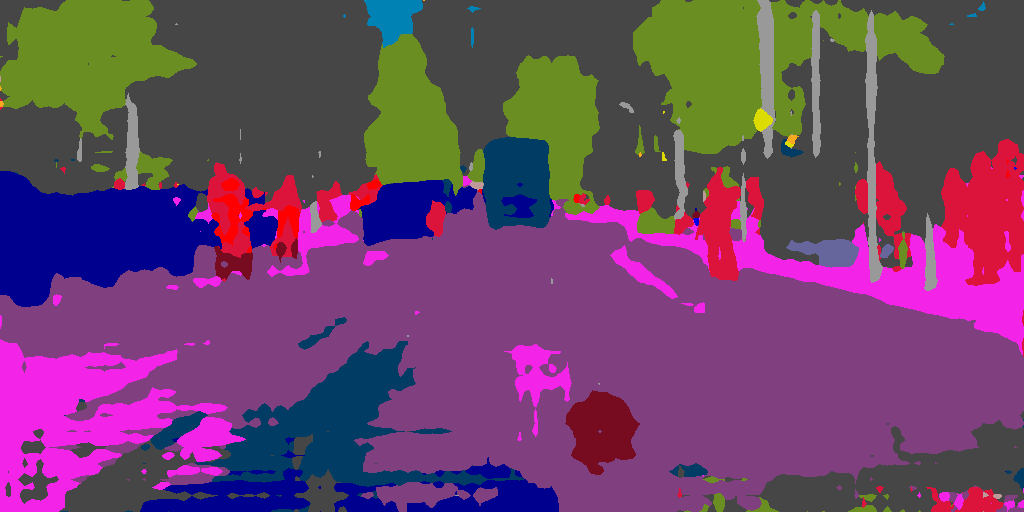} & 
   \includegraphics[width=\imgsize]{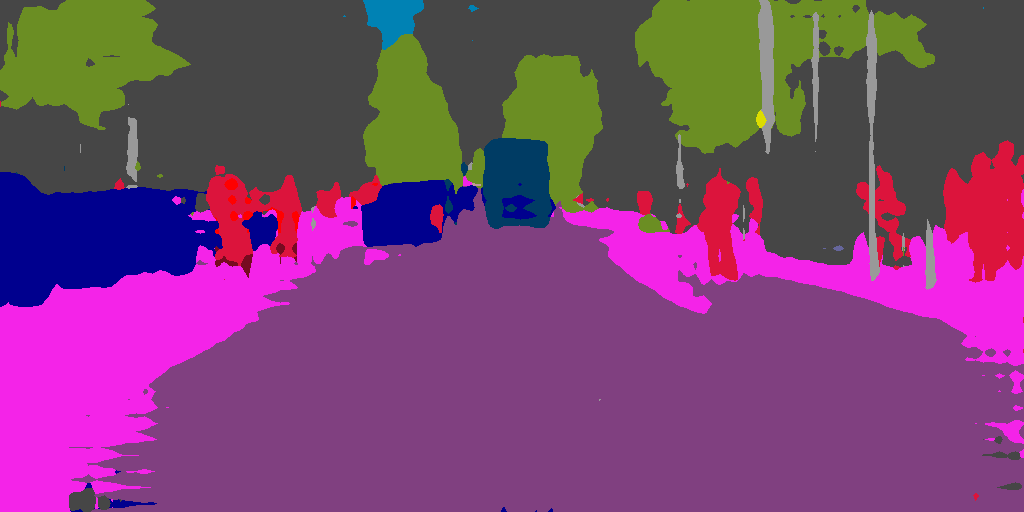} &
   \includegraphics[width=\imgsize]{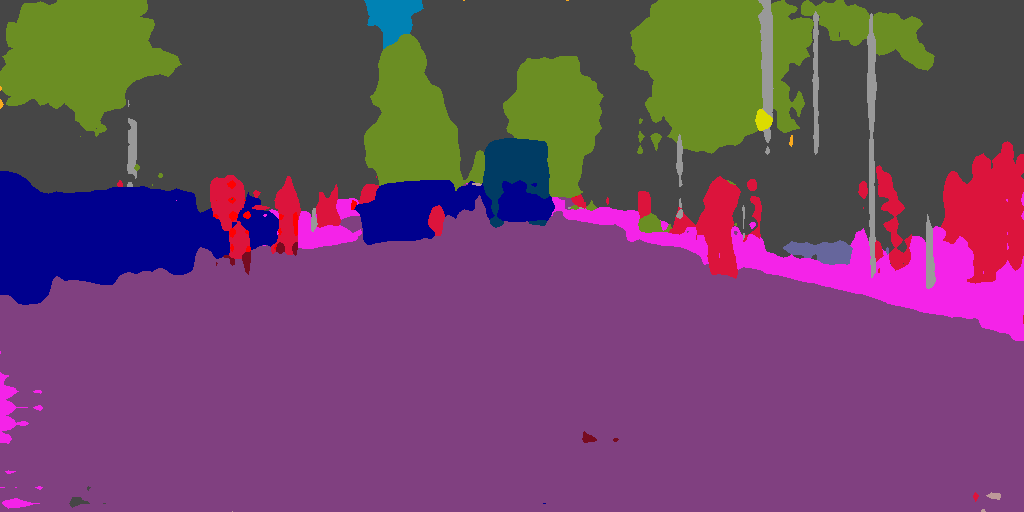} \\
   
   &
   \includegraphics[width=\imgsize]{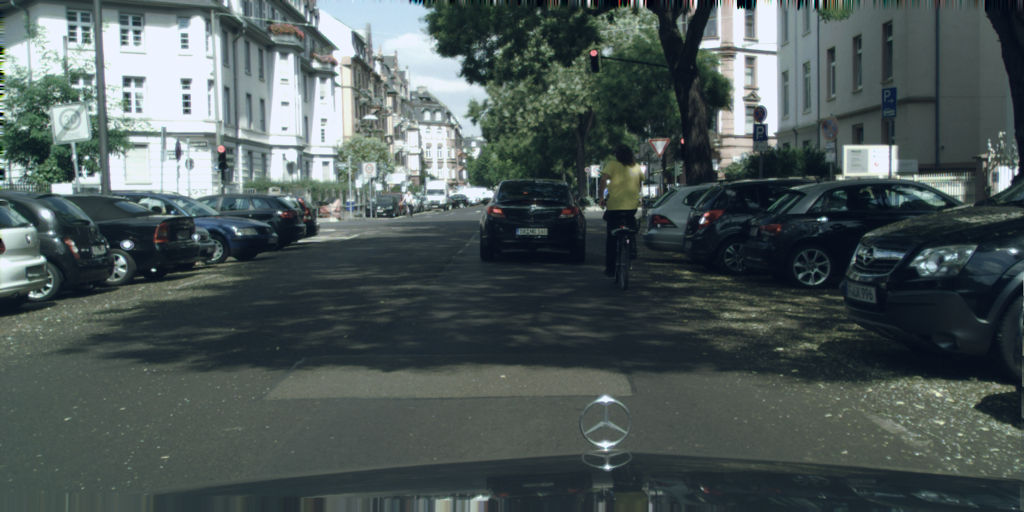} &
   \includegraphics[width=\imgsize]{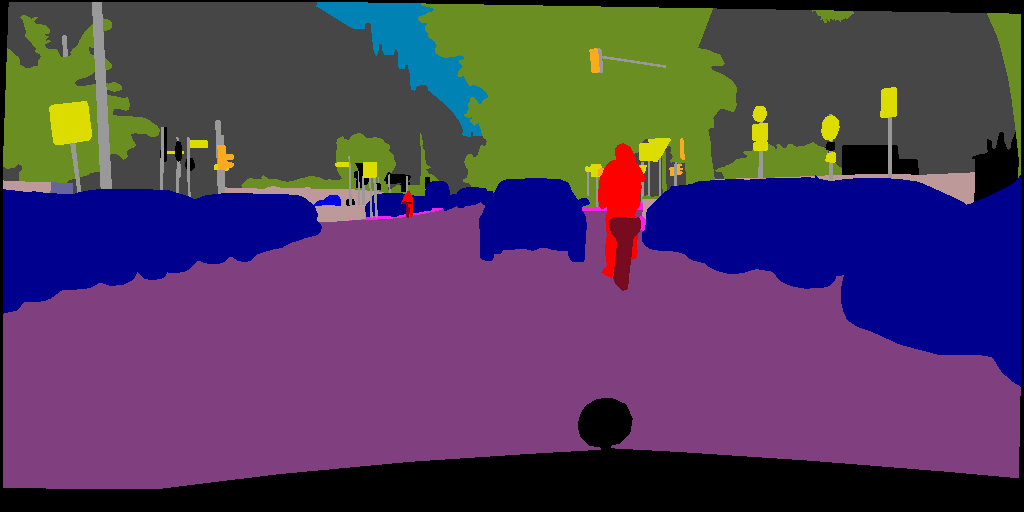} & 
   \includegraphics[width=\imgsize]{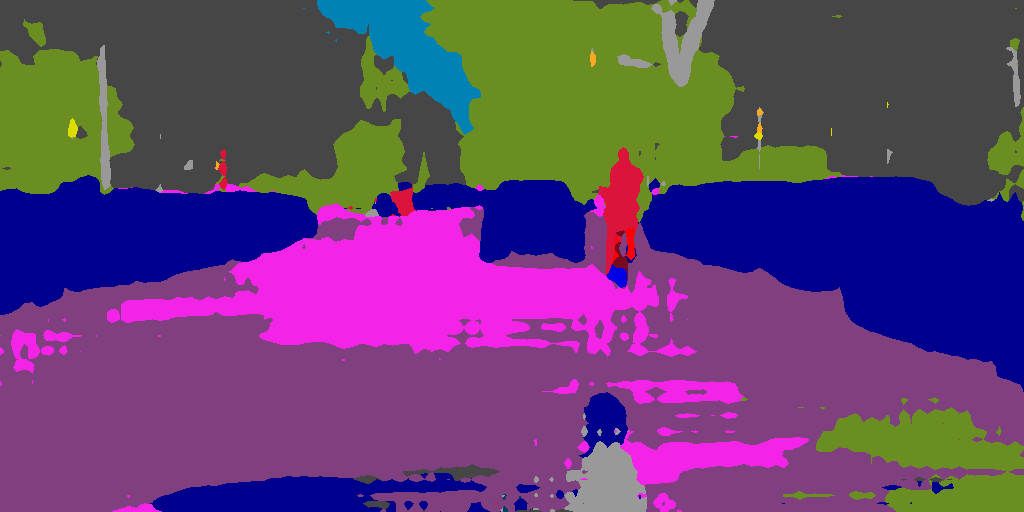} & 
   \includegraphics[width=\imgsize]{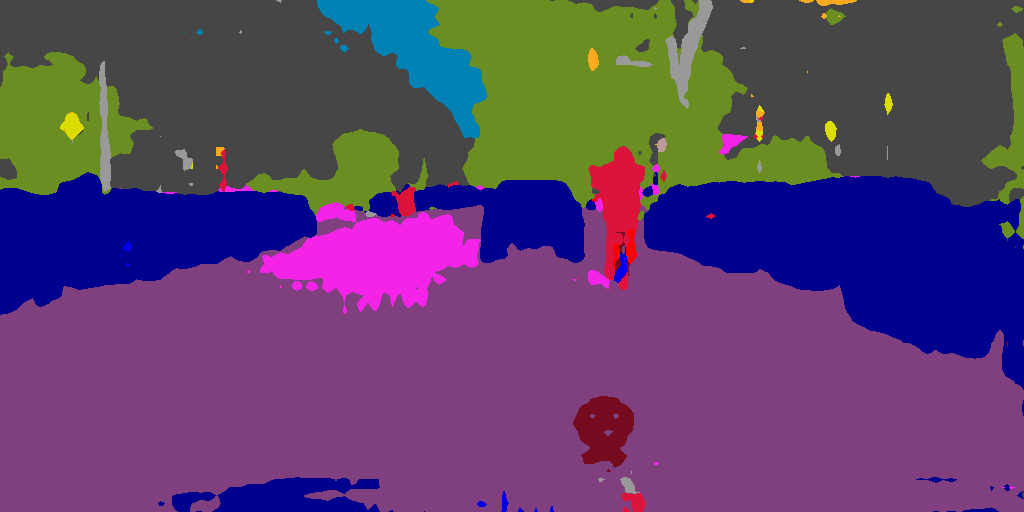} & 
   \includegraphics[width=\imgsize]{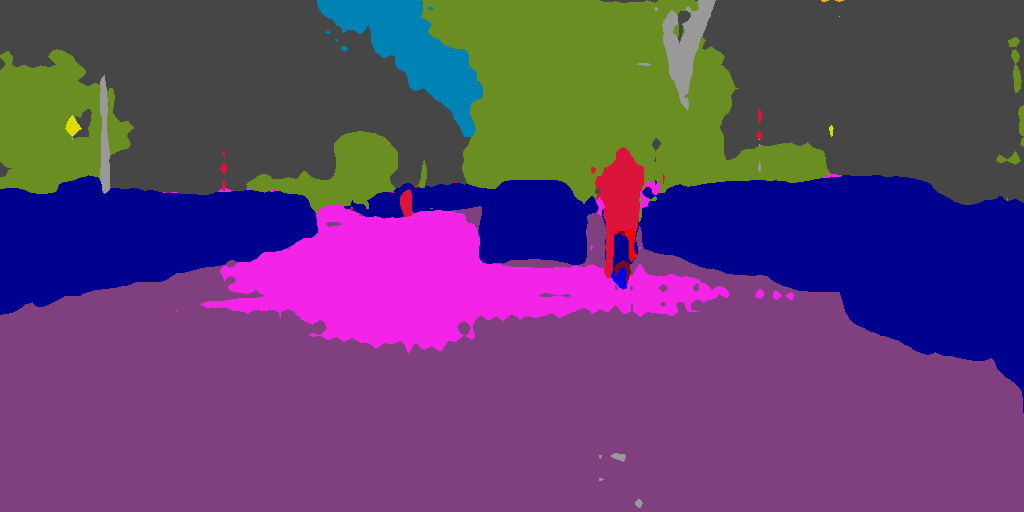} &
   \includegraphics[width=\imgsize]{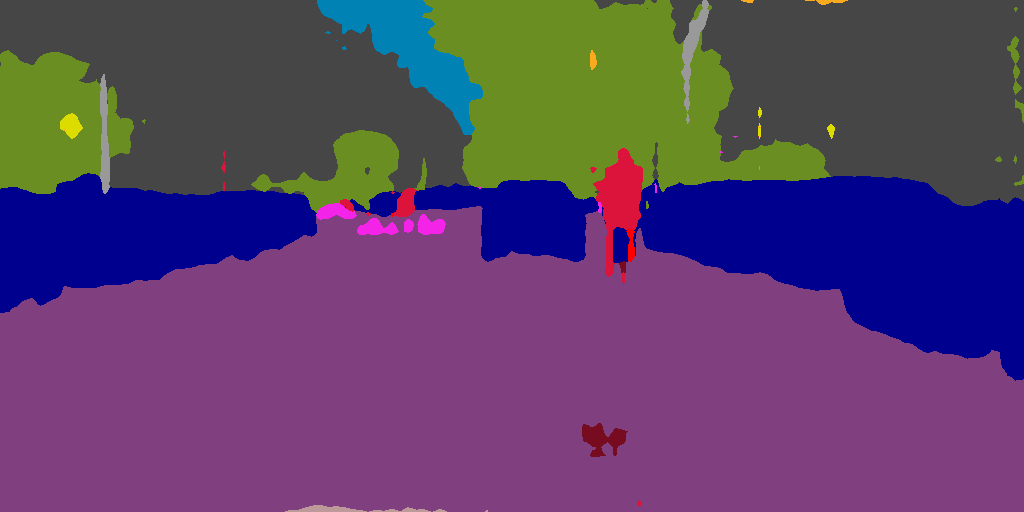} \\
   
  \multicolumn{1}{c}{} & \multicolumn{1}{c}{Target Images} & Ground Truth & Source Only  & Ours ($\mathcal{L}_{cl}$) & MaxSquare IW \cite{Chen2019} & Ours ($\mathcal{L}_{tot}$)

\end{tabular}
\end{subfigure}

\caption{Semantic segmentation of some sample scenes extracted from the Cityscapes validation target dataset when adaptation is performed from the GTA5 (top) and SYNTHIA (bottom) source datasets and the DeepLab-V2 with ResNet-101 backbone is employed as segmentation network (\textit{best viewed in colors}).}
\label{fig:qual_res}
\end{figure*}

\section{Ablation Studies}

In this section we provide further analysis for each novel loss component of our complete framework.

\subsection{Clustering Loss}

The effect introduced by the clustering objective is investigated by means of the t-SNE tool \cite{maaten2008visualizing}. 
The results are reported in Figure \ref{fig:plot_tsne}. 
In particular, we extract all feature vectors from a single target image and reduce their dimensionality from 2048 to 2, so that we able to visualize their disposition. 
Each single feature instance is then associated to a semantic class from the ground-truth segmentation map, with the categorization expressed by the standard color map we jointly report.   
To allow for the analysis of the aggregating effect of the clustering module, in Figure~\ref{fig:plot_tsne} we show the t-SNE plots in the \textit{source only} scenario, when only $\mathcal{L}_{cl}$ is enabled and when all adaptation modules are turned on ($\mathcal{L}_{tot}$). 
The effect brought by the clustering constraint is twofold. 
From one hand, we can see how features of the same class are more tightly clustered when $\mathcal{L}_{cl}$ is enabled, effect which is even further amplified by the class-conditional structural regularization provided by 
the other components of our work (see $\mathcal{L}_{tot}$). 
For instance, this is particularly visible in \textit{road} and \textit{vegetation} in row 2. 
From the other hand, we can appreciate that features belonging to different classes are more easily spaced apart, as shown in \textit{car} or \textit{person} in row 1 or in \textit{traffic light} in row 3.

\begin{figure*}[htbp]
\centering
\begin{subfigure}[htbp]{\textwidth}
\centering
\includegraphics[trim=3cm 0 3cm 0,clip,width=0.9\linewidth]{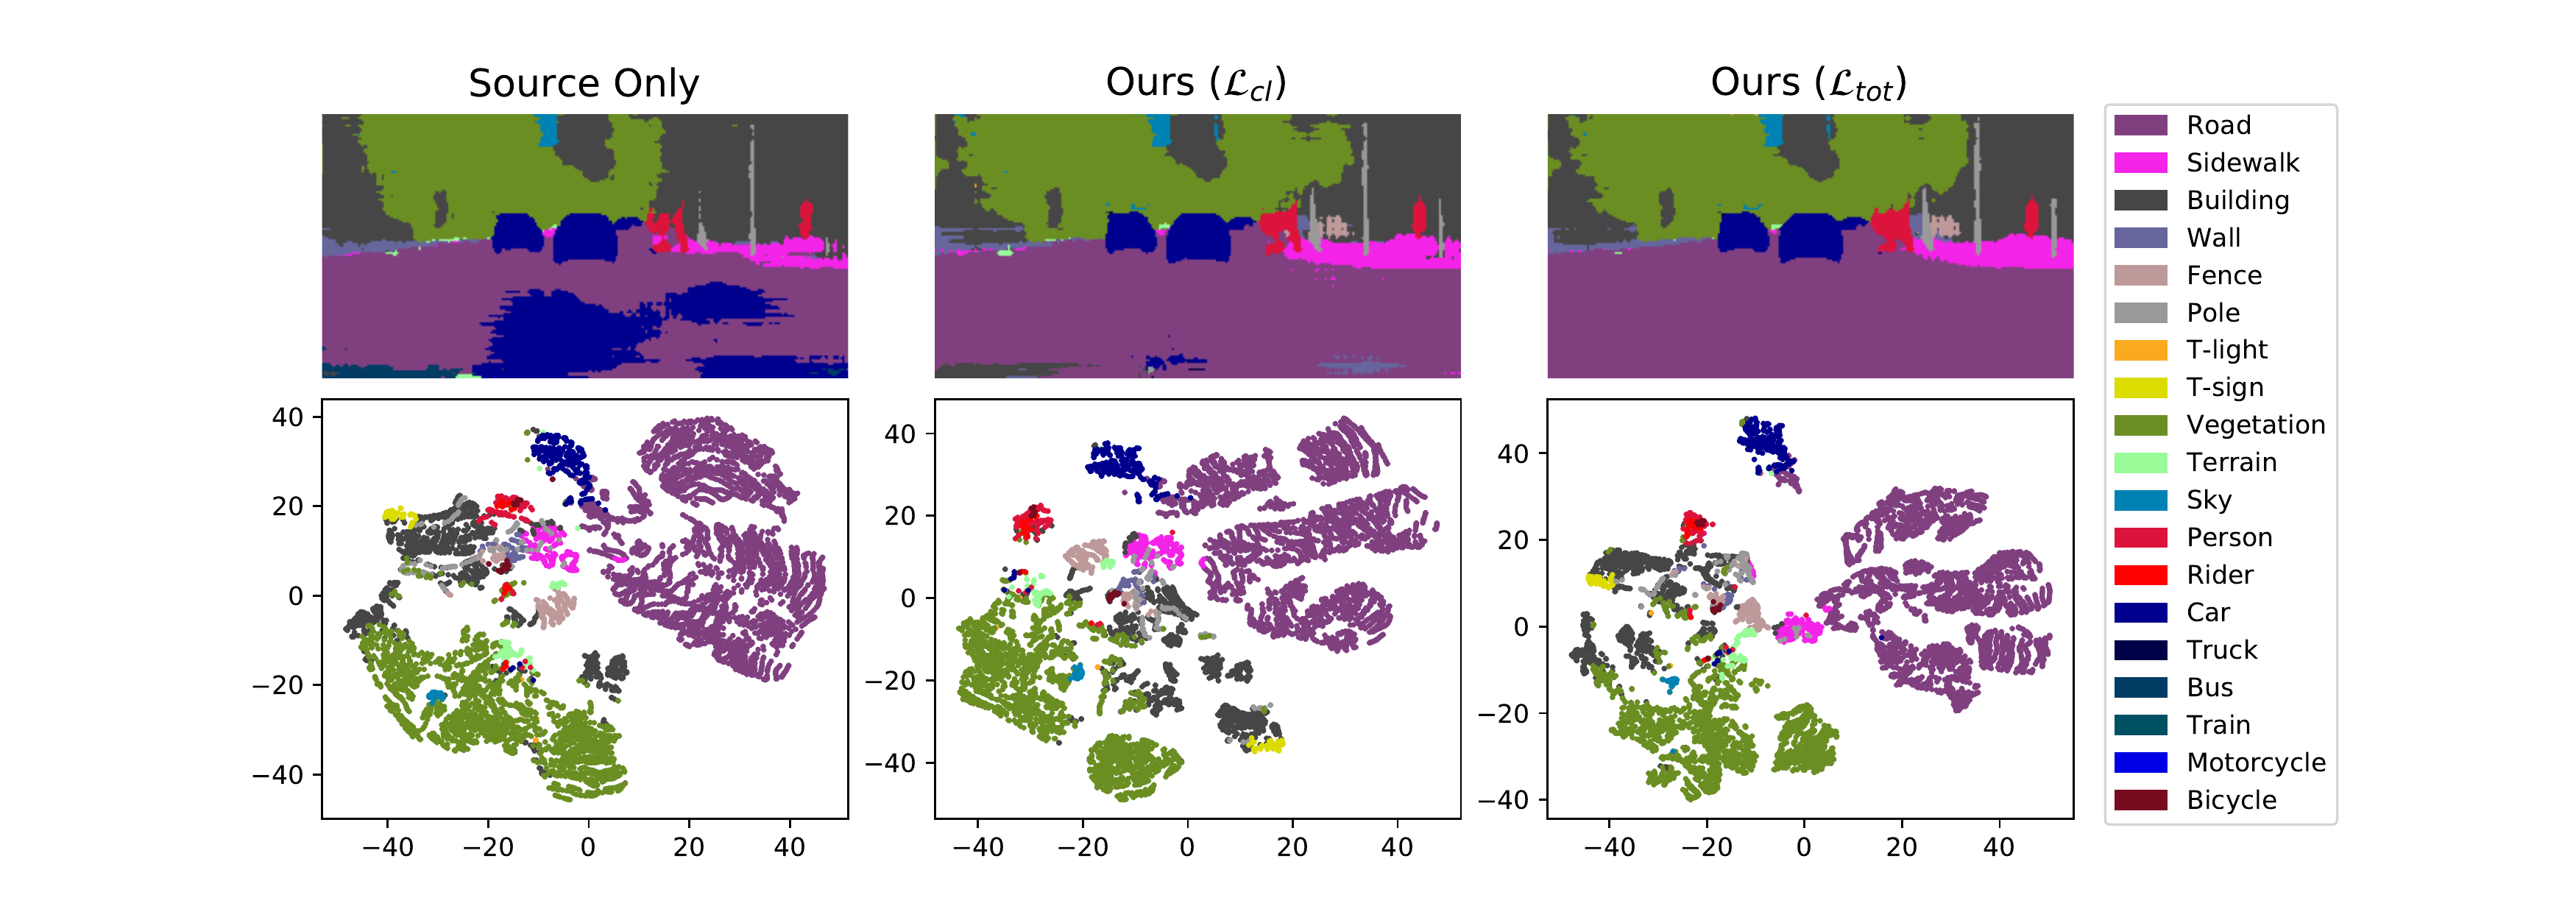}
\end{subfigure}
\begin{subfigure}[htbp]{\textwidth}
\centering
\includegraphics[trim=3cm 0 3cm 0,clip,width=0.9\linewidth]{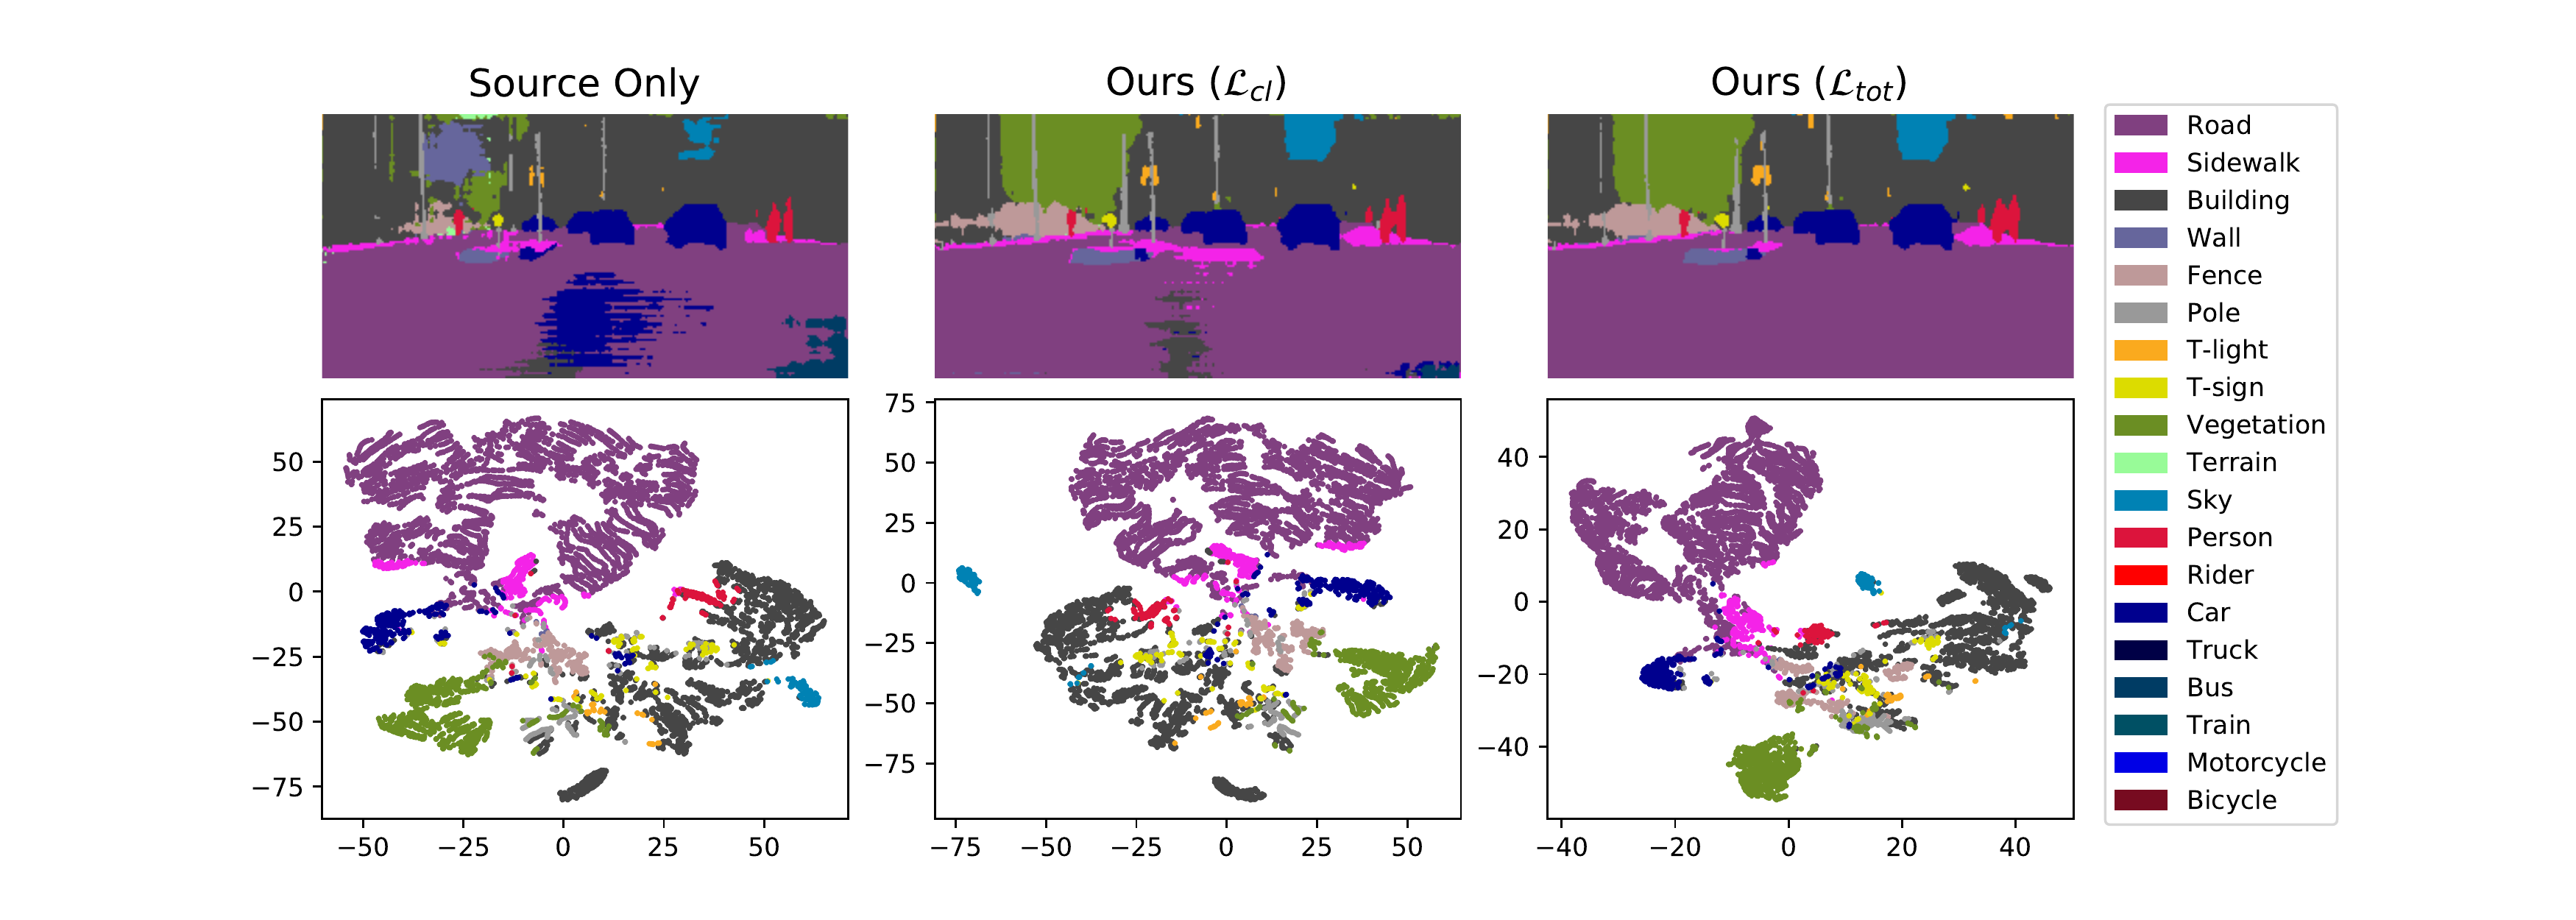}
\end{subfigure}
\begin{subfigure}[htbp]{\textwidth}
\centering
\includegraphics[trim=3cm 0 3cm 0,clip,width=0.9\linewidth]{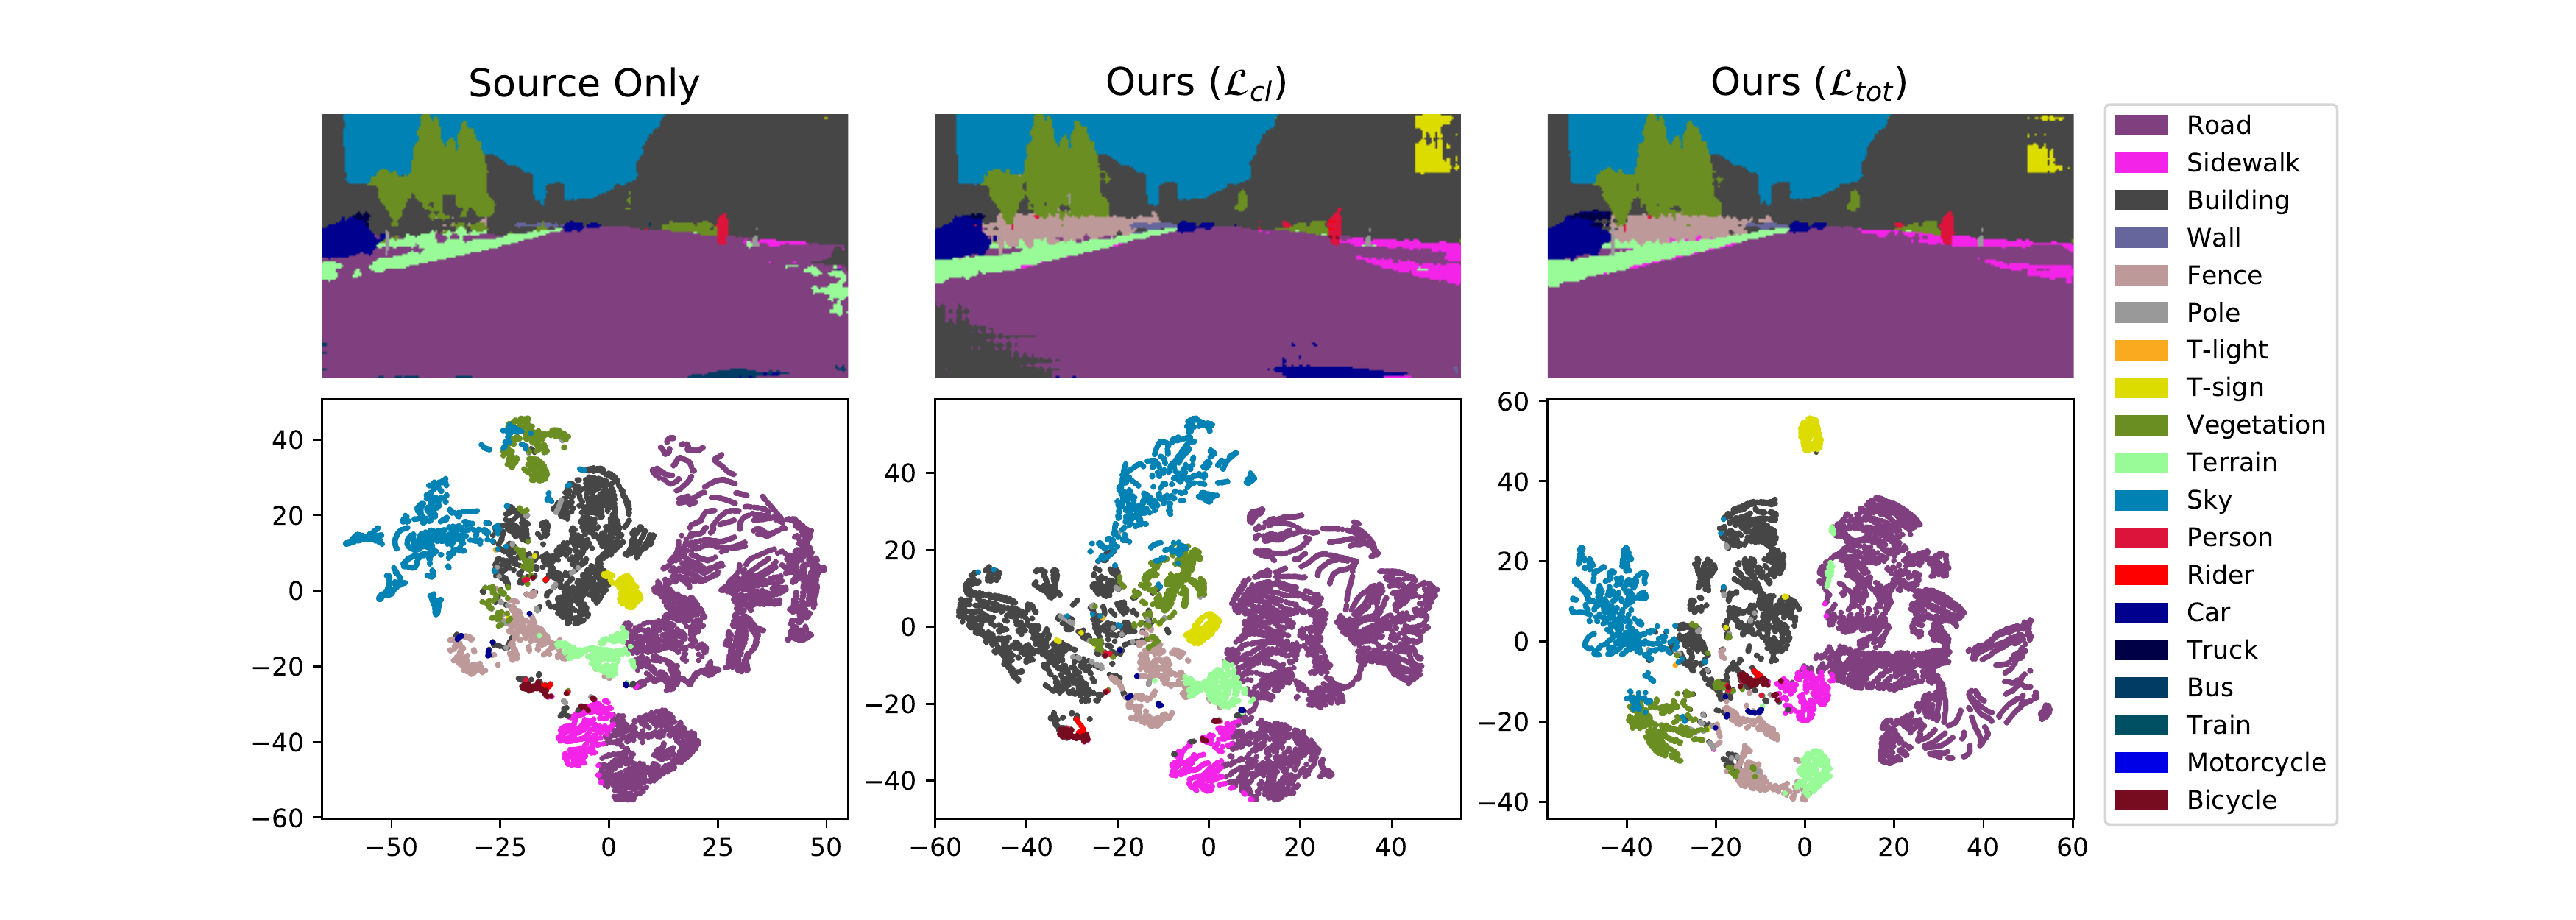}
\end{subfigure}

\caption{T-SNE computed over features of single images from the Cityscapes validation set when adapting from GTA5 (\textit{best viewed in colors}).}
\label{fig:plot_tsne}
\end{figure*}

\subsection{Orthogonality Loss}

We investigate the contribution of the orthogonality constraint $\mathcal{L}_{or}$ via a similarity score defined as an average class-wise cosine similarity measure. 
The cosine distance is first computed for every pair of feature vectors from a single target image. 
Then, the average values are taken over all features from the same class to get a score for each pair of semantic classes. 
The final values are computed by averaging over all images from the Cityscapes validation set. 

In Figure~\ref{fig:plot_similarity} we analyze the orthogonalizing action in three different configurations and we can clearly see that $\mathcal{L}_{or}$ causes the similarity score to significantly increase on almost all the classes (higher similarity reflects into lower orthogonality). 
To show the effect of the orthogonality constraint alone, we compare the \textit{source only} similarity score and the scenario with only $\mathcal{L}_{or}$ enabled (Figure~\ref{fig:plot_similarity}a). %(Figure~\ref{fig:plot_similaritya}). 
To investigate its effect when all the loss components are enabled, we compared the similarity scores of the full approach with respect to \textit{source only} (Figure~\ref{fig:plot_similarity}b) %(Figure~\ref{fig:plot_similarityb}) 
and to the case where all components but the $\mathcal{L}_{or}$ are enabled (Figure~\ref{fig:plot_similarity}c). %(Figure~\ref{fig:plot_similarityc}). 
The results are robust and coherent in showing an increased similarity score in the configurations where $\mathcal{L}_{or}$ is active.

The same considerations are visible in Figure~\ref{fig:orthogonality_matrix} in which the matrices of class-wise similarity scores are reported for the three aforementioned scenarios. In particular, we can see how the diagonal is much brighter (i.e., high similarity for classes with themselves) when $\mathcal{L}_{or}$ is added, while off-diagonal entries are darker.

\begin{figure*}[htbp]
\centering
\begin{subfigure}[t]{0.03\textwidth}
a)
\end{subfigure}
\begin{subfigure}[htbp]{0.7\textwidth}
\includegraphics[width=\linewidth]{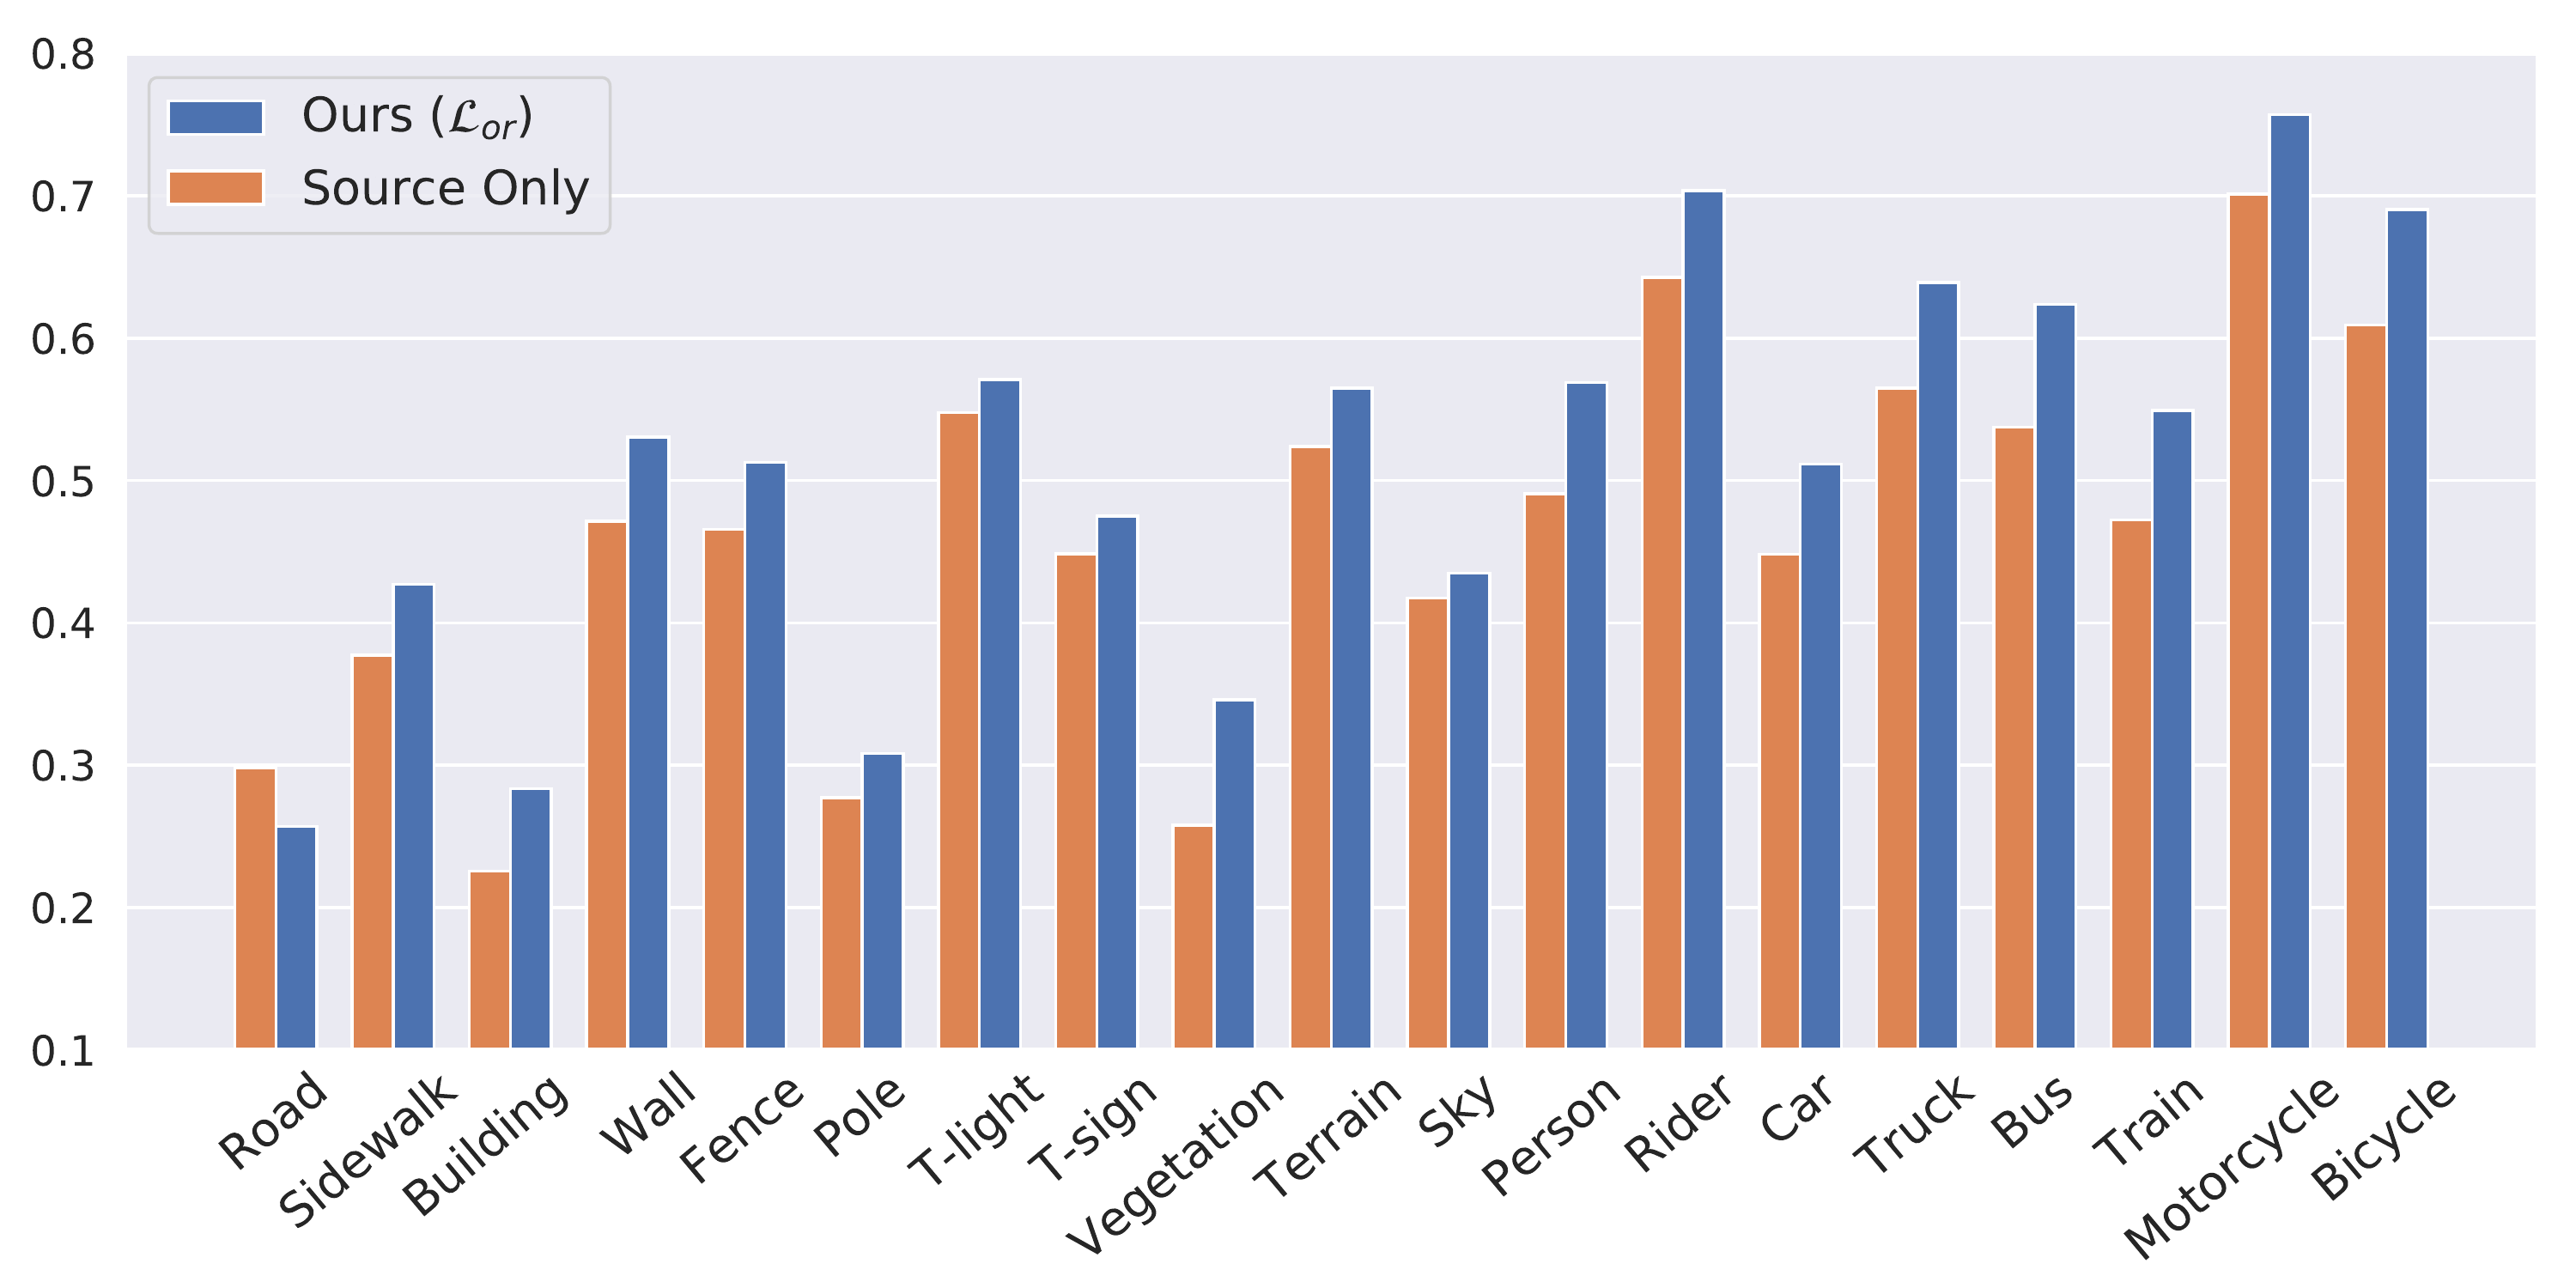}
\end{subfigure}
\\
\begin{subfigure}[t]{0.03\textwidth}
b)
\end{subfigure}
\begin{subfigure}[htbp]{0.7\textwidth}
\centering
\includegraphics[width=\linewidth]{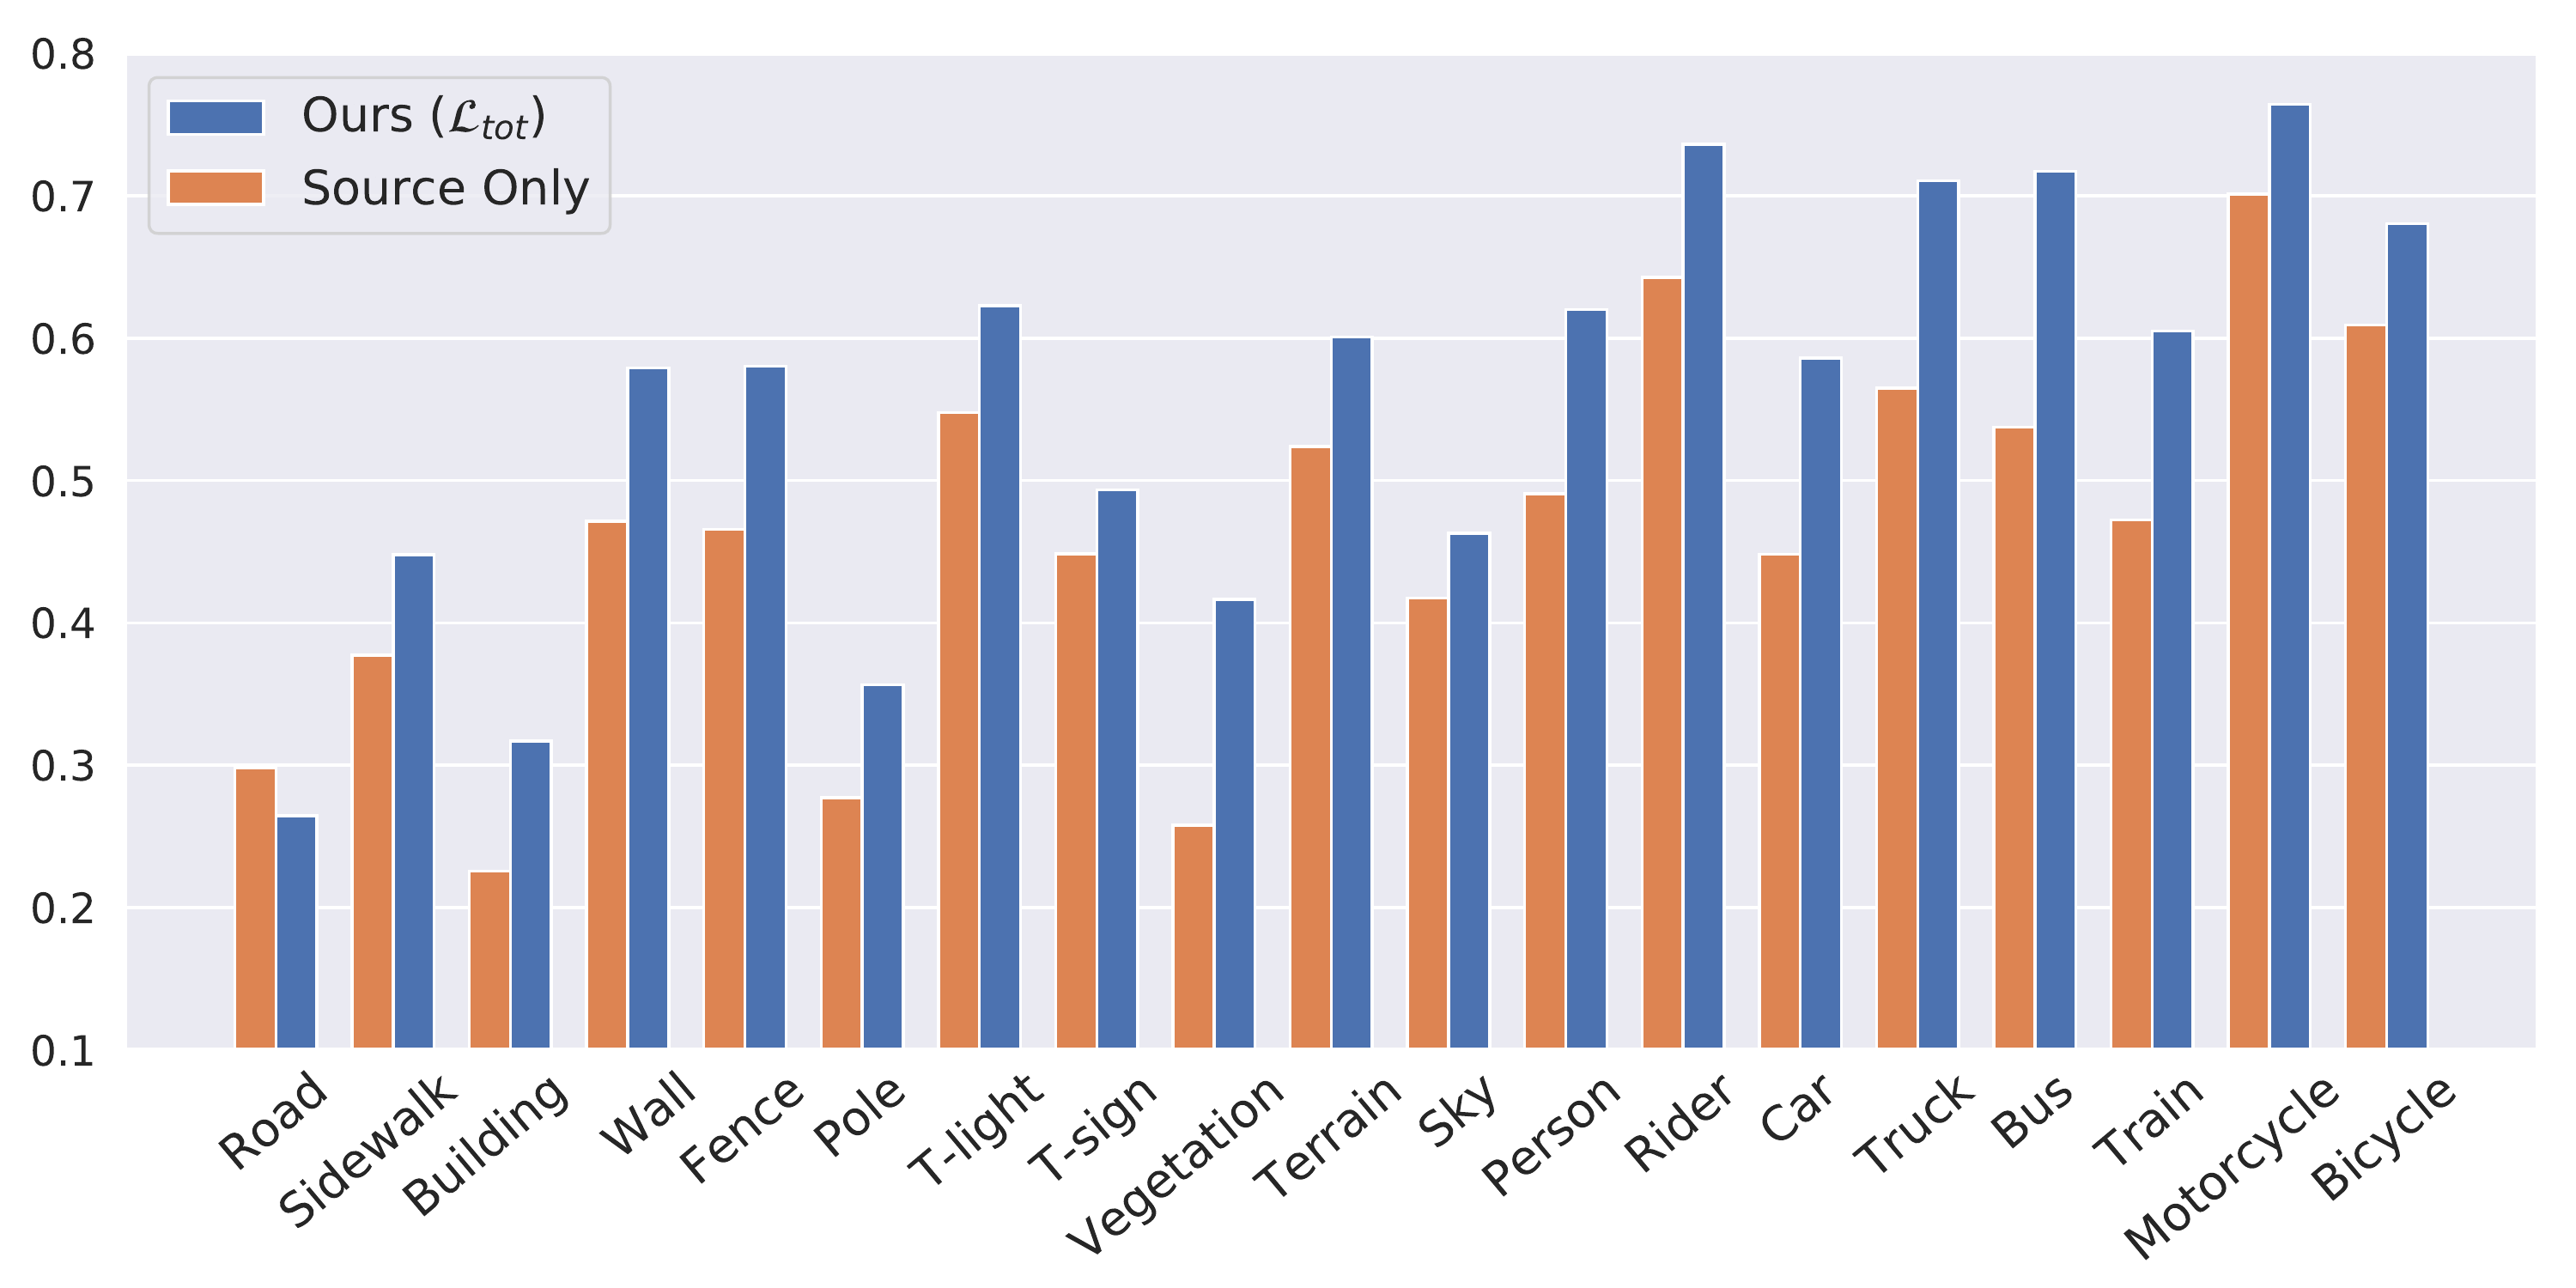}
\end{subfigure}
\\
\begin{subfigure}[t]{0.03\textwidth}
c)
\end{subfigure}
\begin{subfigure}[htbp]{0.7\textwidth}
\centering
\includegraphics[width=\linewidth]{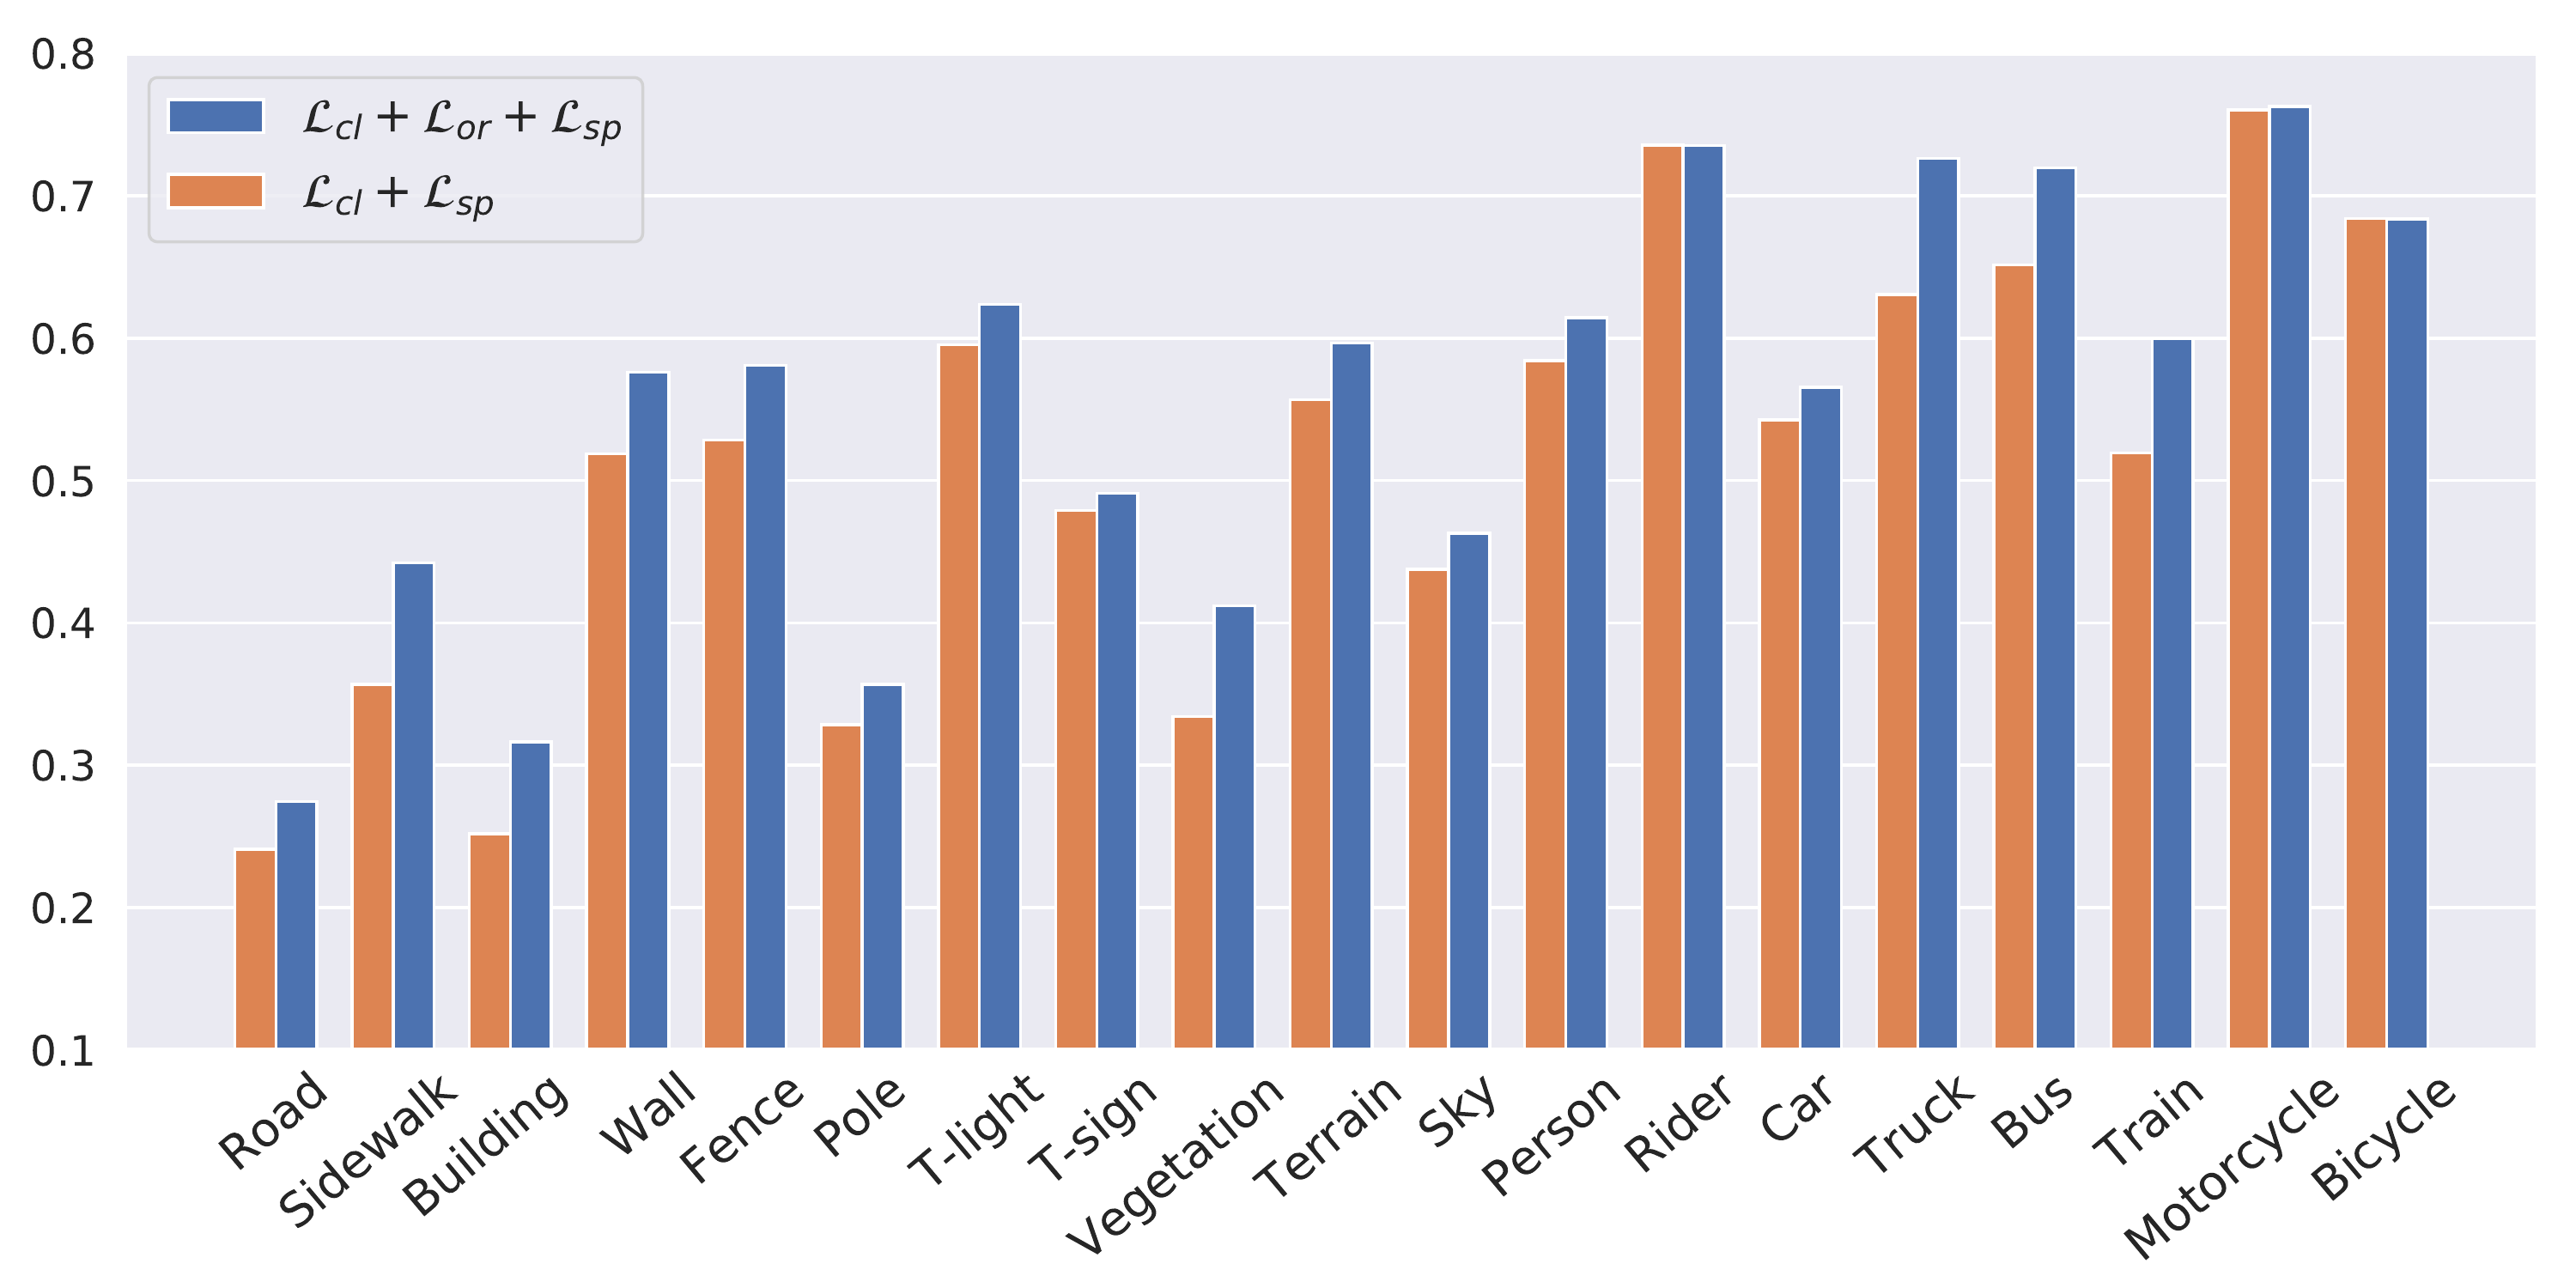}
\end{subfigure}
\caption{Similarity scores computed over all the images on the Cityscapes validation set when adapting from GTA5 to analyze the effect of the orthogonality constraint (\textit{best viewed in colors}).}
\label{fig:plot_similarity}
\end{figure*}
%
%
%
% ORTHOGONALITY MATRIX
\begin{figure*}[htbp]
\centering
\begin{subfigure}[htbp]{\textwidth}
\centering
\includegraphics[width=0.93\linewidth]{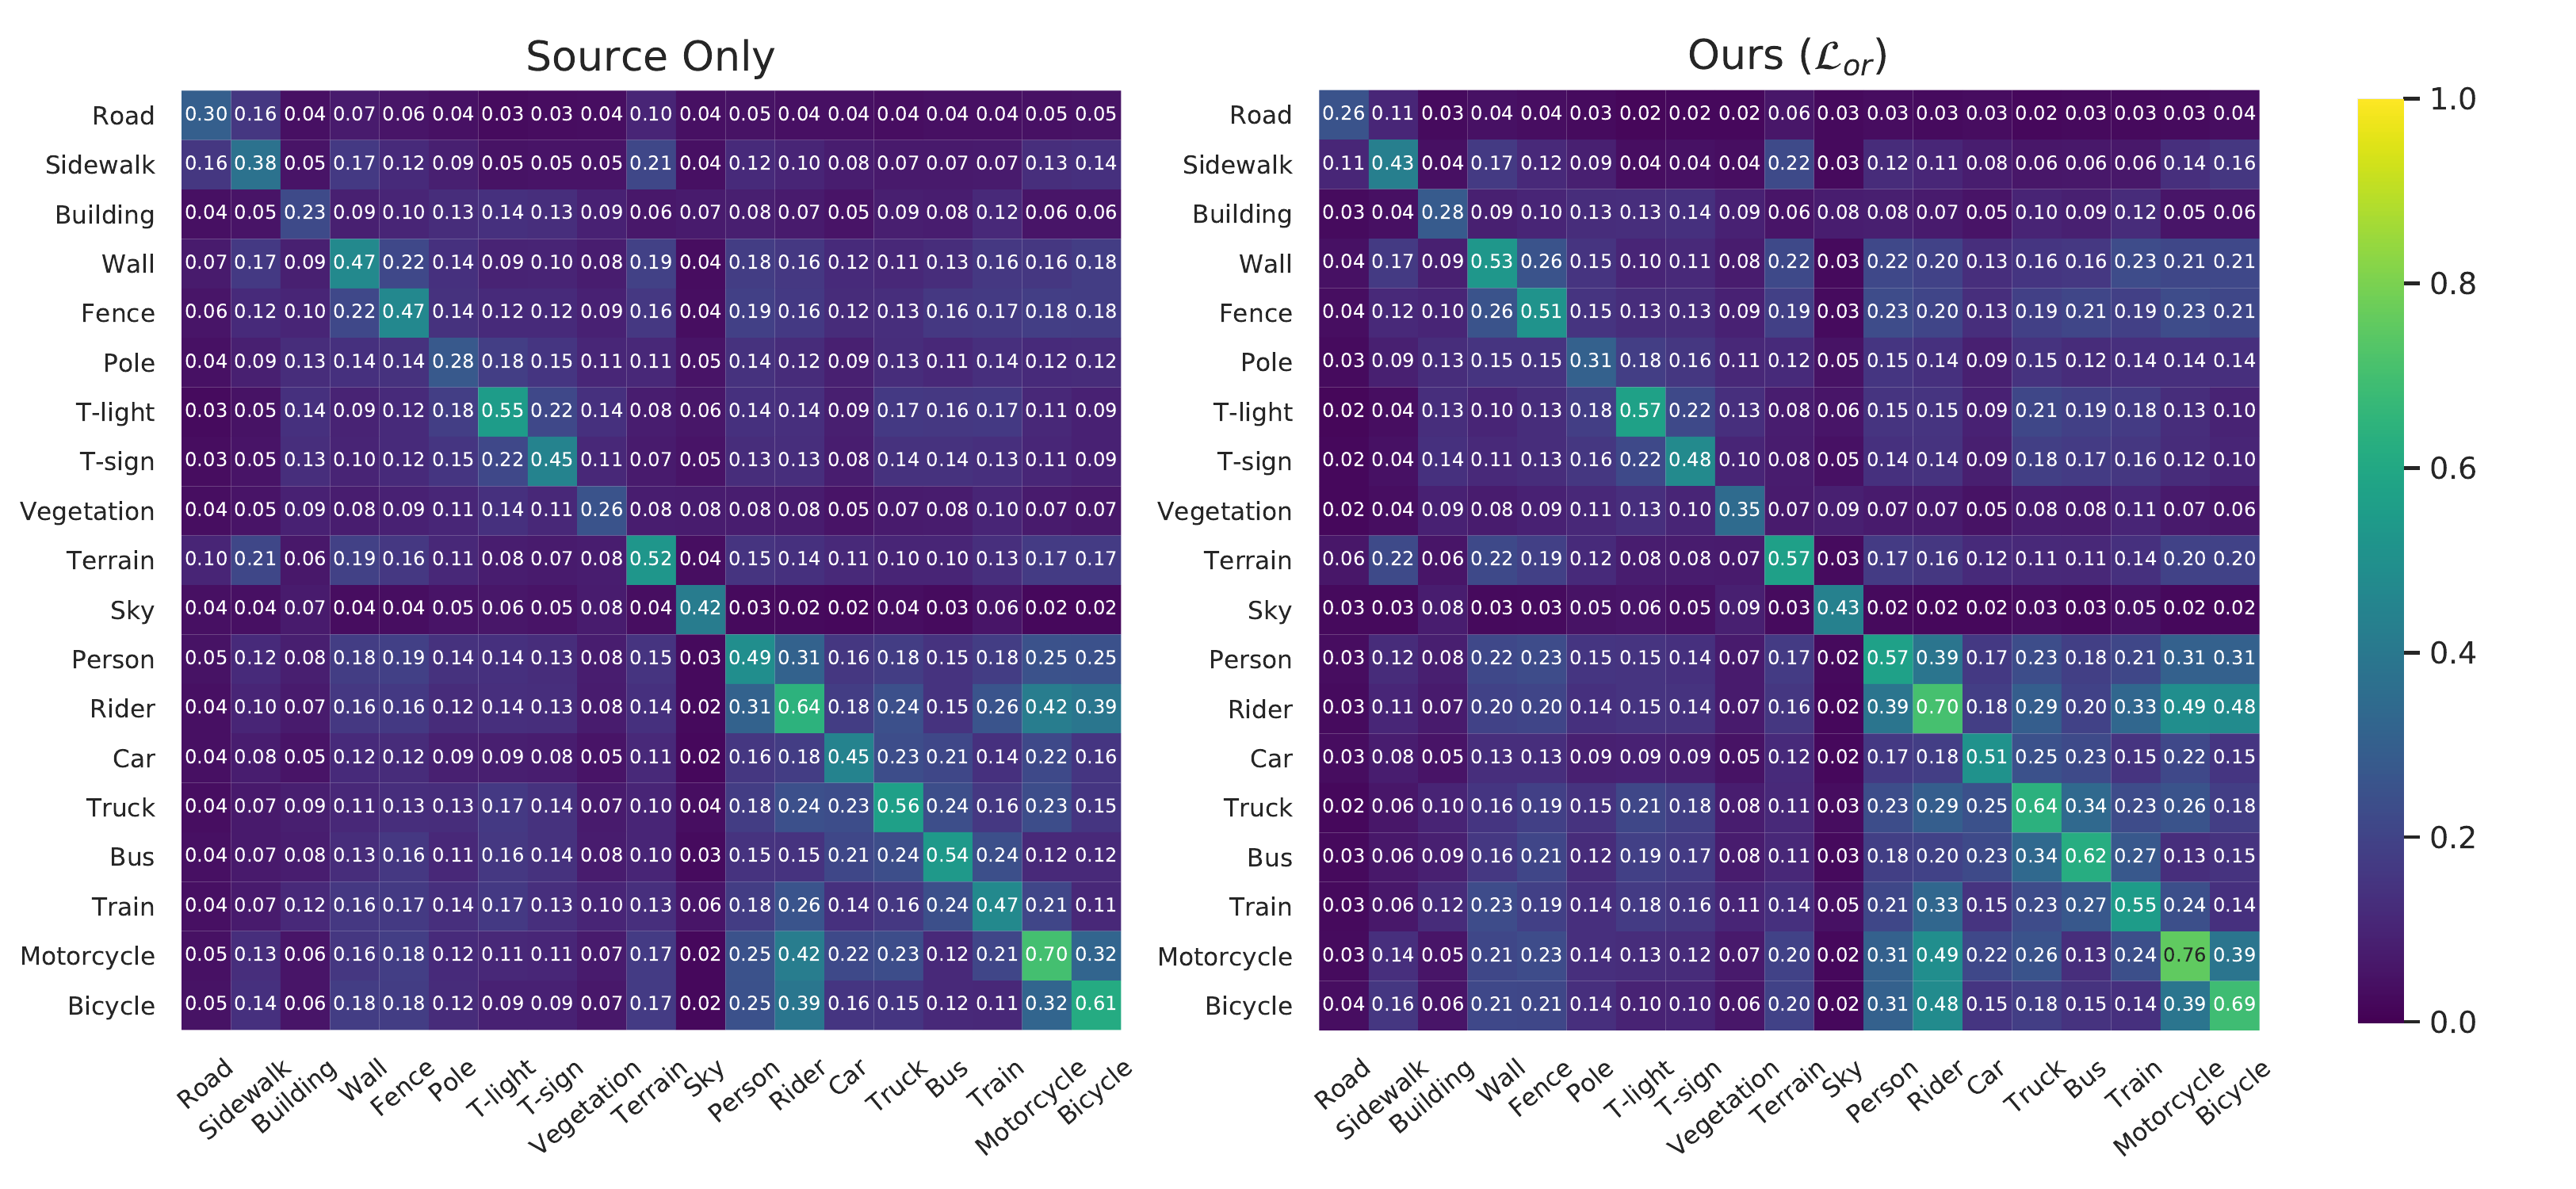}
\vspace{-0.5cm}
%\caption{}
%\label{fig:orthogonality_matrixa}
\end{subfigure}
\begin{subfigure}[htbp]{\textwidth}
\centering
\includegraphics[width=0.93\linewidth]{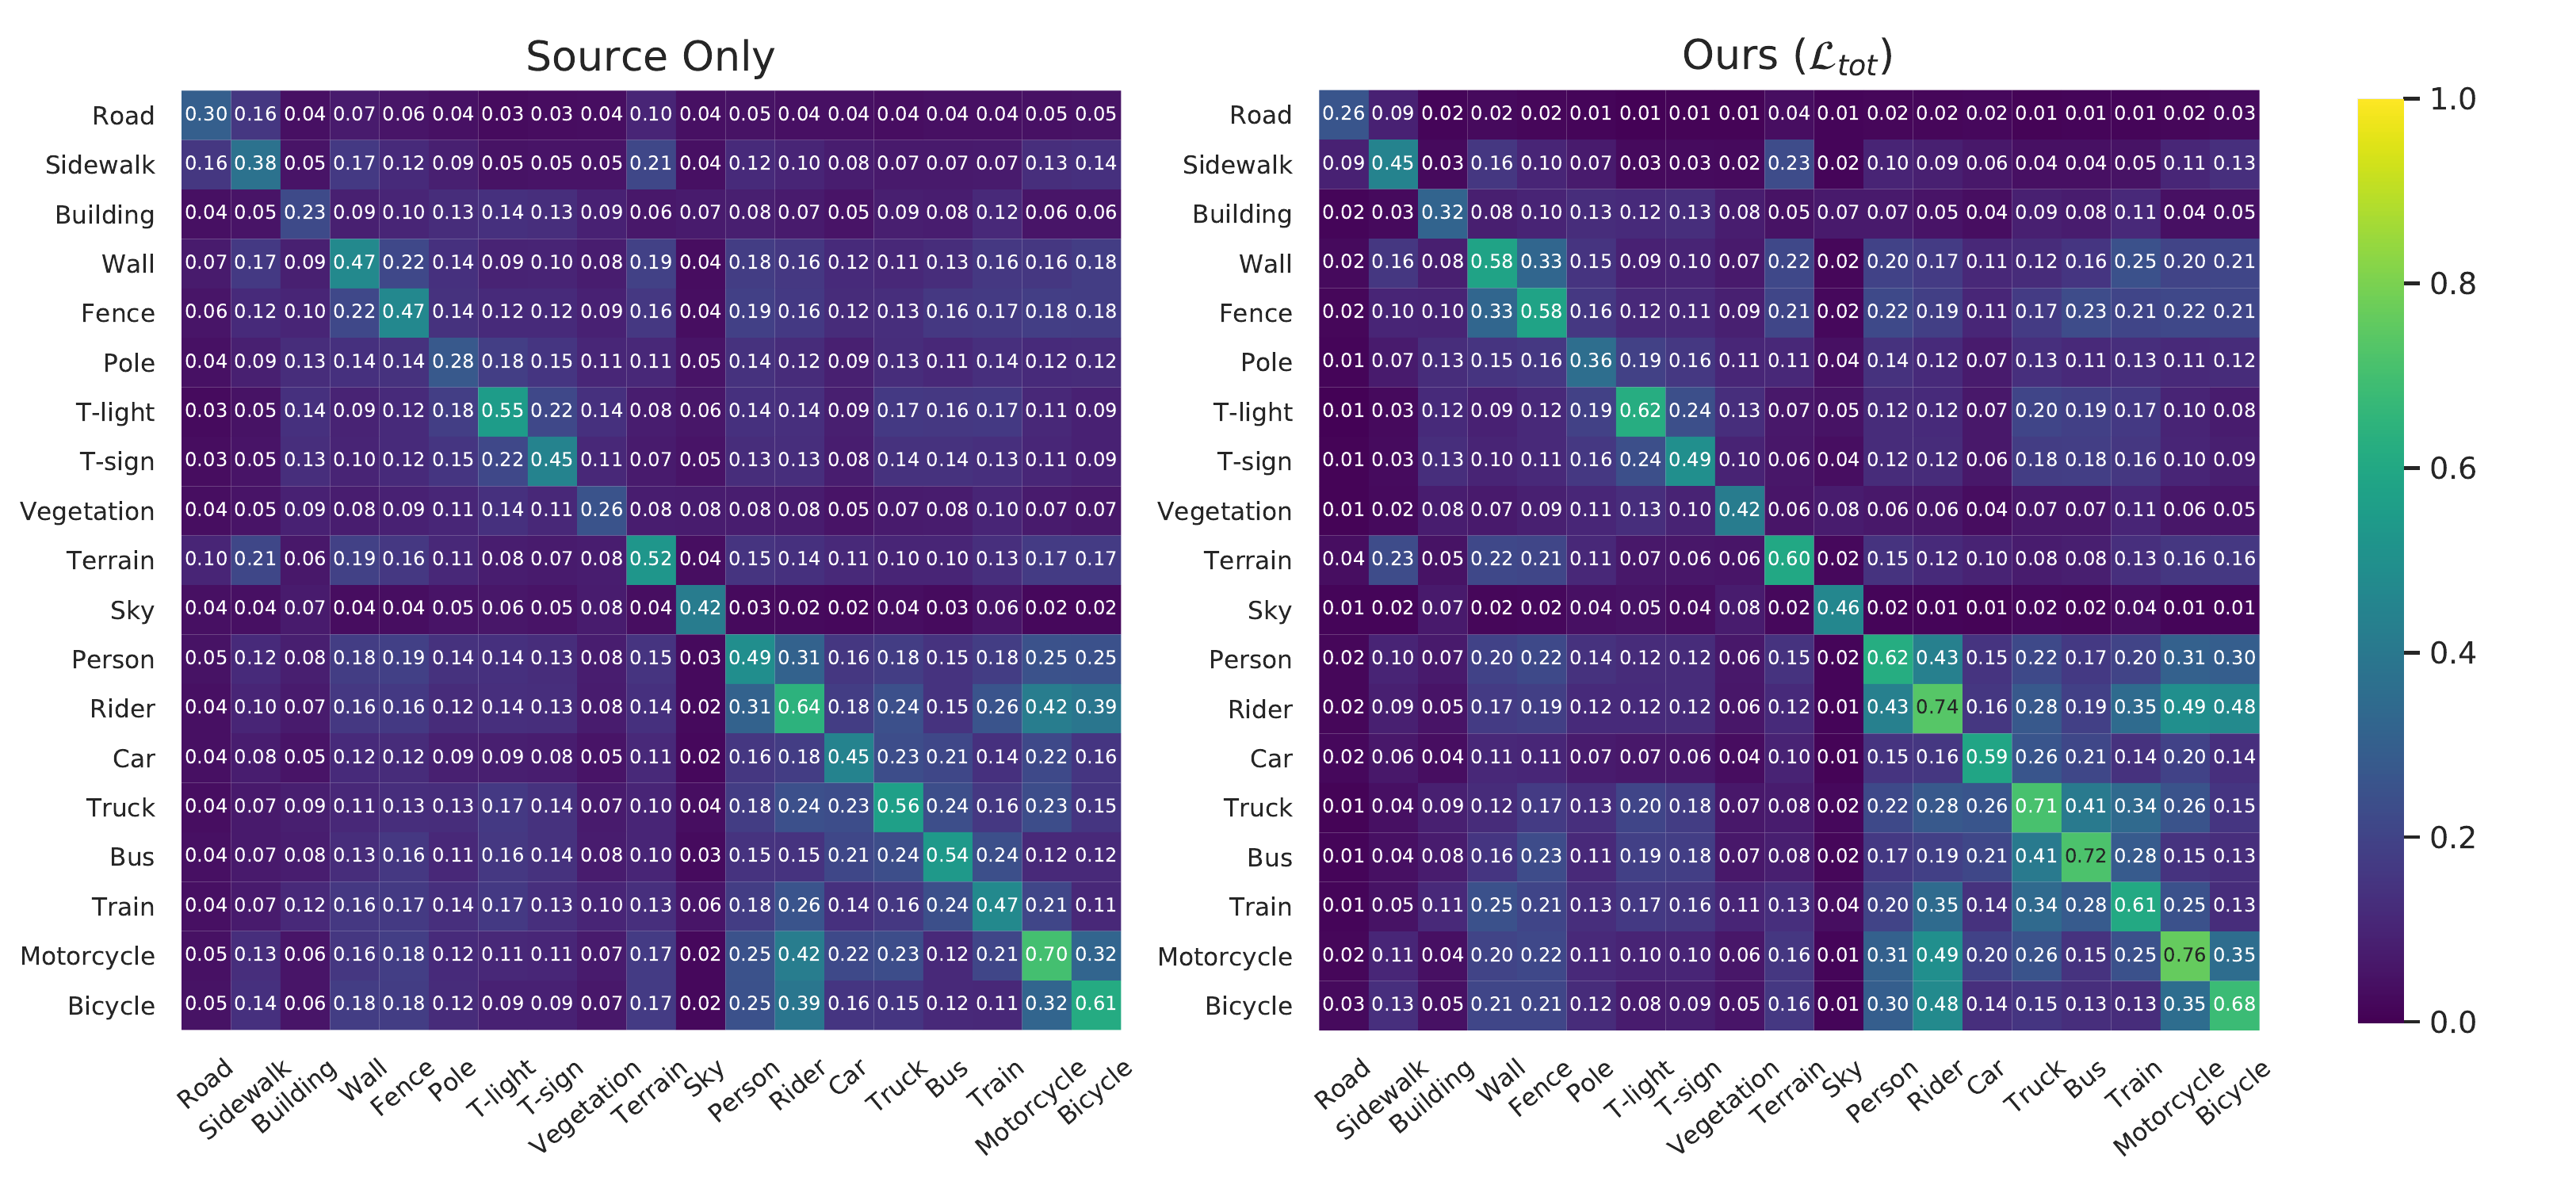}
\vspace{-0.5cm}
%\caption{}
%\label{fig:orthogonality_matrixb}
\end{subfigure}
\begin{subfigure}[htbp]{\textwidth}
\centering
\includegraphics[width=0.93\linewidth]{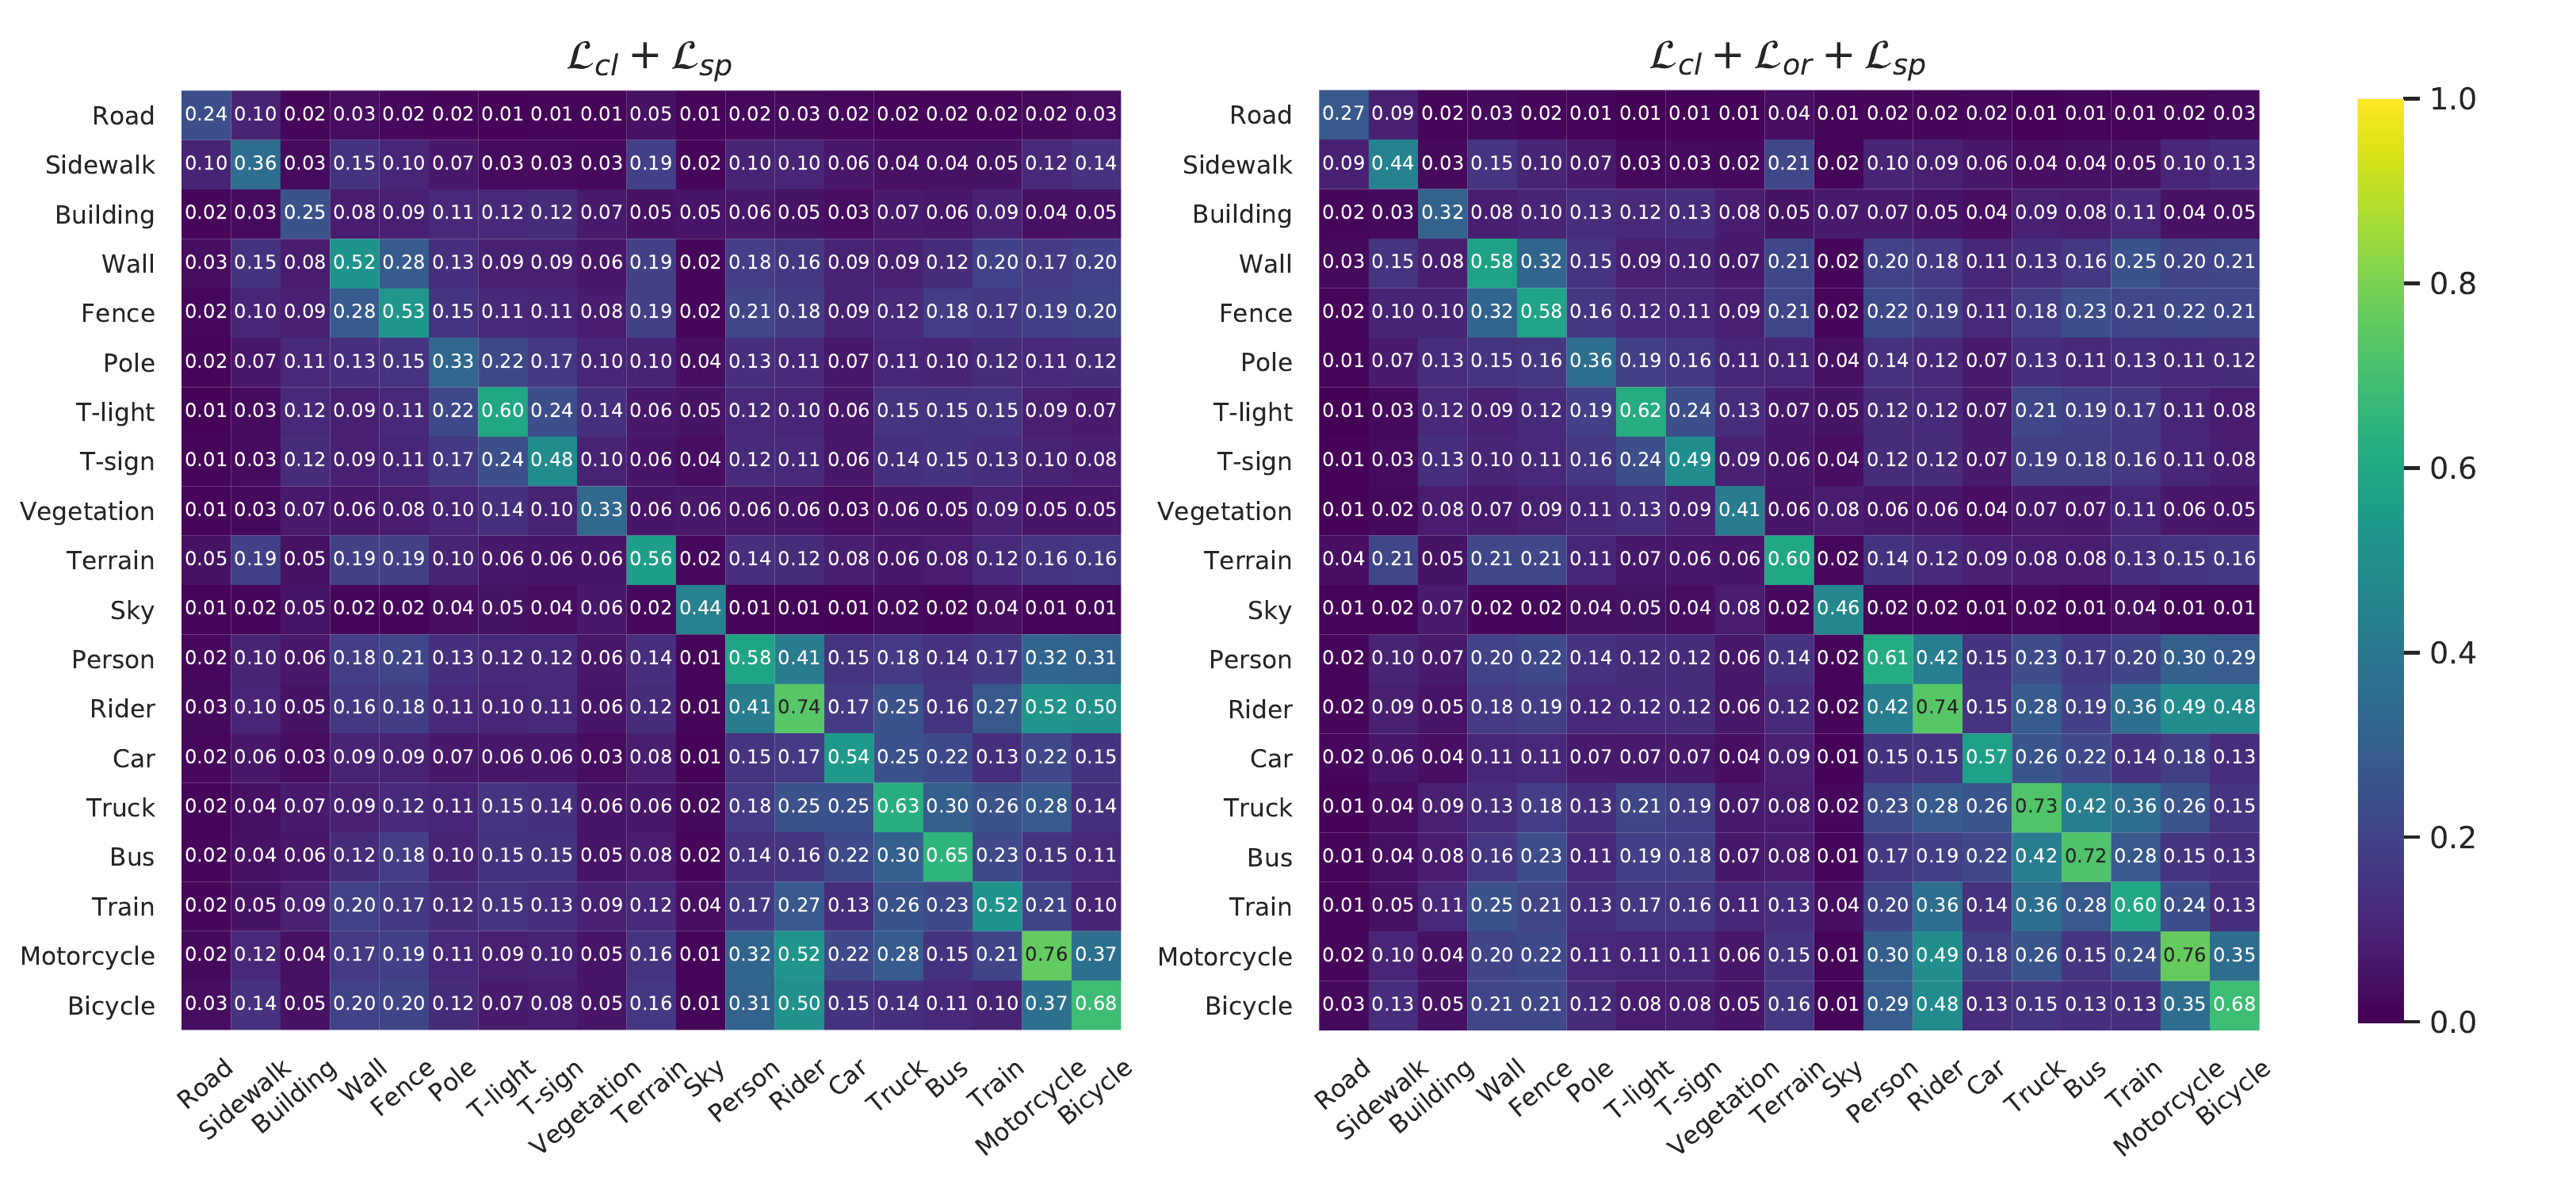}
%\vspace{-0.5cm}
%\caption{}
%\label{fig:orthogonality_matrixc}
\end{subfigure}
\vspace{-0.3cm}
\caption{Class-wise similarity scores computed over images on the Cityscapes validation set when adapting from GTA5 (\textit{best viewed in colors}).}
\label{fig:orthogonality_matrix}
\end{figure*}
%
%
% SPARSITY DENSITY HISTOGRAM
\begin{figure*}[htbp]
\centering
\includegraphics[width=0.9\linewidth]{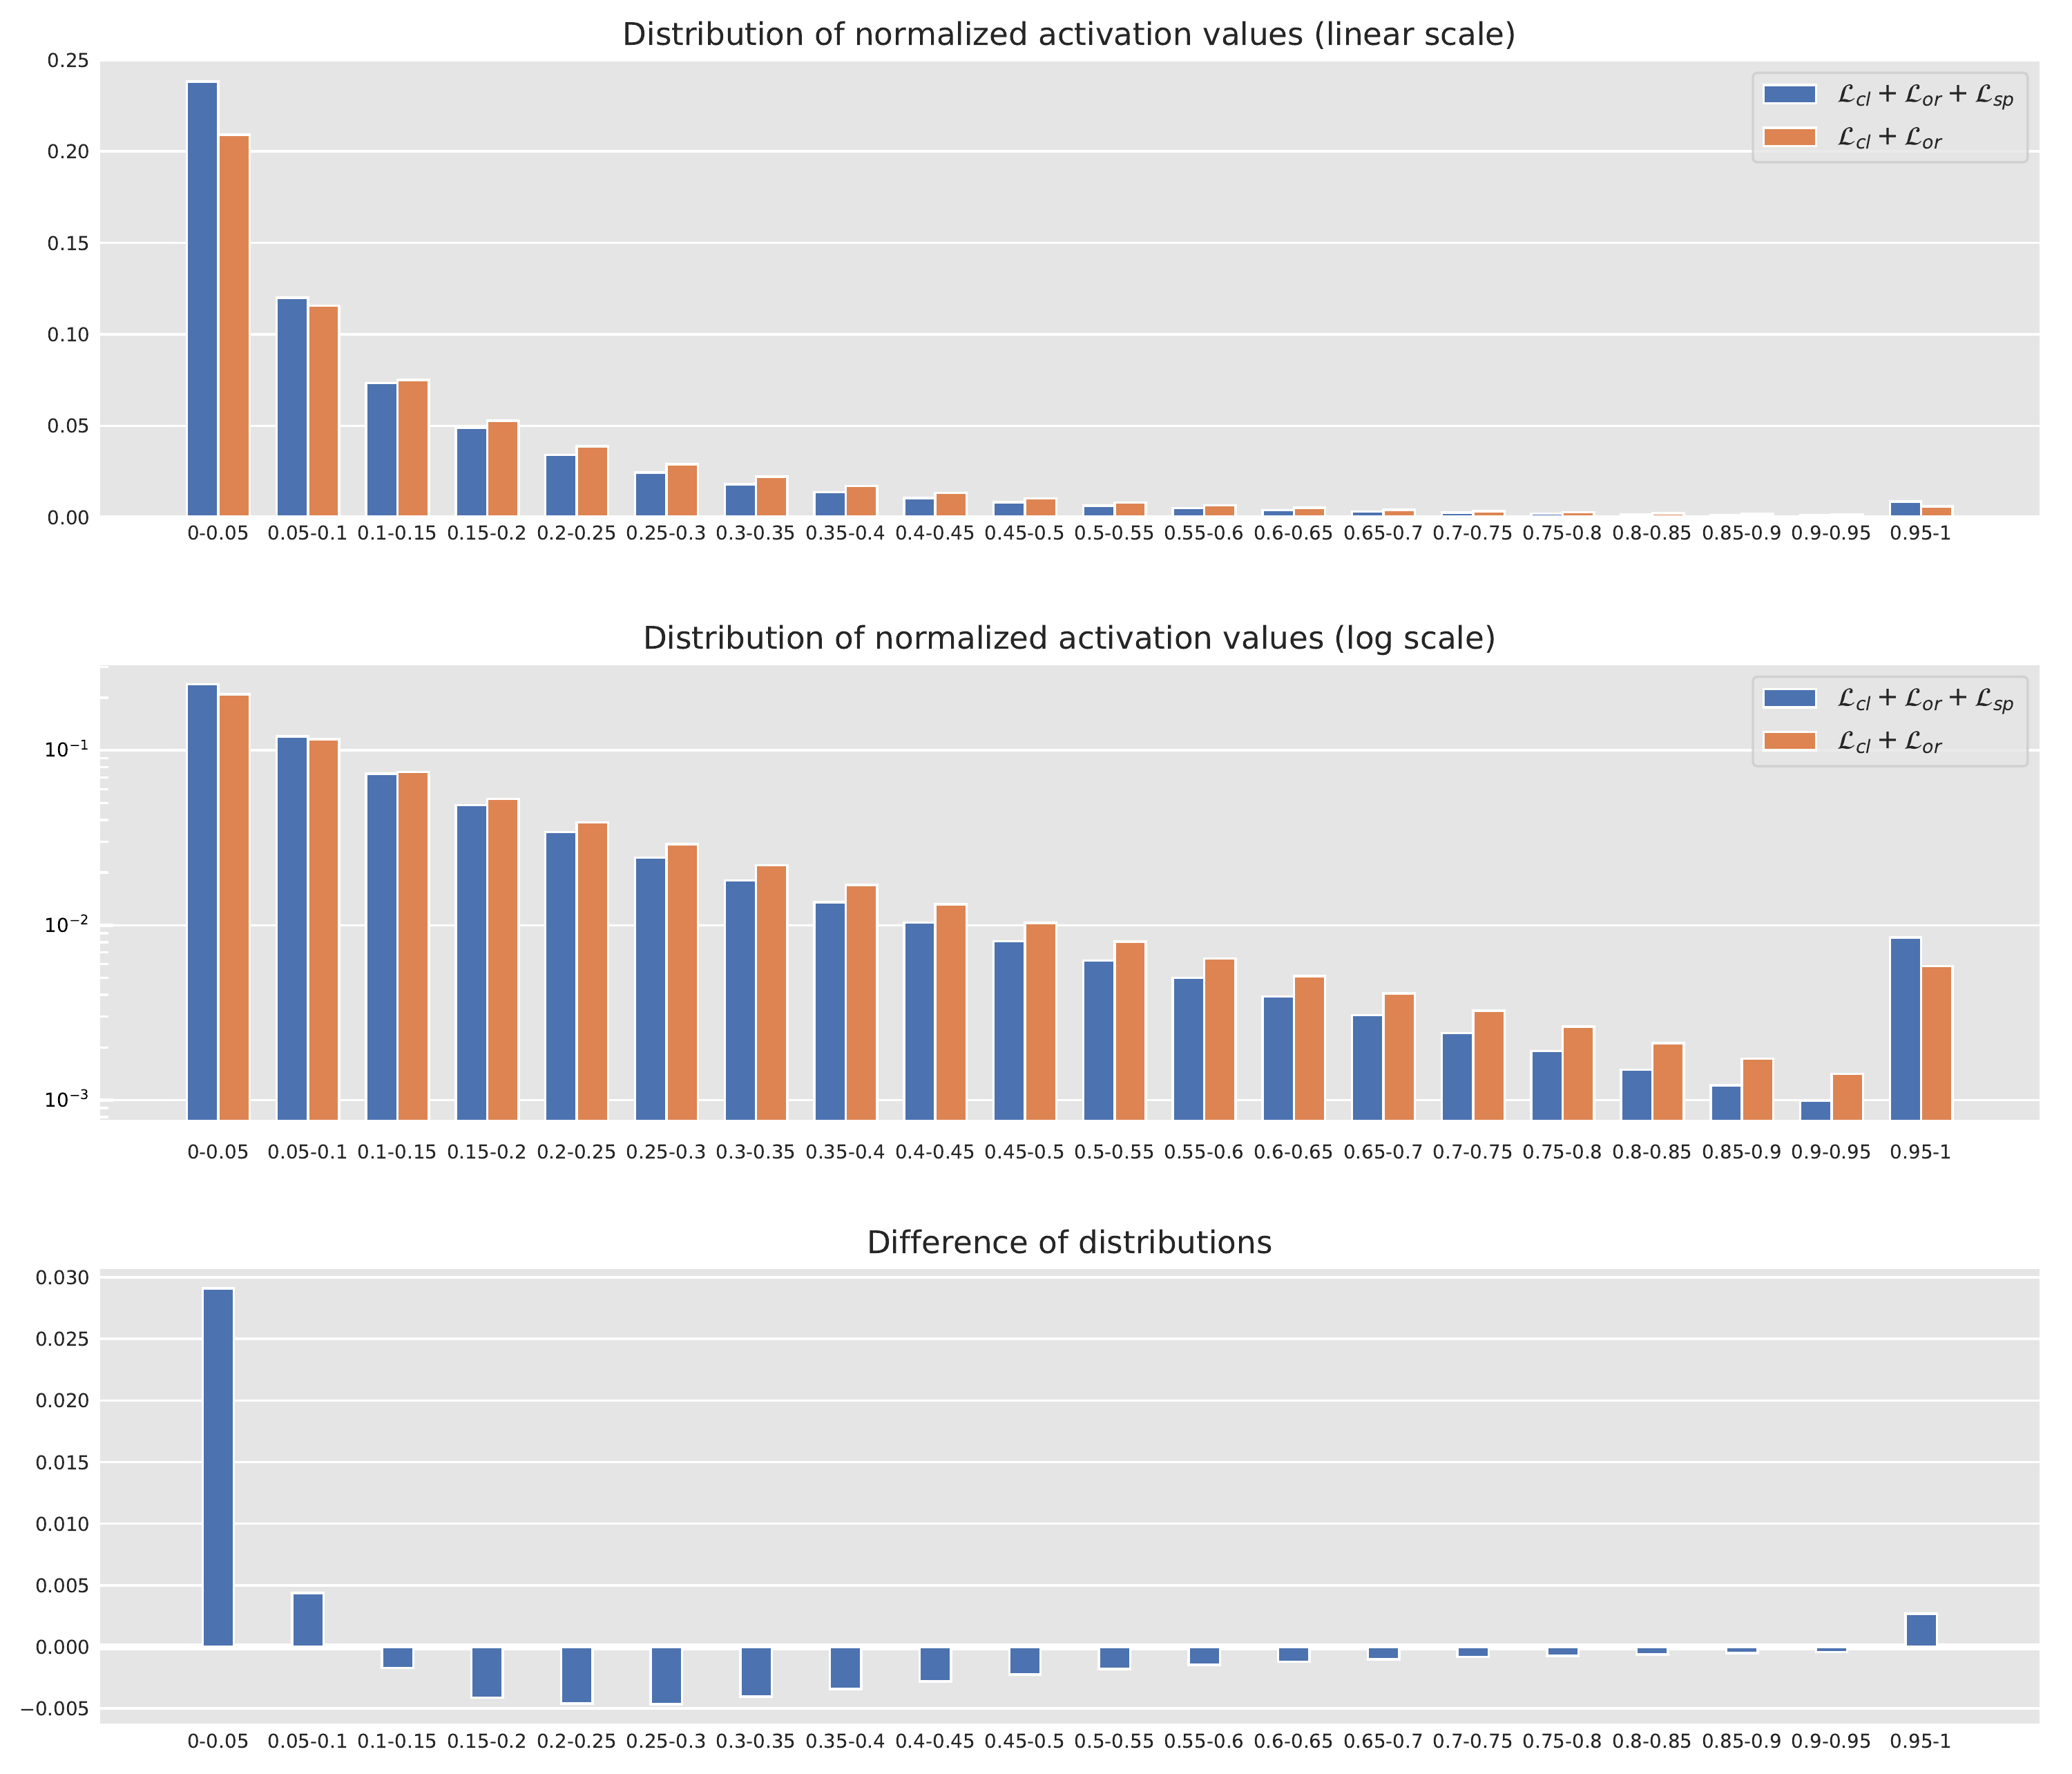}
%\caption{Average per-class confidence thresholds for different classes and at different training steps on the Mapillary dataset when adapting from GTA5 (\textit{best viewed in colors}).}
\caption{Analysis of the distribution of feature activations computed over all the images on the Cityscapes validation set when adapting from GTA5 (\textit{best viewed in colors}).}
\label{fig:plot_sparsity}
\end{figure*}

\subsection{Sparsity Loss}

%To investigate the contribution of the sparsity loss, $\mathcal{L}_{sp}$, we define a sparsity measure as the fraction of activations in normalized feature vectors close to $0$ or $1$. 
%Closeness is intended as being distant from $0$ or $1$ less than a threshold, which we set to $10^{-4}$. 
%As for the similarity scores, the sparsity measures for a single target image are obtained through averaging over all feature vectors from the same class. 

To further investigate the contribution of the sparsity loss, $\mathcal{L}_{sp}$, we inspect how values of feature channels (i.e.\ single units in feature vectors) end up being %are 
distributed for different adaptation settings.  
In Figure~\ref{fig:plot_sparsity} we plot the histogram distribution of all normalized feature activations with bin size set to $0.05$ in linear scale and in log scale. Here, we can observe that adding $\mathcal{L}_{sp}$ leads to a greater number of occurrences of activations within $0$ and $0.1$ and within $0.95$ and $1$ than in the case without sparsity constraint. In the middle, instead, the opposite is true. We refer the reader to Eq. 7 of the main paper to certify that this is indeed what the sparsity loss was aiming to achieve. Namely, the sparsity constraint reduces class-wise the number of active feature channels pushing them either toward $0$ (inactive features) or towards $1$ (active features).

Ultimately, for more immediate visualization, we plot in the third image of Figure~\ref{fig:plot_sparsity} the difference of the sparsity distributions with and without $\mathcal{L}_{sp}$. We can more easily verify that extremely low (in closest range to $0$) and extremely high (in closest range to $1$) bins have positive values while middle-range bins have negative values.
