# Supplementary material for: Unsupervised Domain Adaptation in Semantic Segmentation via Orthogonal and Clustered Embeddings
Source: arXiv:2011.12616 source file (2020-11-25)
Supplement: Supplementary file 2 [file mosaic_supp.tex]

\newcommand{\imgsize}{27.58mm}
\begin{figure*}[h!]
\centering
\begin{subfigure}[htbp]{\textwidth}

%\hspace{0.22cm}
\centering
\resizebox{\textwidth}{!}{%
\hspace{0.6cm}
\begin{tabular}{cccccccccc}
\cellcolor[HTML]{804080}{\color[HTML]{FFFFFF} \textbf{road}} & \cellcolor[HTML]{F423E8}\textbf{sidewalk} & \cellcolor[HTML]{464646}{\color[HTML]{FFFFFF} \textbf{building}} & \cellcolor[HTML]{66669C}{\color[HTML]{FFFFFF} \textbf{wall}} & \cellcolor[HTML]{BE9999}\textbf{fence} & \cellcolor[HTML]{999999}\textbf{pole} & \cellcolor[HTML]{FAAA1E}\textbf{traffic light} & \cellcolor[HTML]{DCDC00}\textbf{traffic sign} &\cellcolor[HTML]{6B8E23} \textbf{vegetation} & \cellcolor[HTML]{98FB98}\textbf{terrain} \\ %\cline{10-10} 
\cellcolor[HTML]{4682B4}\textbf{sky} & \cellcolor[HTML]{DC143C}{\color[HTML]{FFFFFF} \textbf{person}} & \cellcolor[HTML]{FF0000}{\color[HTML]{FFFFFF} \textbf{rider}} & \cellcolor[HTML]{00008E}{\color[HTML]{FFFFFF} \textbf{car}} & \cellcolor[HTML]{000046}{\color[HTML]{FFFFFF} \textbf{truck}} & \cellcolor[HTML]{003C64}{\color[HTML]{FFFFFF} \textbf{bus}} & \cellcolor[HTML]{005064}{\color[HTML]{FFFFFF} \textbf{train}} & \cellcolor[HTML]{0000E6}{\color[HTML]{FFFFFF} \textbf{motorcycle}} & \cellcolor[HTML]{770B20}{\color[HTML]{FFFFFF} \textbf{bicycle}} & \cellcolor[HTML]{000000}{\color[HTML]{FFFFFF} \textbf{unlabeled}} \\ 
%& \multicolumn{1}{c|}{\cellcolor[HTML]{770B20}{\color[HTML]{FFFFFF} \textbf{bicycle}}} & \multicolumn{1}{c|}{\textbf{unlabeled}} \\ \cline{10-10} 
\end{tabular}%
}

\vspace{0.1cm}
\end{subfigure}
\setlength{\tabcolsep}{0.7pt} % Default value: 6pt

\centering
\begin{subfigure}[htbp]{2\textwidth}
\begin{tabular}{c @{\hspace{1mm}} | @{\hspace{1.5mm}} cccccc}
  
   \multirow{8}{*}{\rotatebox{90}{GTA5 $\rightarrow$ Cityscapes}} &
   \includegraphics[width=\imgsize]{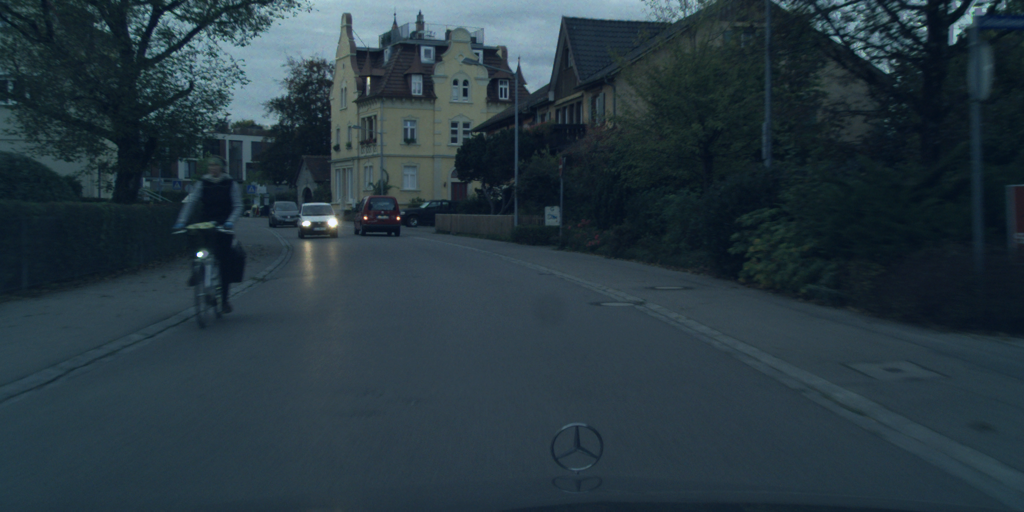} &
   \includegraphics[width=\imgsize]{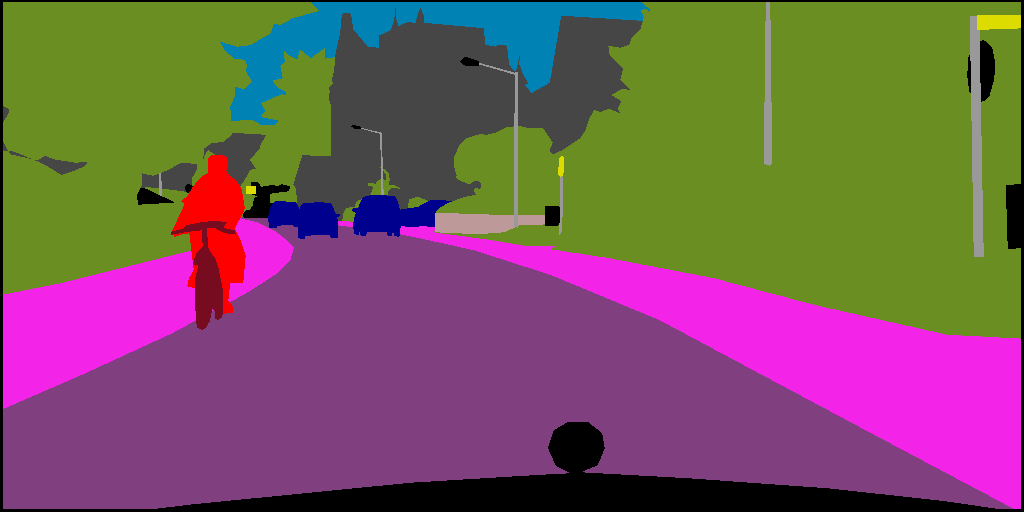} & 
   \includegraphics[width=\imgsize]{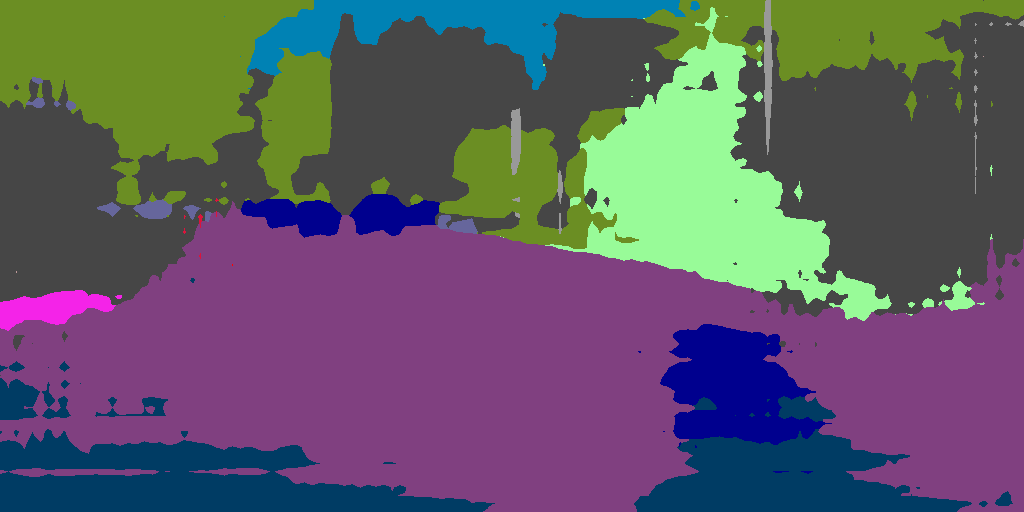} & 
   \includegraphics[width=\imgsize]{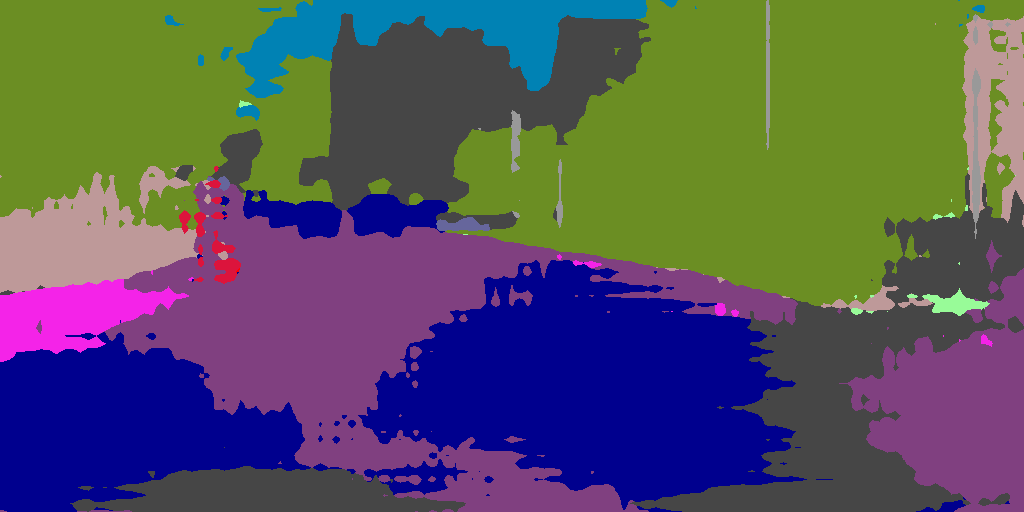} & 
   \includegraphics[width=\imgsize]{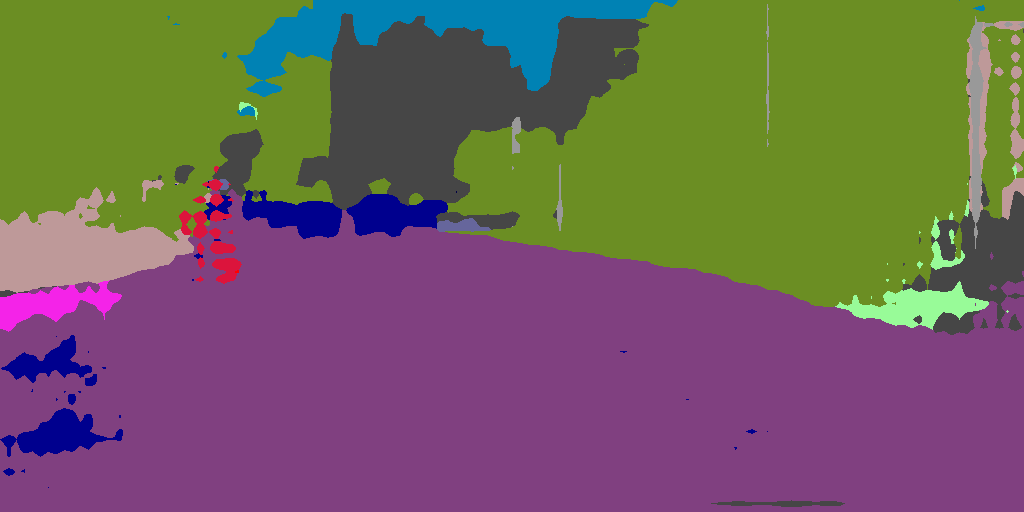} &
   \includegraphics[width=\imgsize]{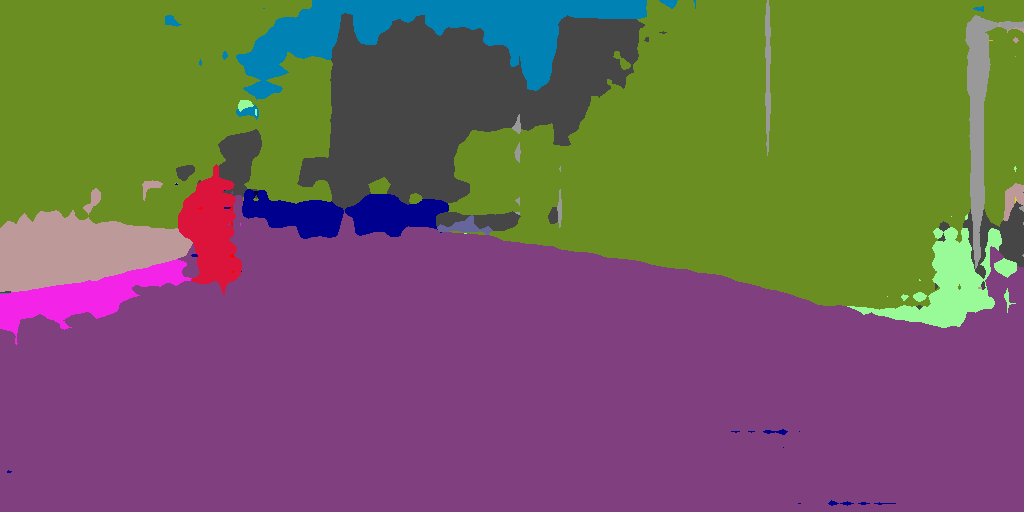} \\ 
   
   &
   \includegraphics[width=\imgsize]{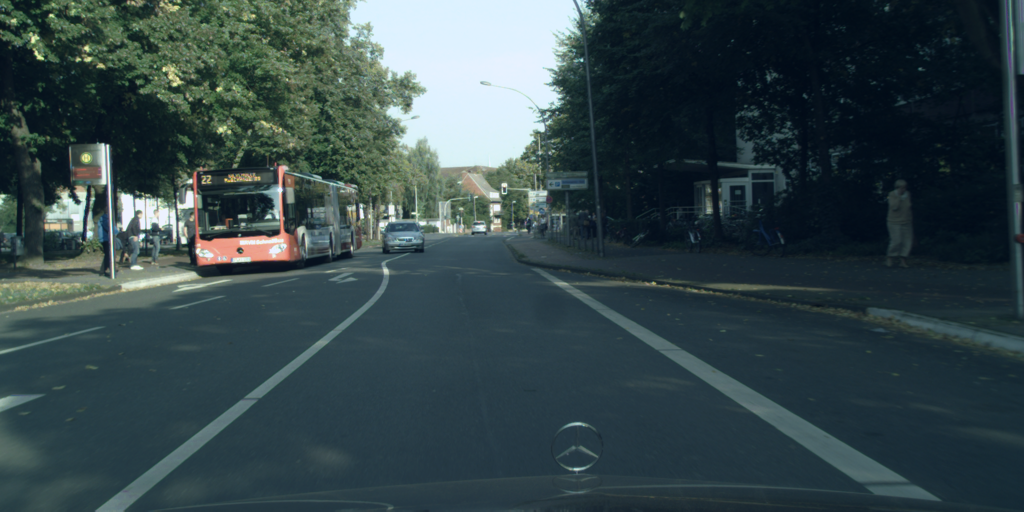} &
   \includegraphics[width=\imgsize]{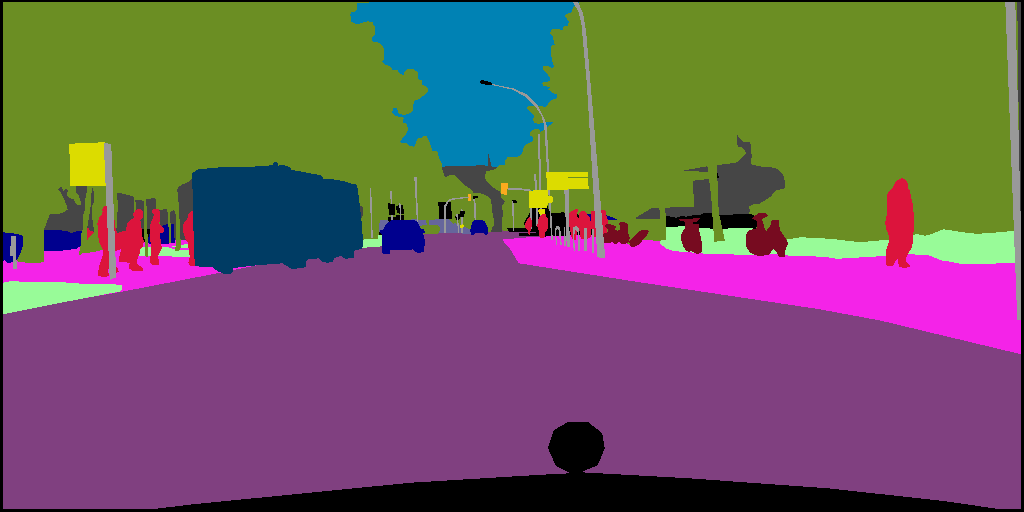} & 
   \includegraphics[width=\imgsize]{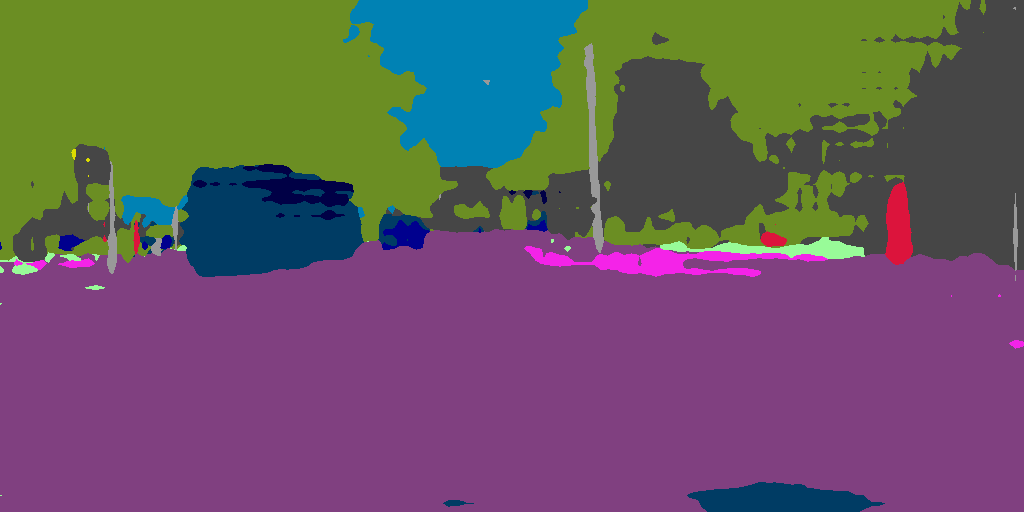} & 
   \includegraphics[width=\imgsize]{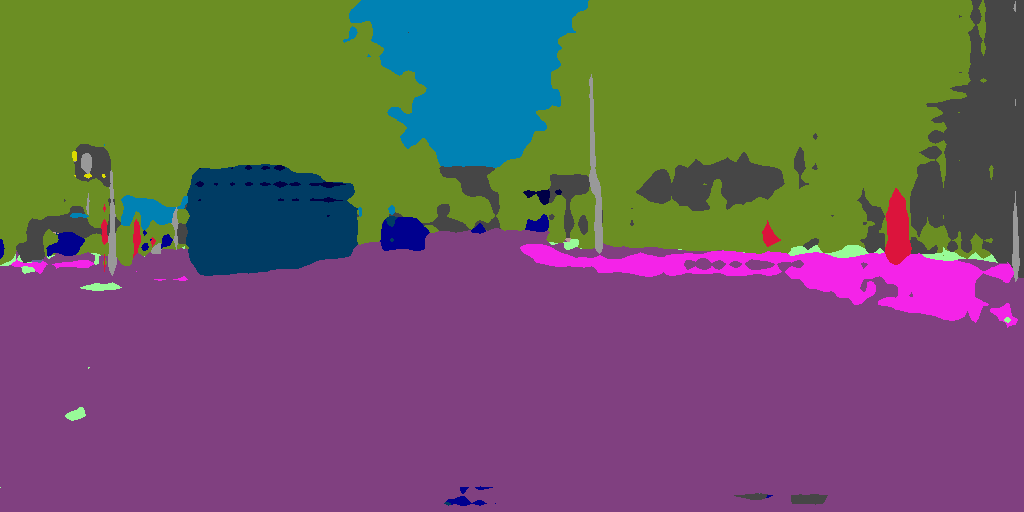} & 
   \includegraphics[width=\imgsize]{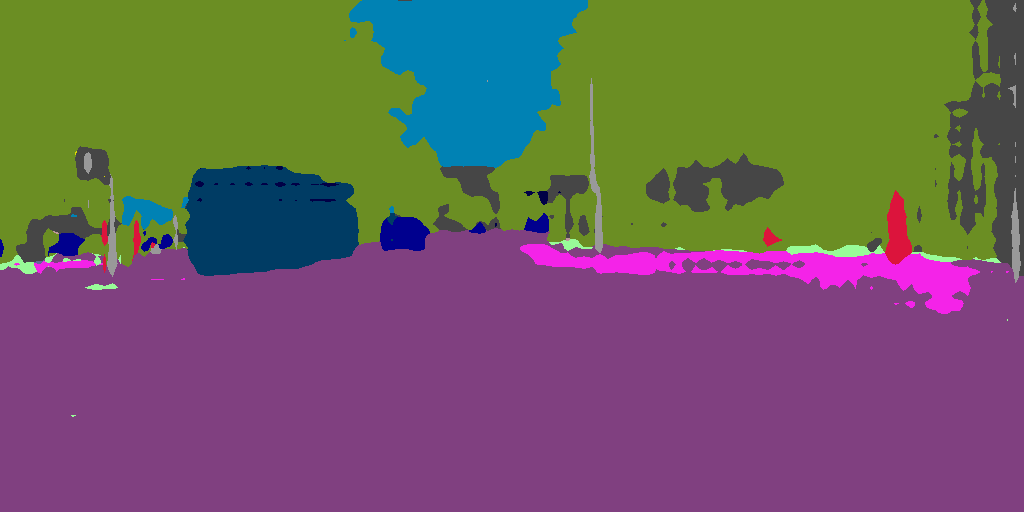} &
   \includegraphics[width=\imgsize]{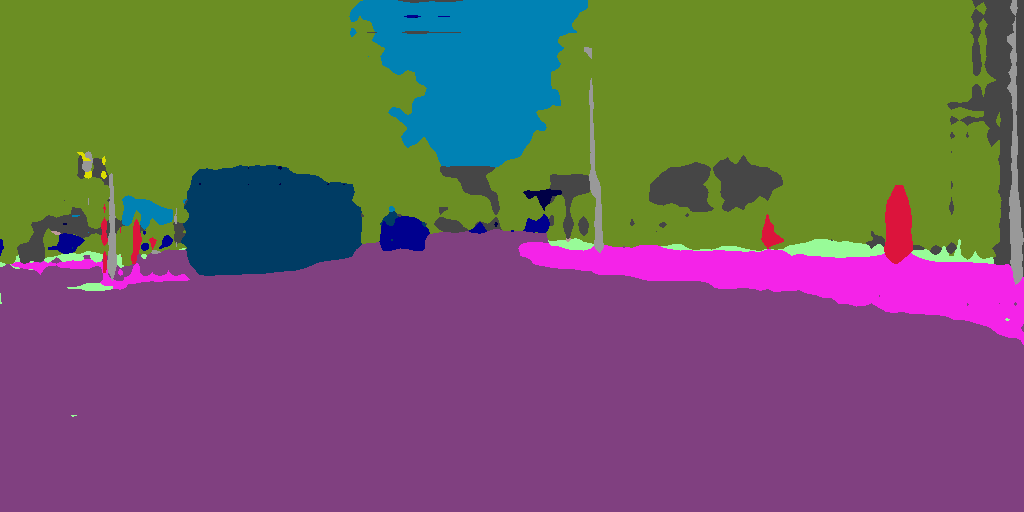} \\    
   
   &
   \includegraphics[width=\imgsize]{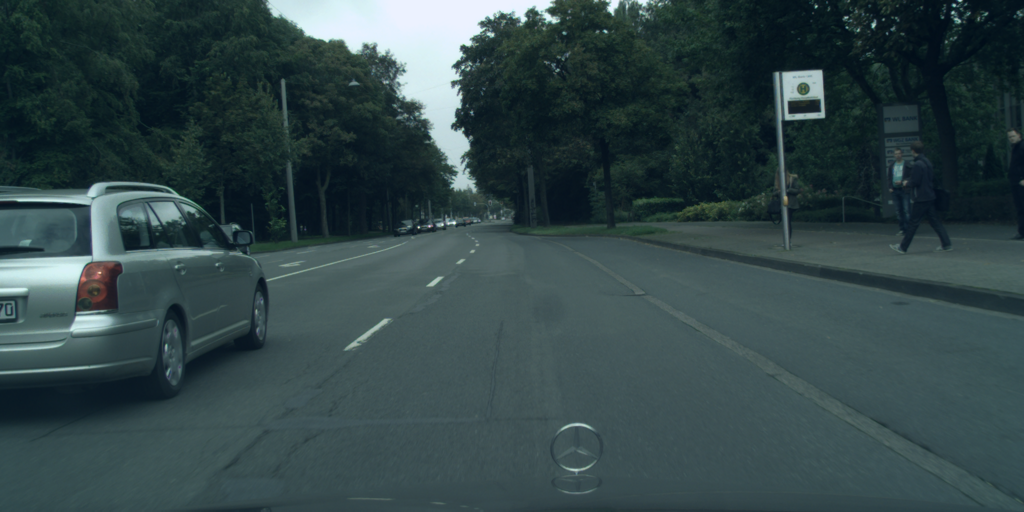} &
   \includegraphics[width=\imgsize]{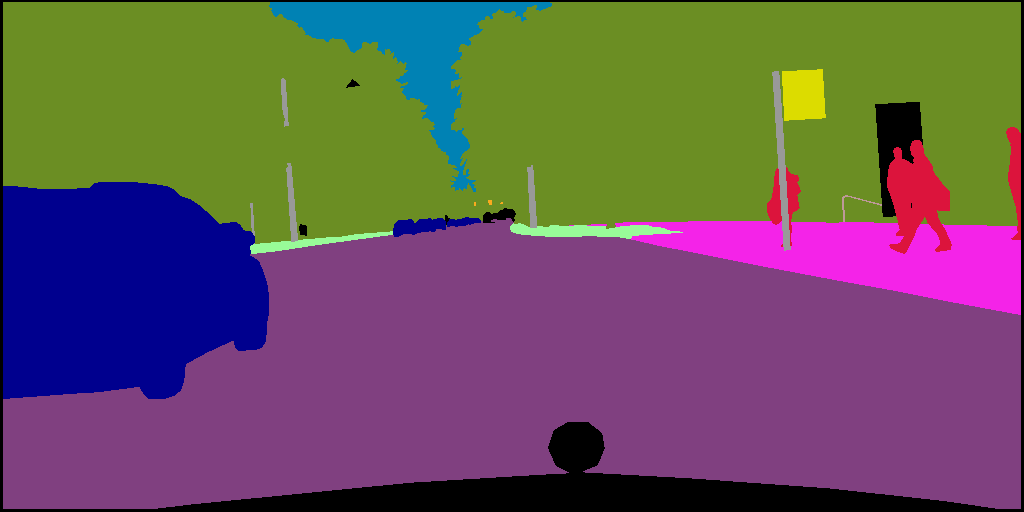} & 
   \includegraphics[width=\imgsize]{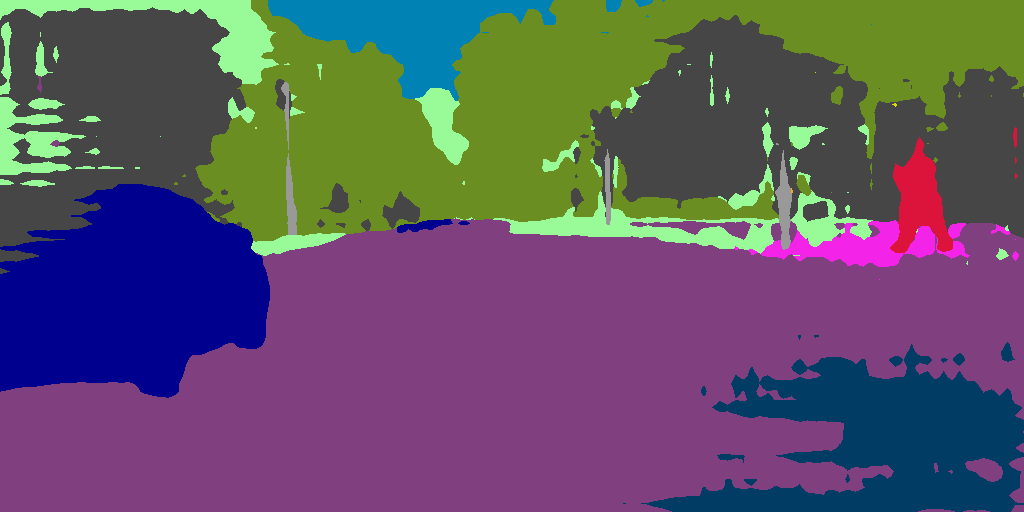} & 
   \includegraphics[width=\imgsize]{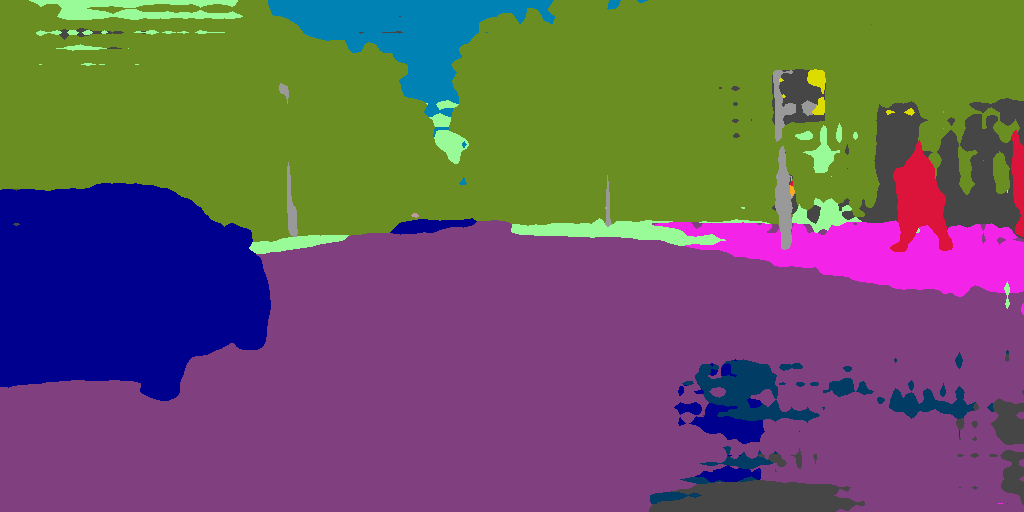} & 
   \includegraphics[width=\imgsize]{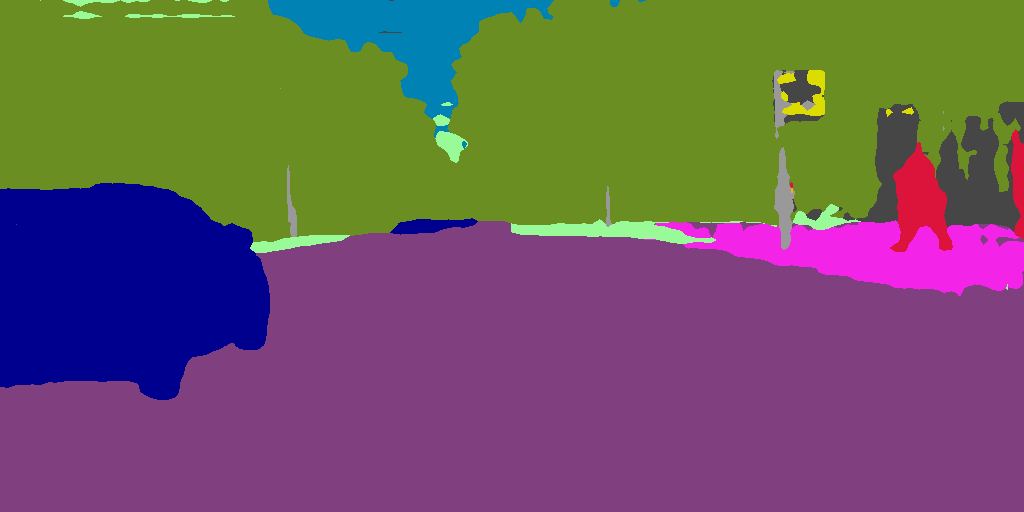} &
   \includegraphics[width=\imgsize]{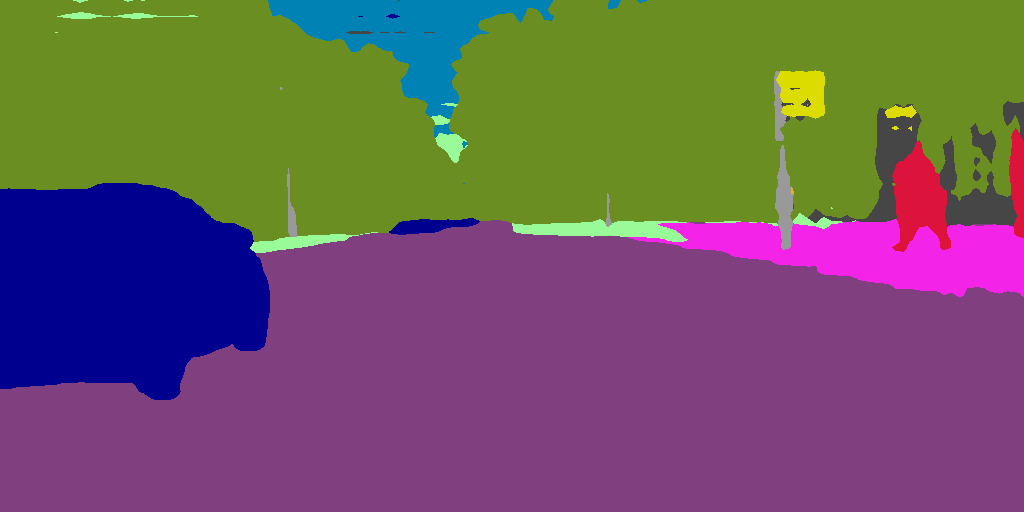} \\
   
   &
   \includegraphics[width=\imgsize]{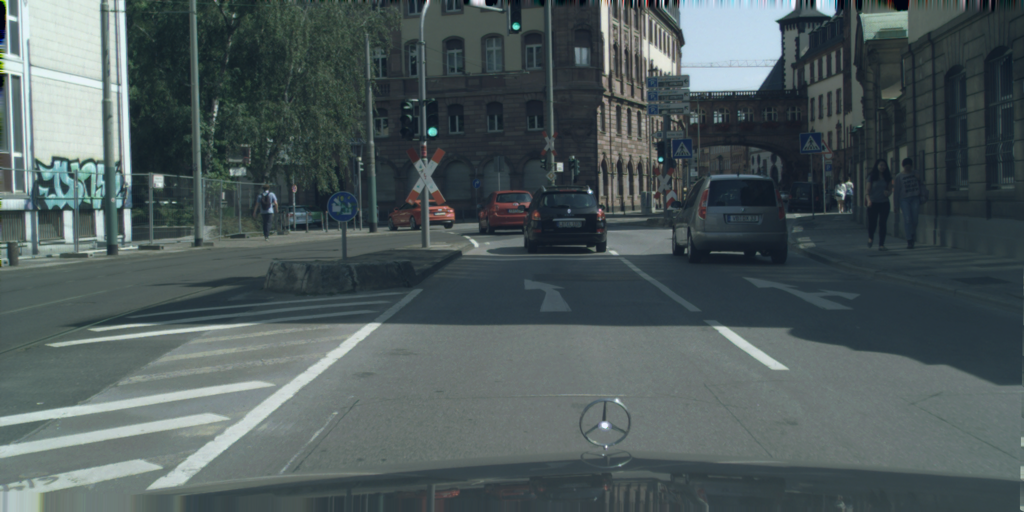} &
   \includegraphics[width=\imgsize]{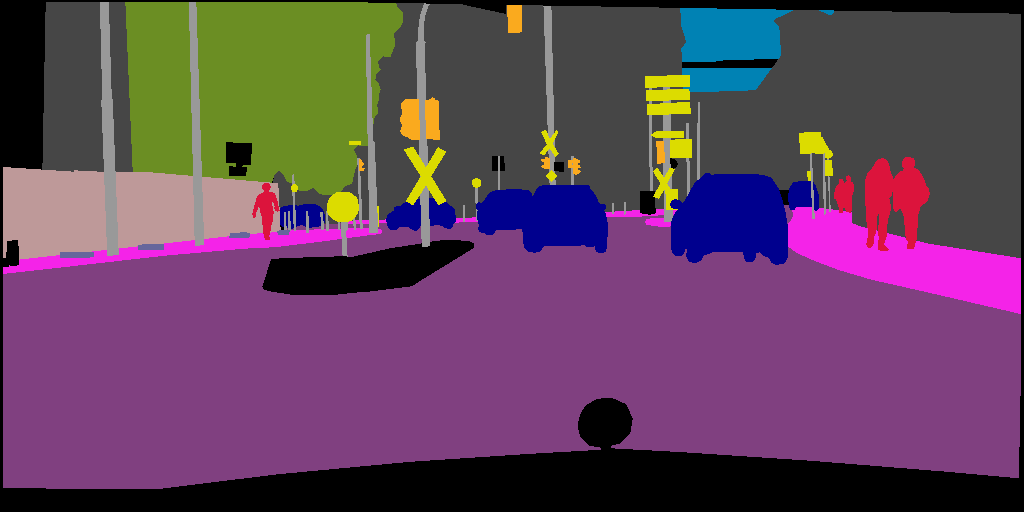} & 
   \includegraphics[width=\imgsize]{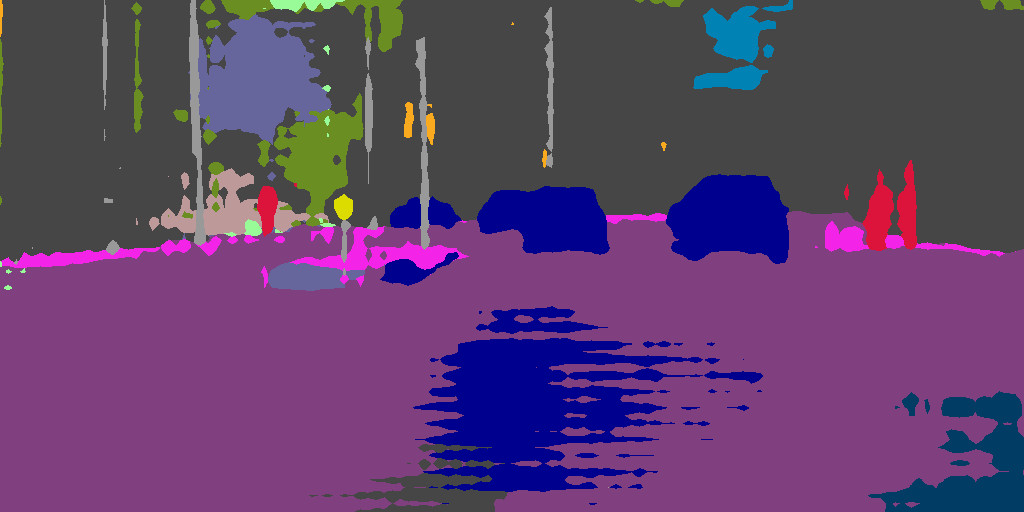} & 
   \includegraphics[width=\imgsize]{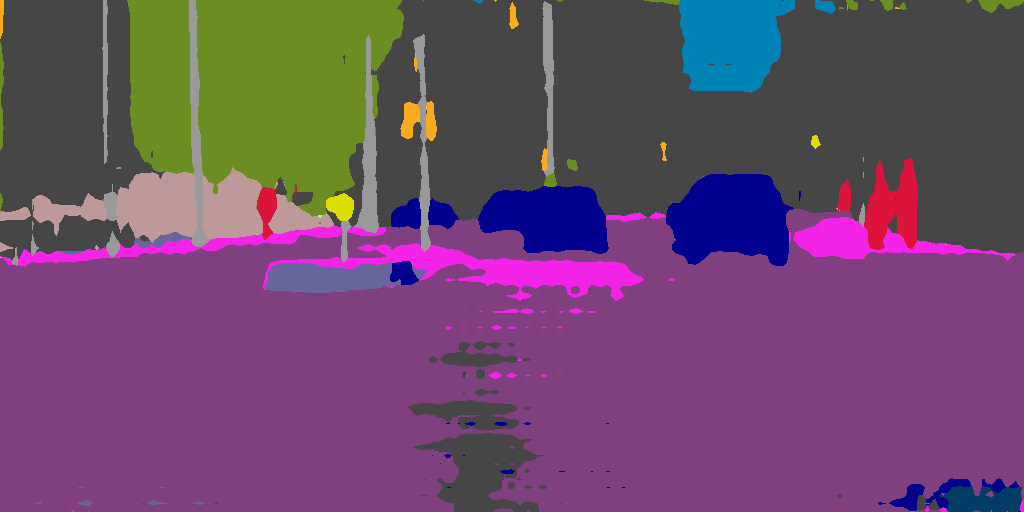} & 
   \includegraphics[width=\imgsize]{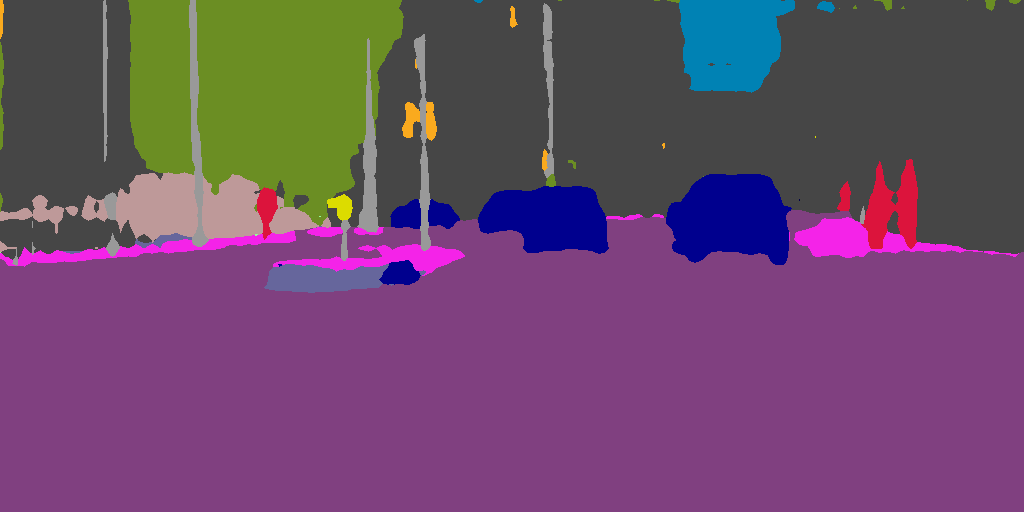} &
   \includegraphics[width=\imgsize]{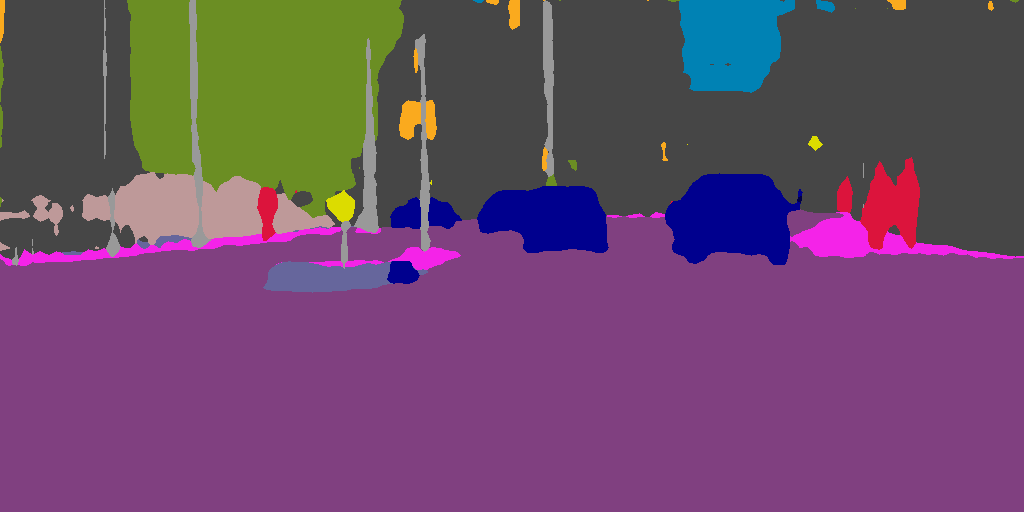} \\%[-0.1em] 
   
   \midrule 
   \rule{0pt}{41pt}
   
   \multirow{1}{*}{\rotatebox{90}{SYNTHIA $\rightarrow$ Cityscapes}} &
   \includegraphics[width=\imgsize]{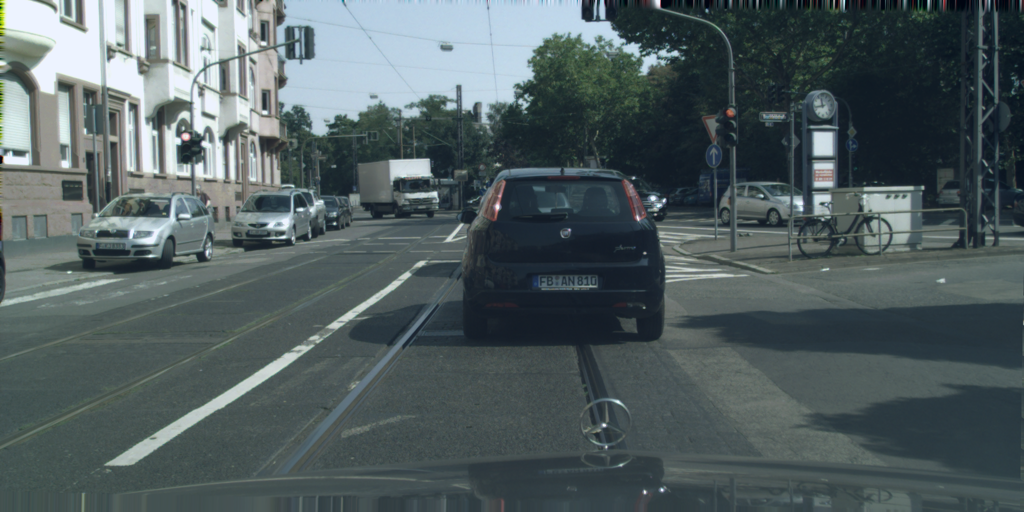} &
   \includegraphics[width=\imgsize]{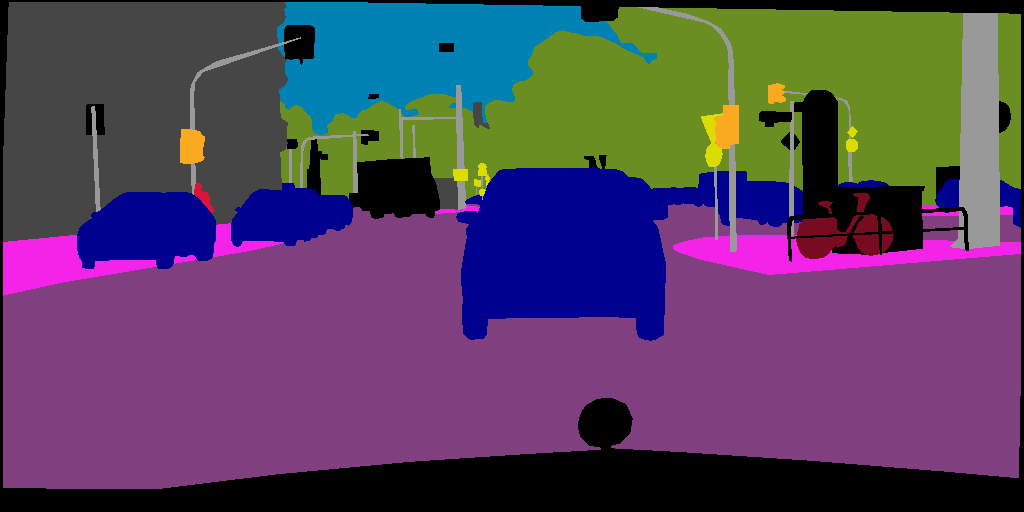} & 
   \includegraphics[width=\imgsize]{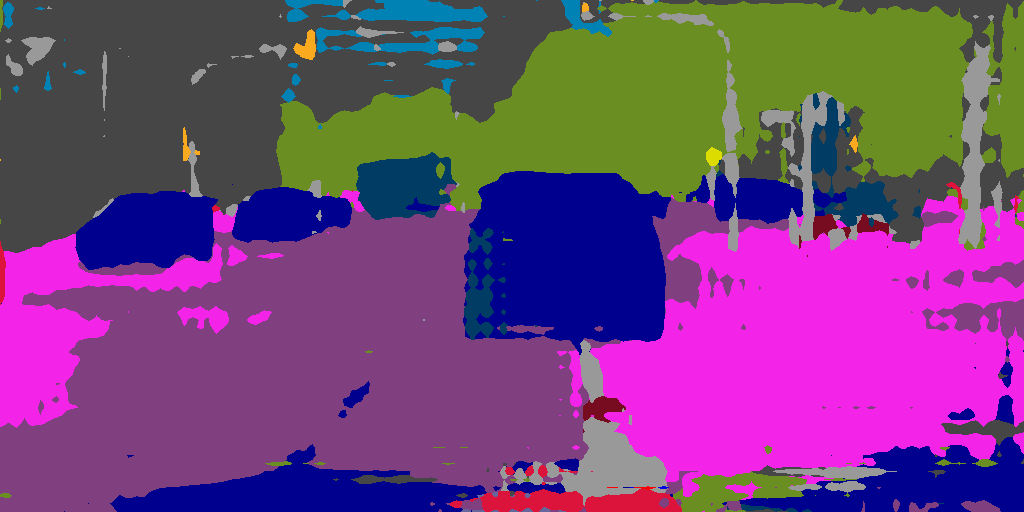} & 
   \includegraphics[width=\imgsize]{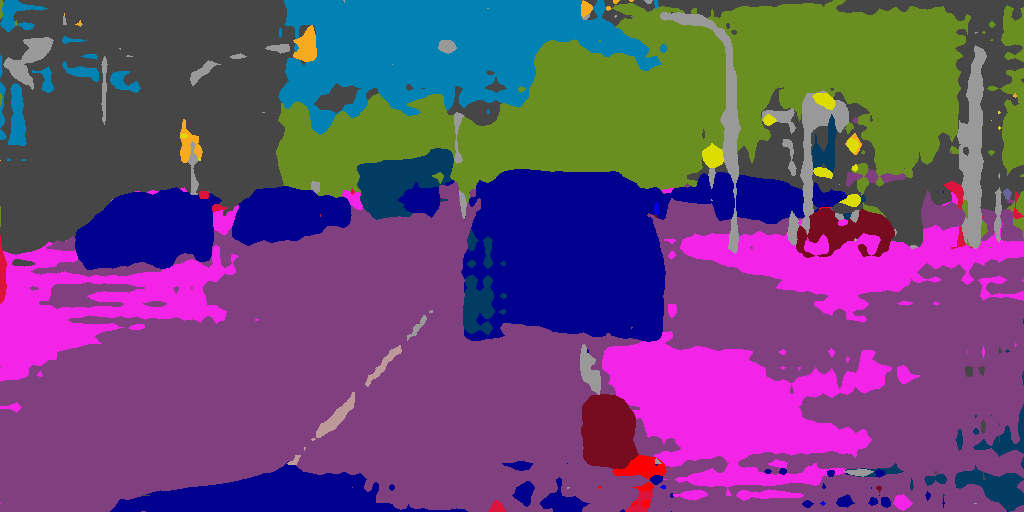} & 
   \includegraphics[width=\imgsize]{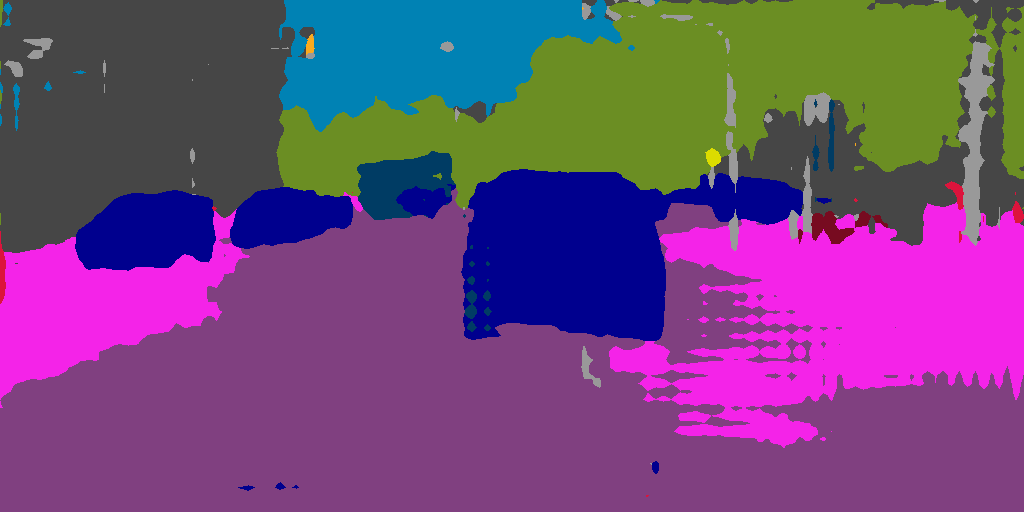} &
   \includegraphics[width=\imgsize]{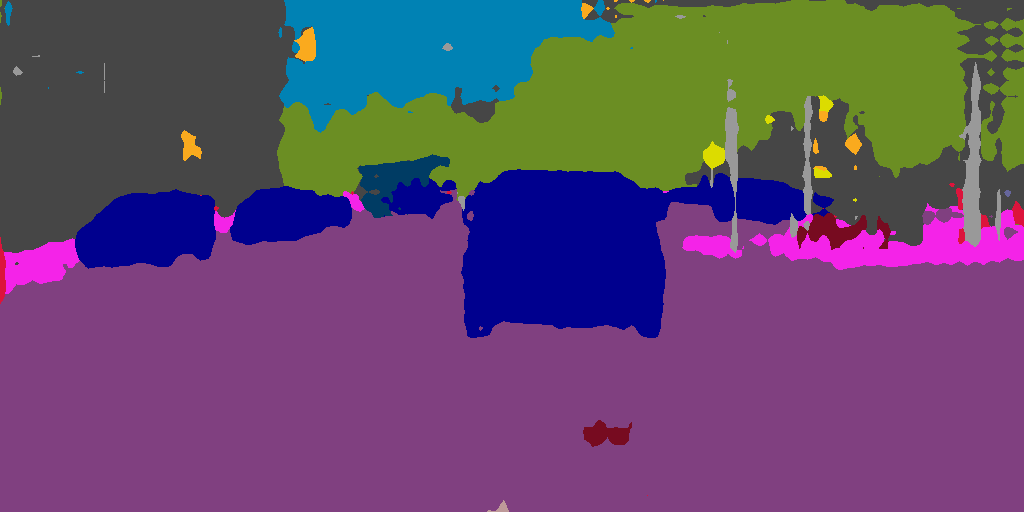} \\ 
   
   &
   \includegraphics[width=\imgsize]{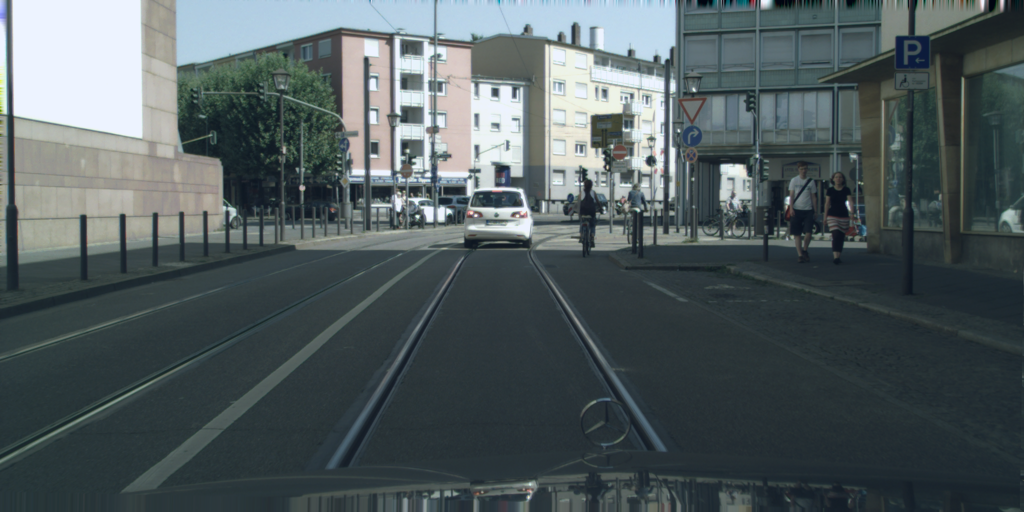} &
   \includegraphics[width=\imgsize]{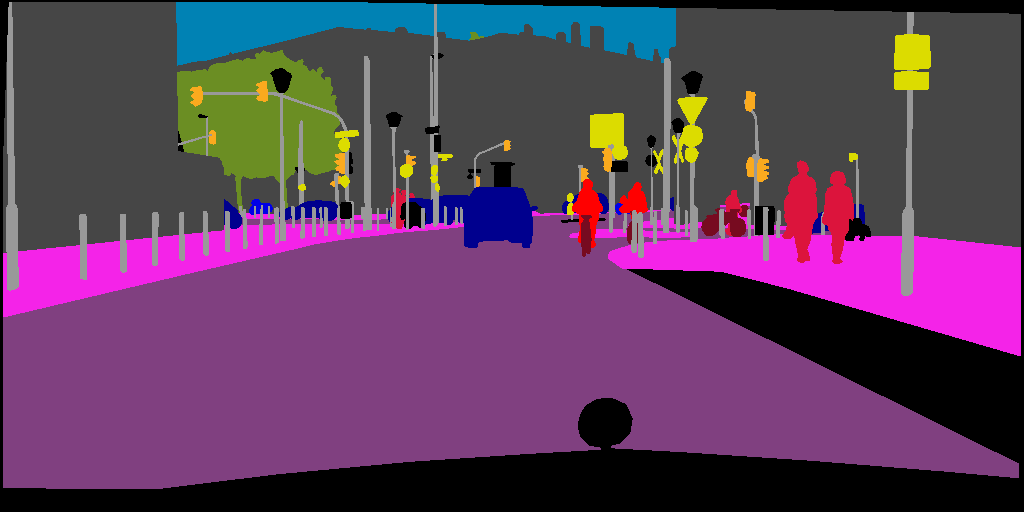} & 
   \includegraphics[width=\imgsize]{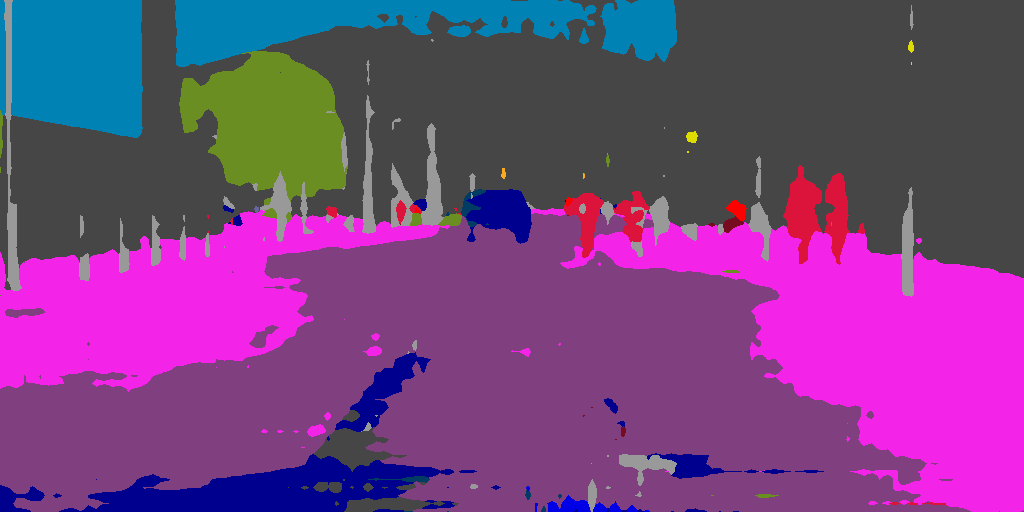} & 
   \includegraphics[width=\imgsize]{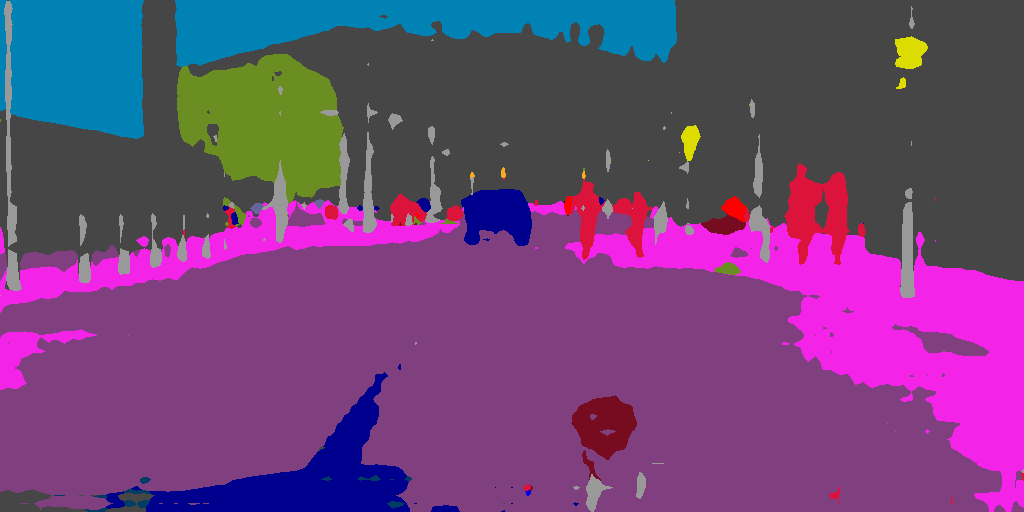} & 
   \includegraphics[width=\imgsize]{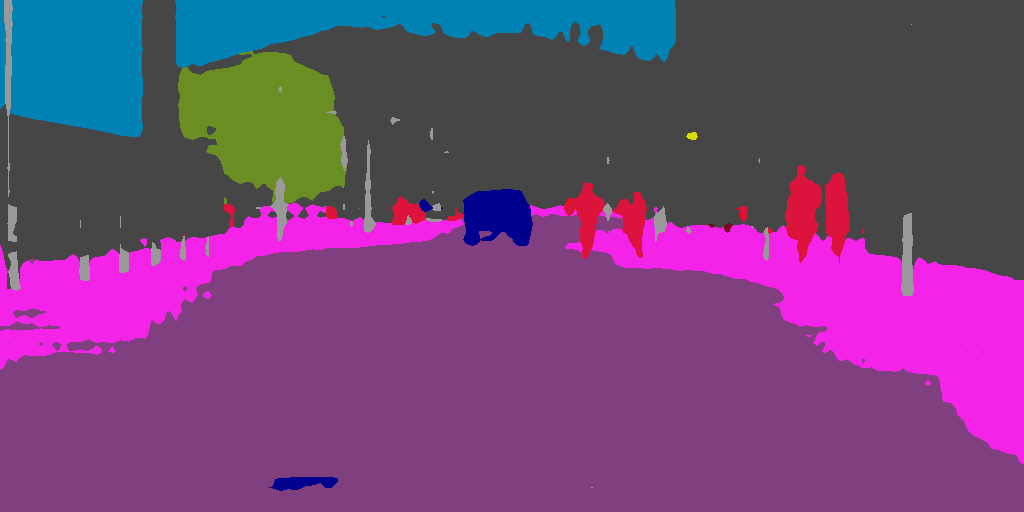} &
   \includegraphics[width=\imgsize]{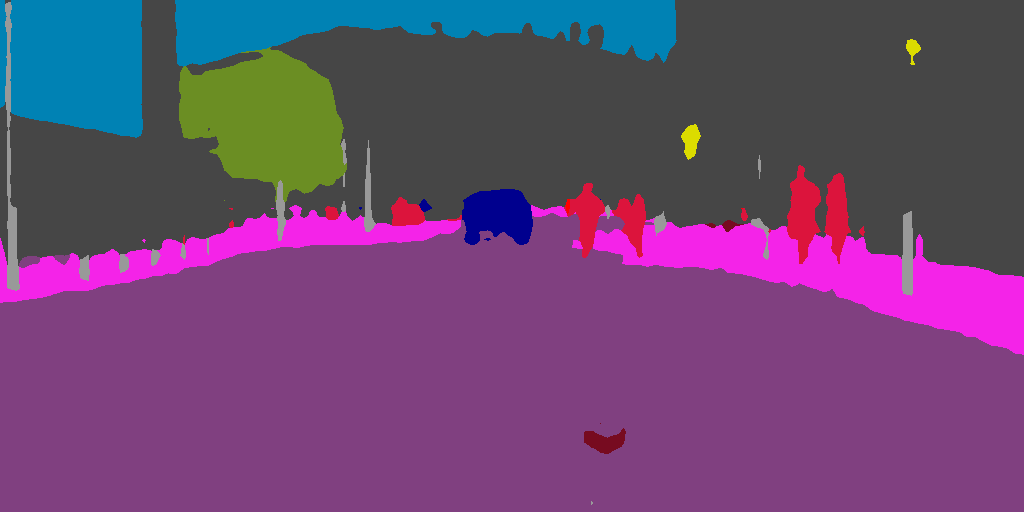} \\    
   
   &
   \includegraphics[width=\imgsize]{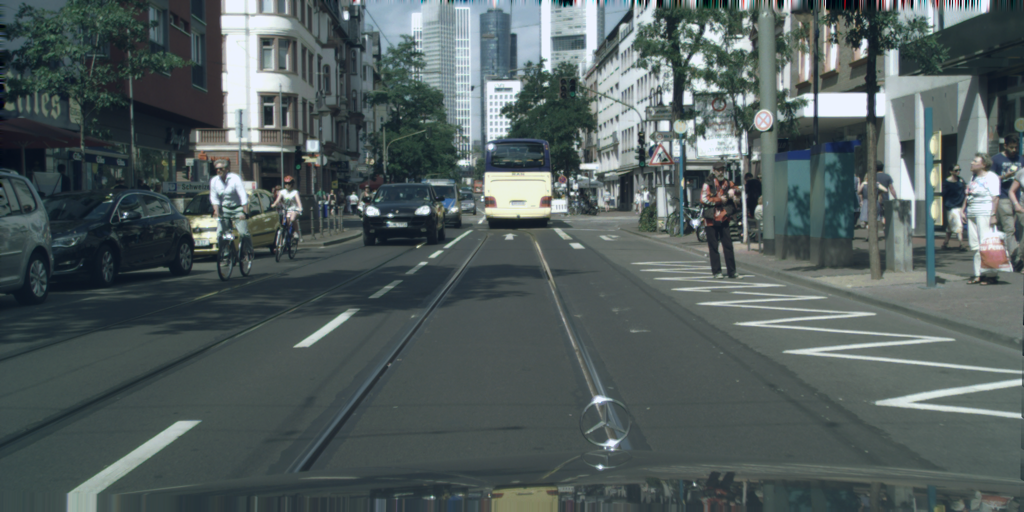} &
   \includegraphics[width=\imgsize]{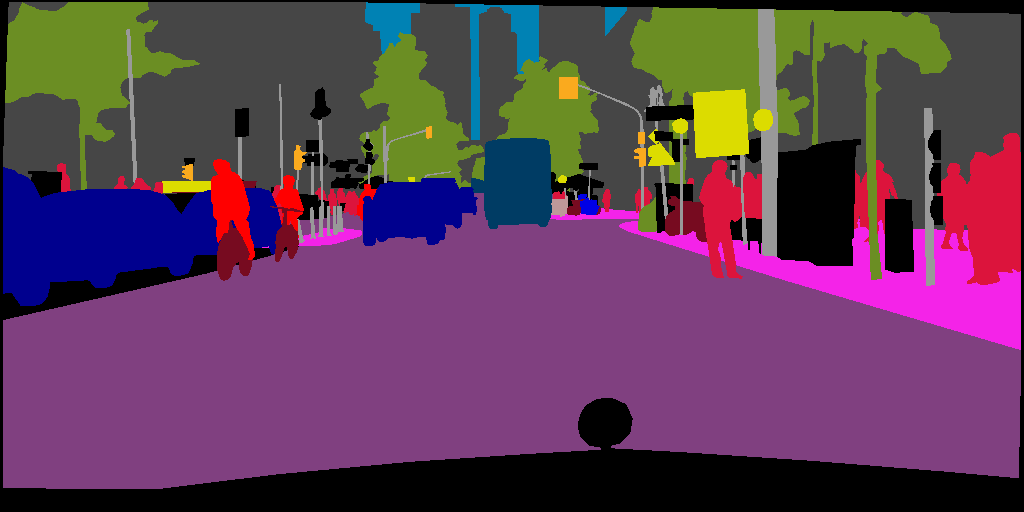} & 
   \includegraphics[width=\imgsize]{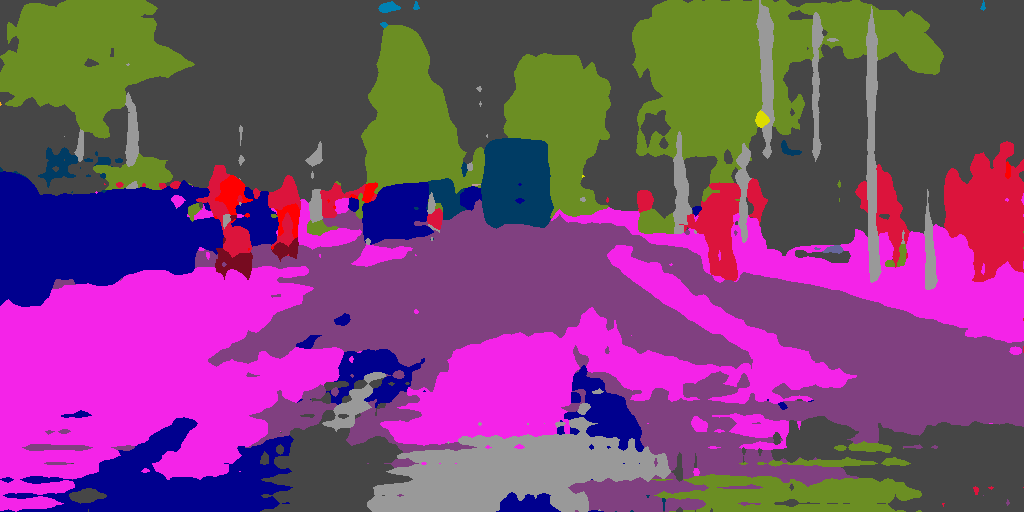} & 
   \includegraphics[width=\imgsize]{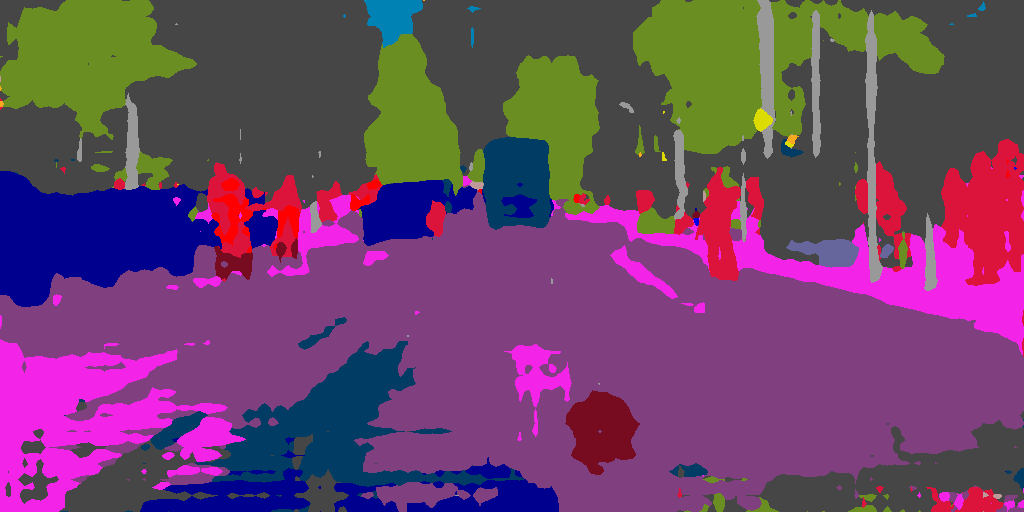} & 
   \includegraphics[width=\imgsize]{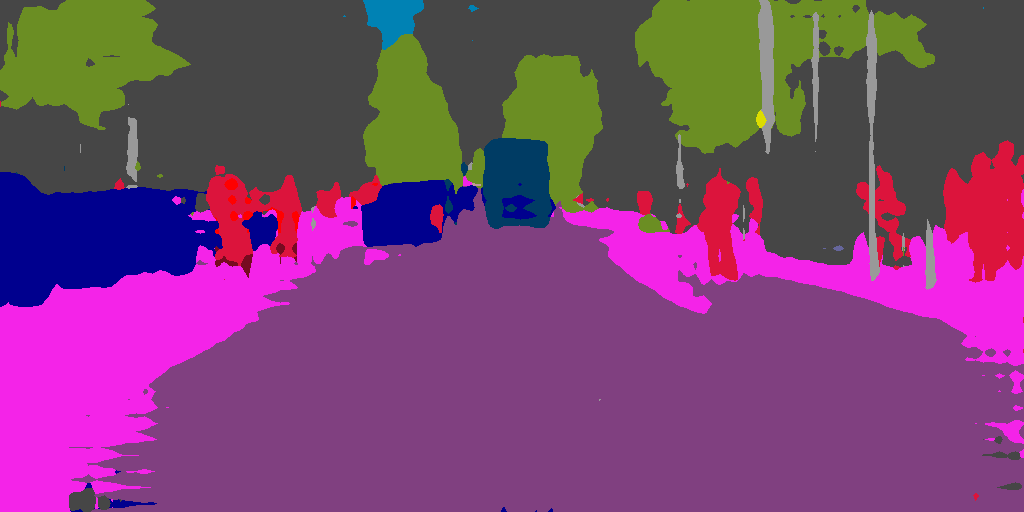} &
   \includegraphics[width=\imgsize]{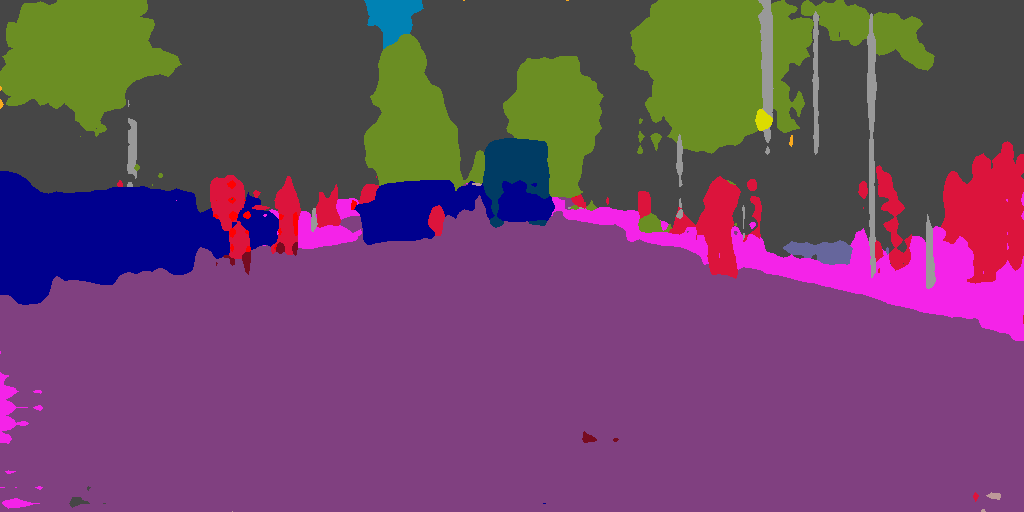} \\
   
   &
   \includegraphics[width=\imgsize]{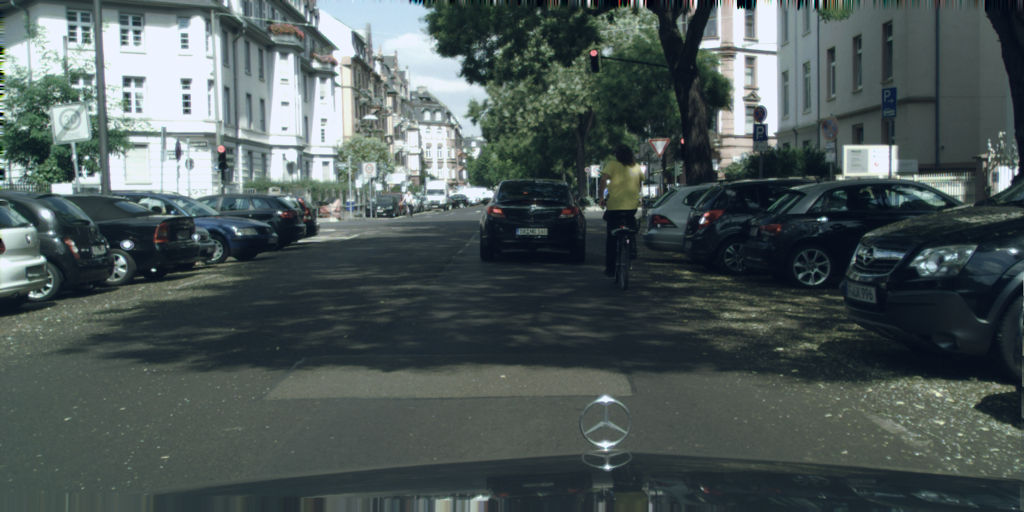} &
   \includegraphics[width=\imgsize]{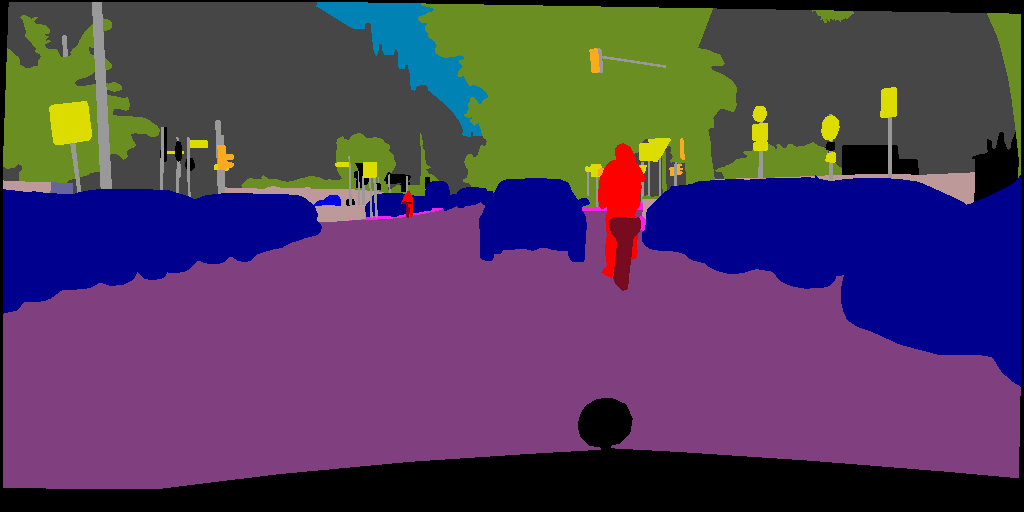} & 
   \includegraphics[width=\imgsize]{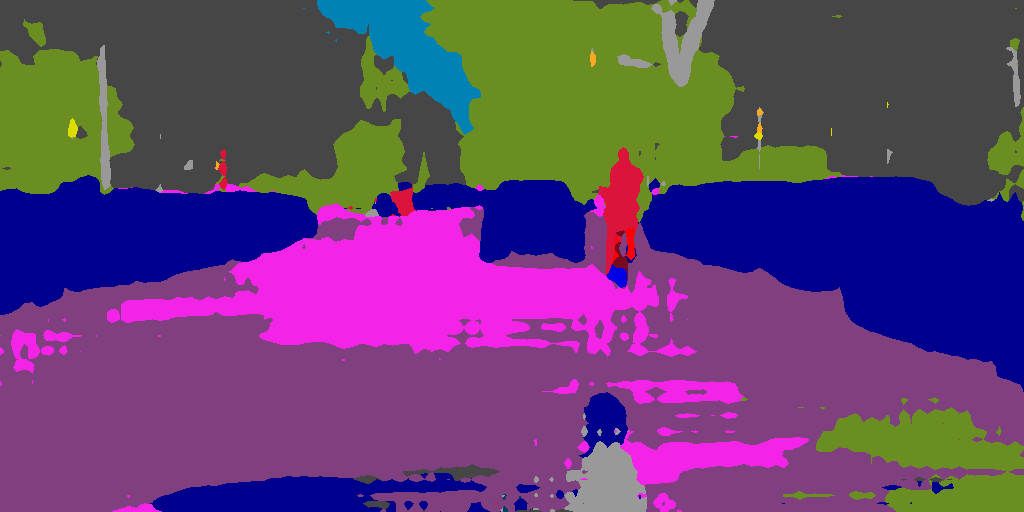} & 
   \includegraphics[width=\imgsize]{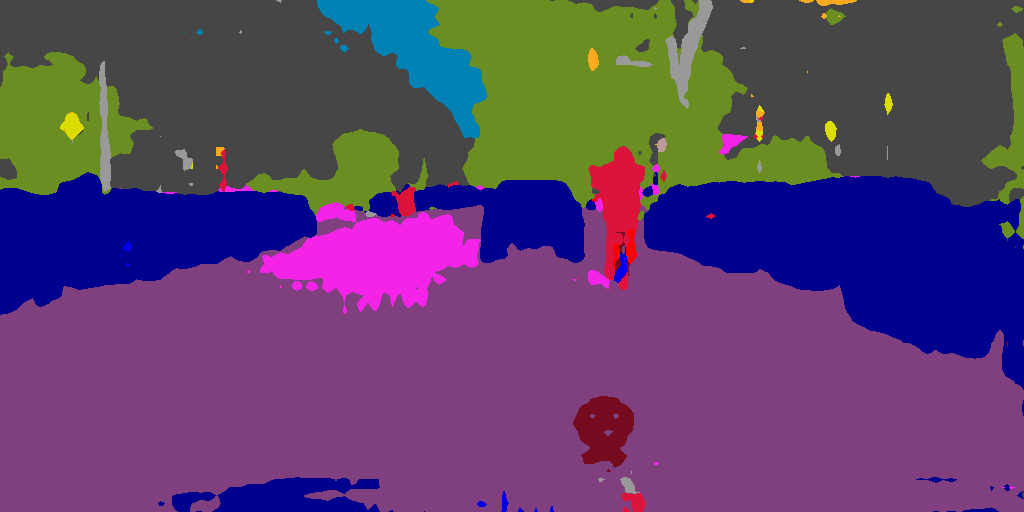} & 
   \includegraphics[width=\imgsize]{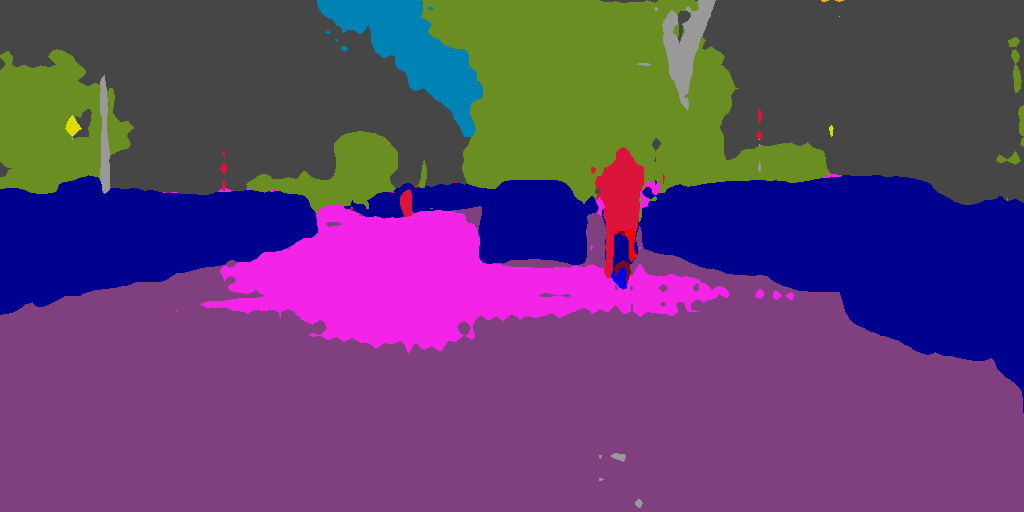} &
   \includegraphics[width=\imgsize]{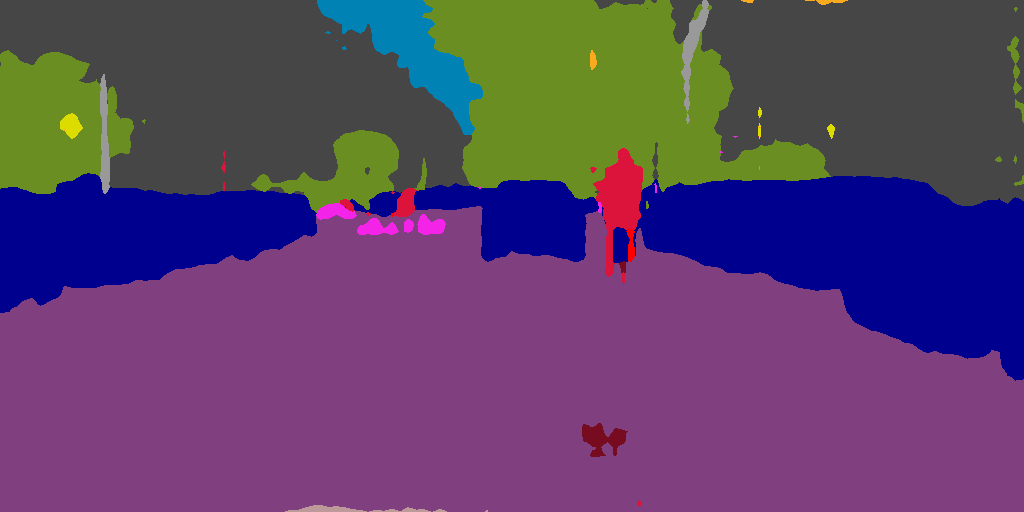} \\
   
  \multicolumn{1}{c}{} & \multicolumn{1}{c}{Target Images} & Ground Truth & Source Only  & Ours ($\mathcal{L}_{cl}$) & MaxSquare IW \cite{Chen2019} & Ours ($\mathcal{L}_{tot}$)

\end{tabular}
\end{subfigure}

\caption{Semantic segmentation of some sample scenes extracted from the Cityscapes validation target dataset when adaptation is performed from the GTA5 (top) and SYNTHIA (bottom) source datasets and the DeepLab-V2 with ResNet-101 backbone is employed as segmentation network (\textit{best viewed in colors}).}
\label{fig:qual_res}
\end{figure*}
